# Supplementary material for: Facilitating Parallel Fuzzing with mutually-exclusive Task Distribution
Source: arXiv:2109.08635 source file (2021-09-17)
Supplement: Supplementary file 1 [file appendices.tex]

\appendix

\clearpage
% \begin{table*}[t!]

\centering
% \begin{adjustwidth}{-0.15cm}{}
 \begin{longtable}{wc{4.5cm}wc{4.5cm}wc{4.5cm}}
         \includegraphics[scale=0.075]{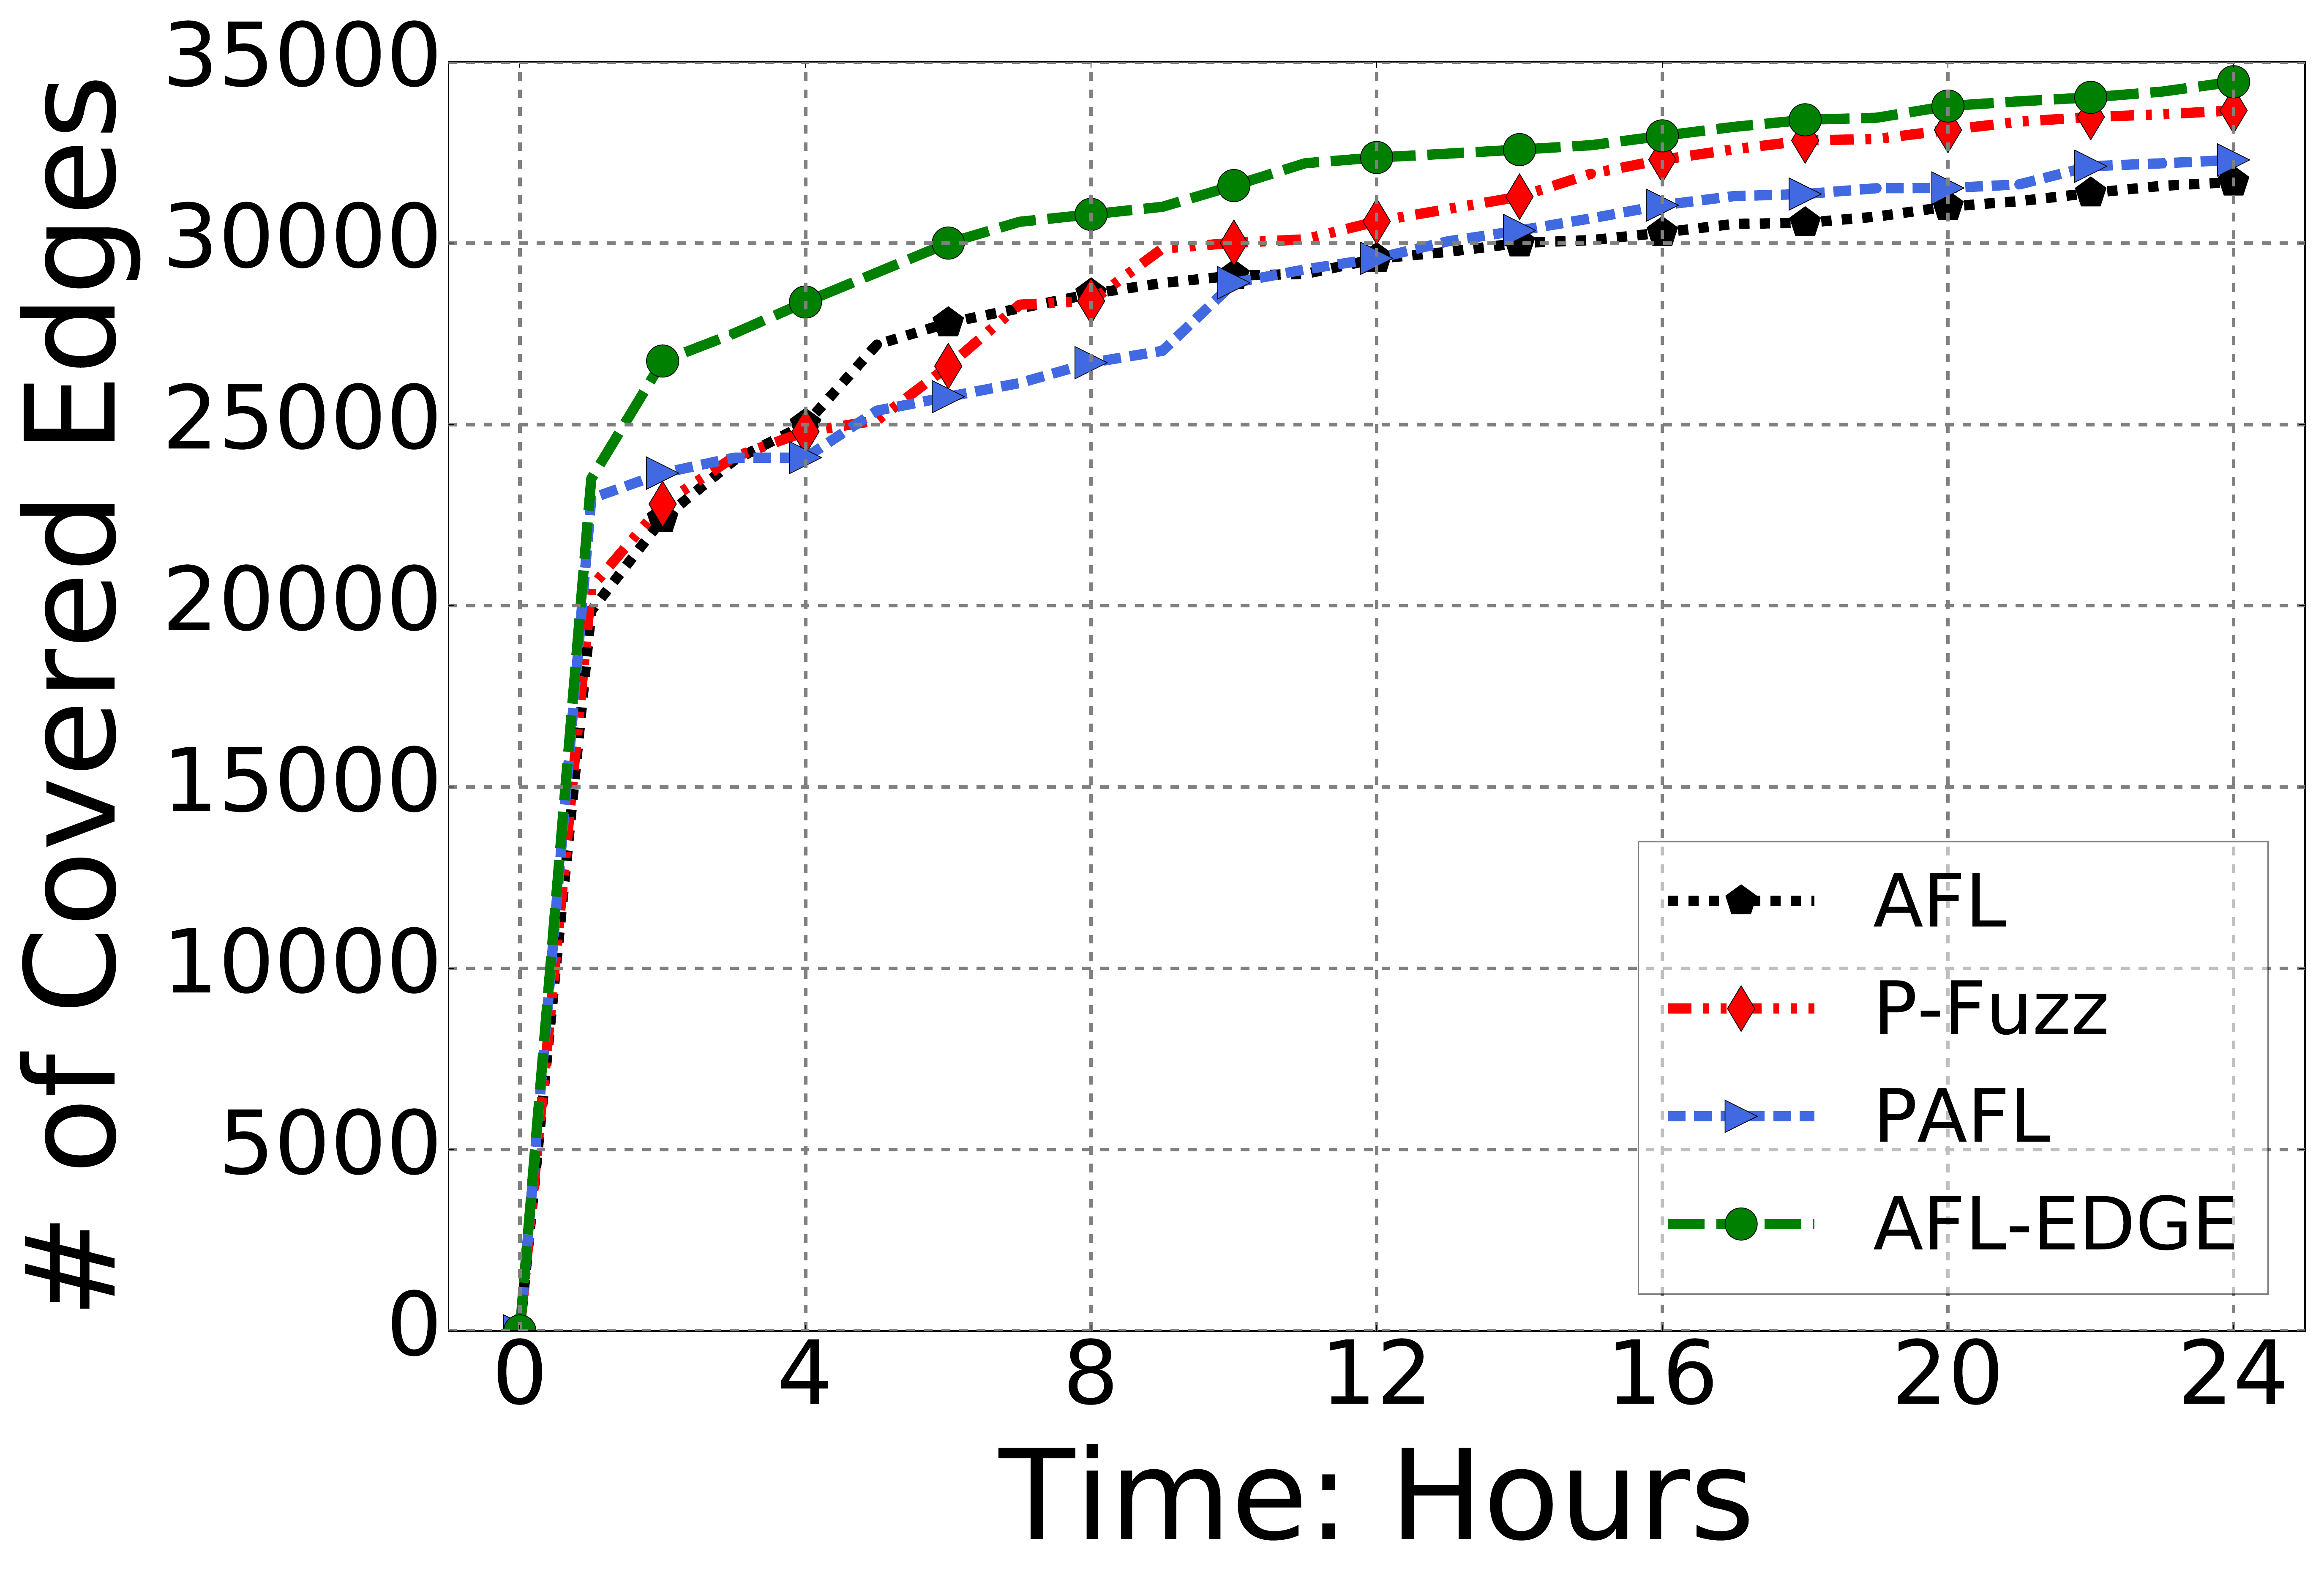} & 
         \includegraphics[scale=0.075]{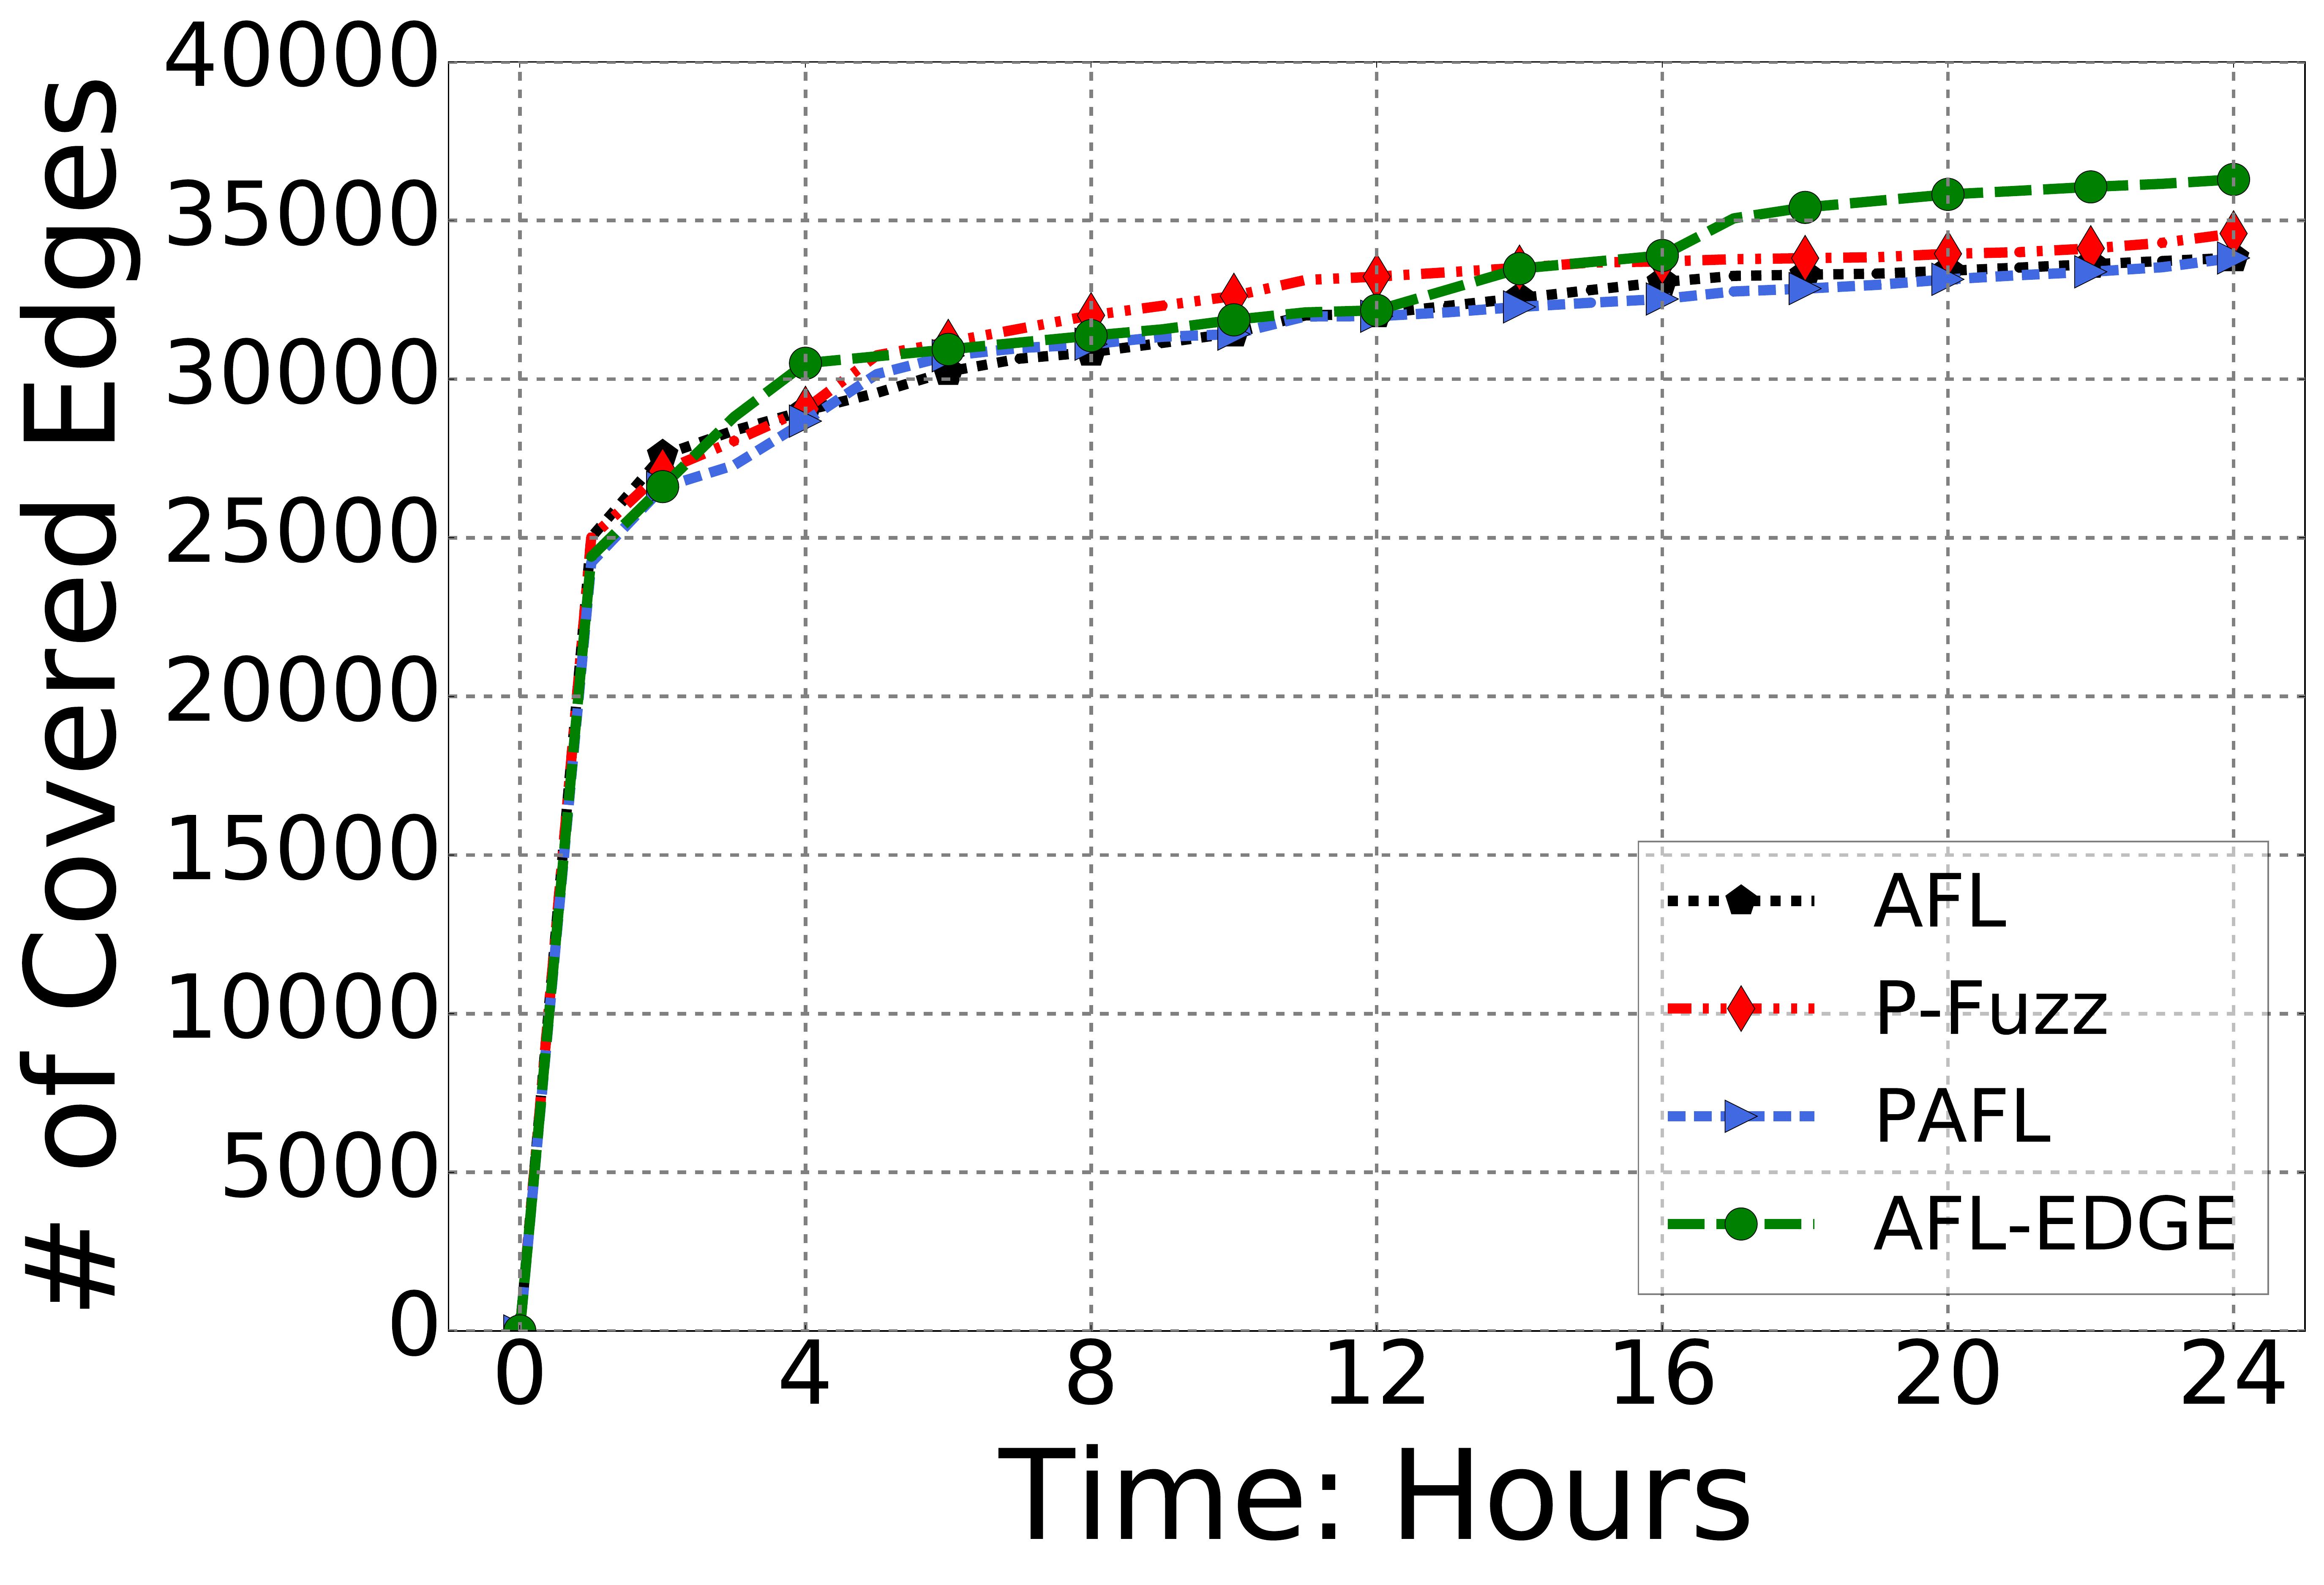} &
         \includegraphics[scale=0.075]{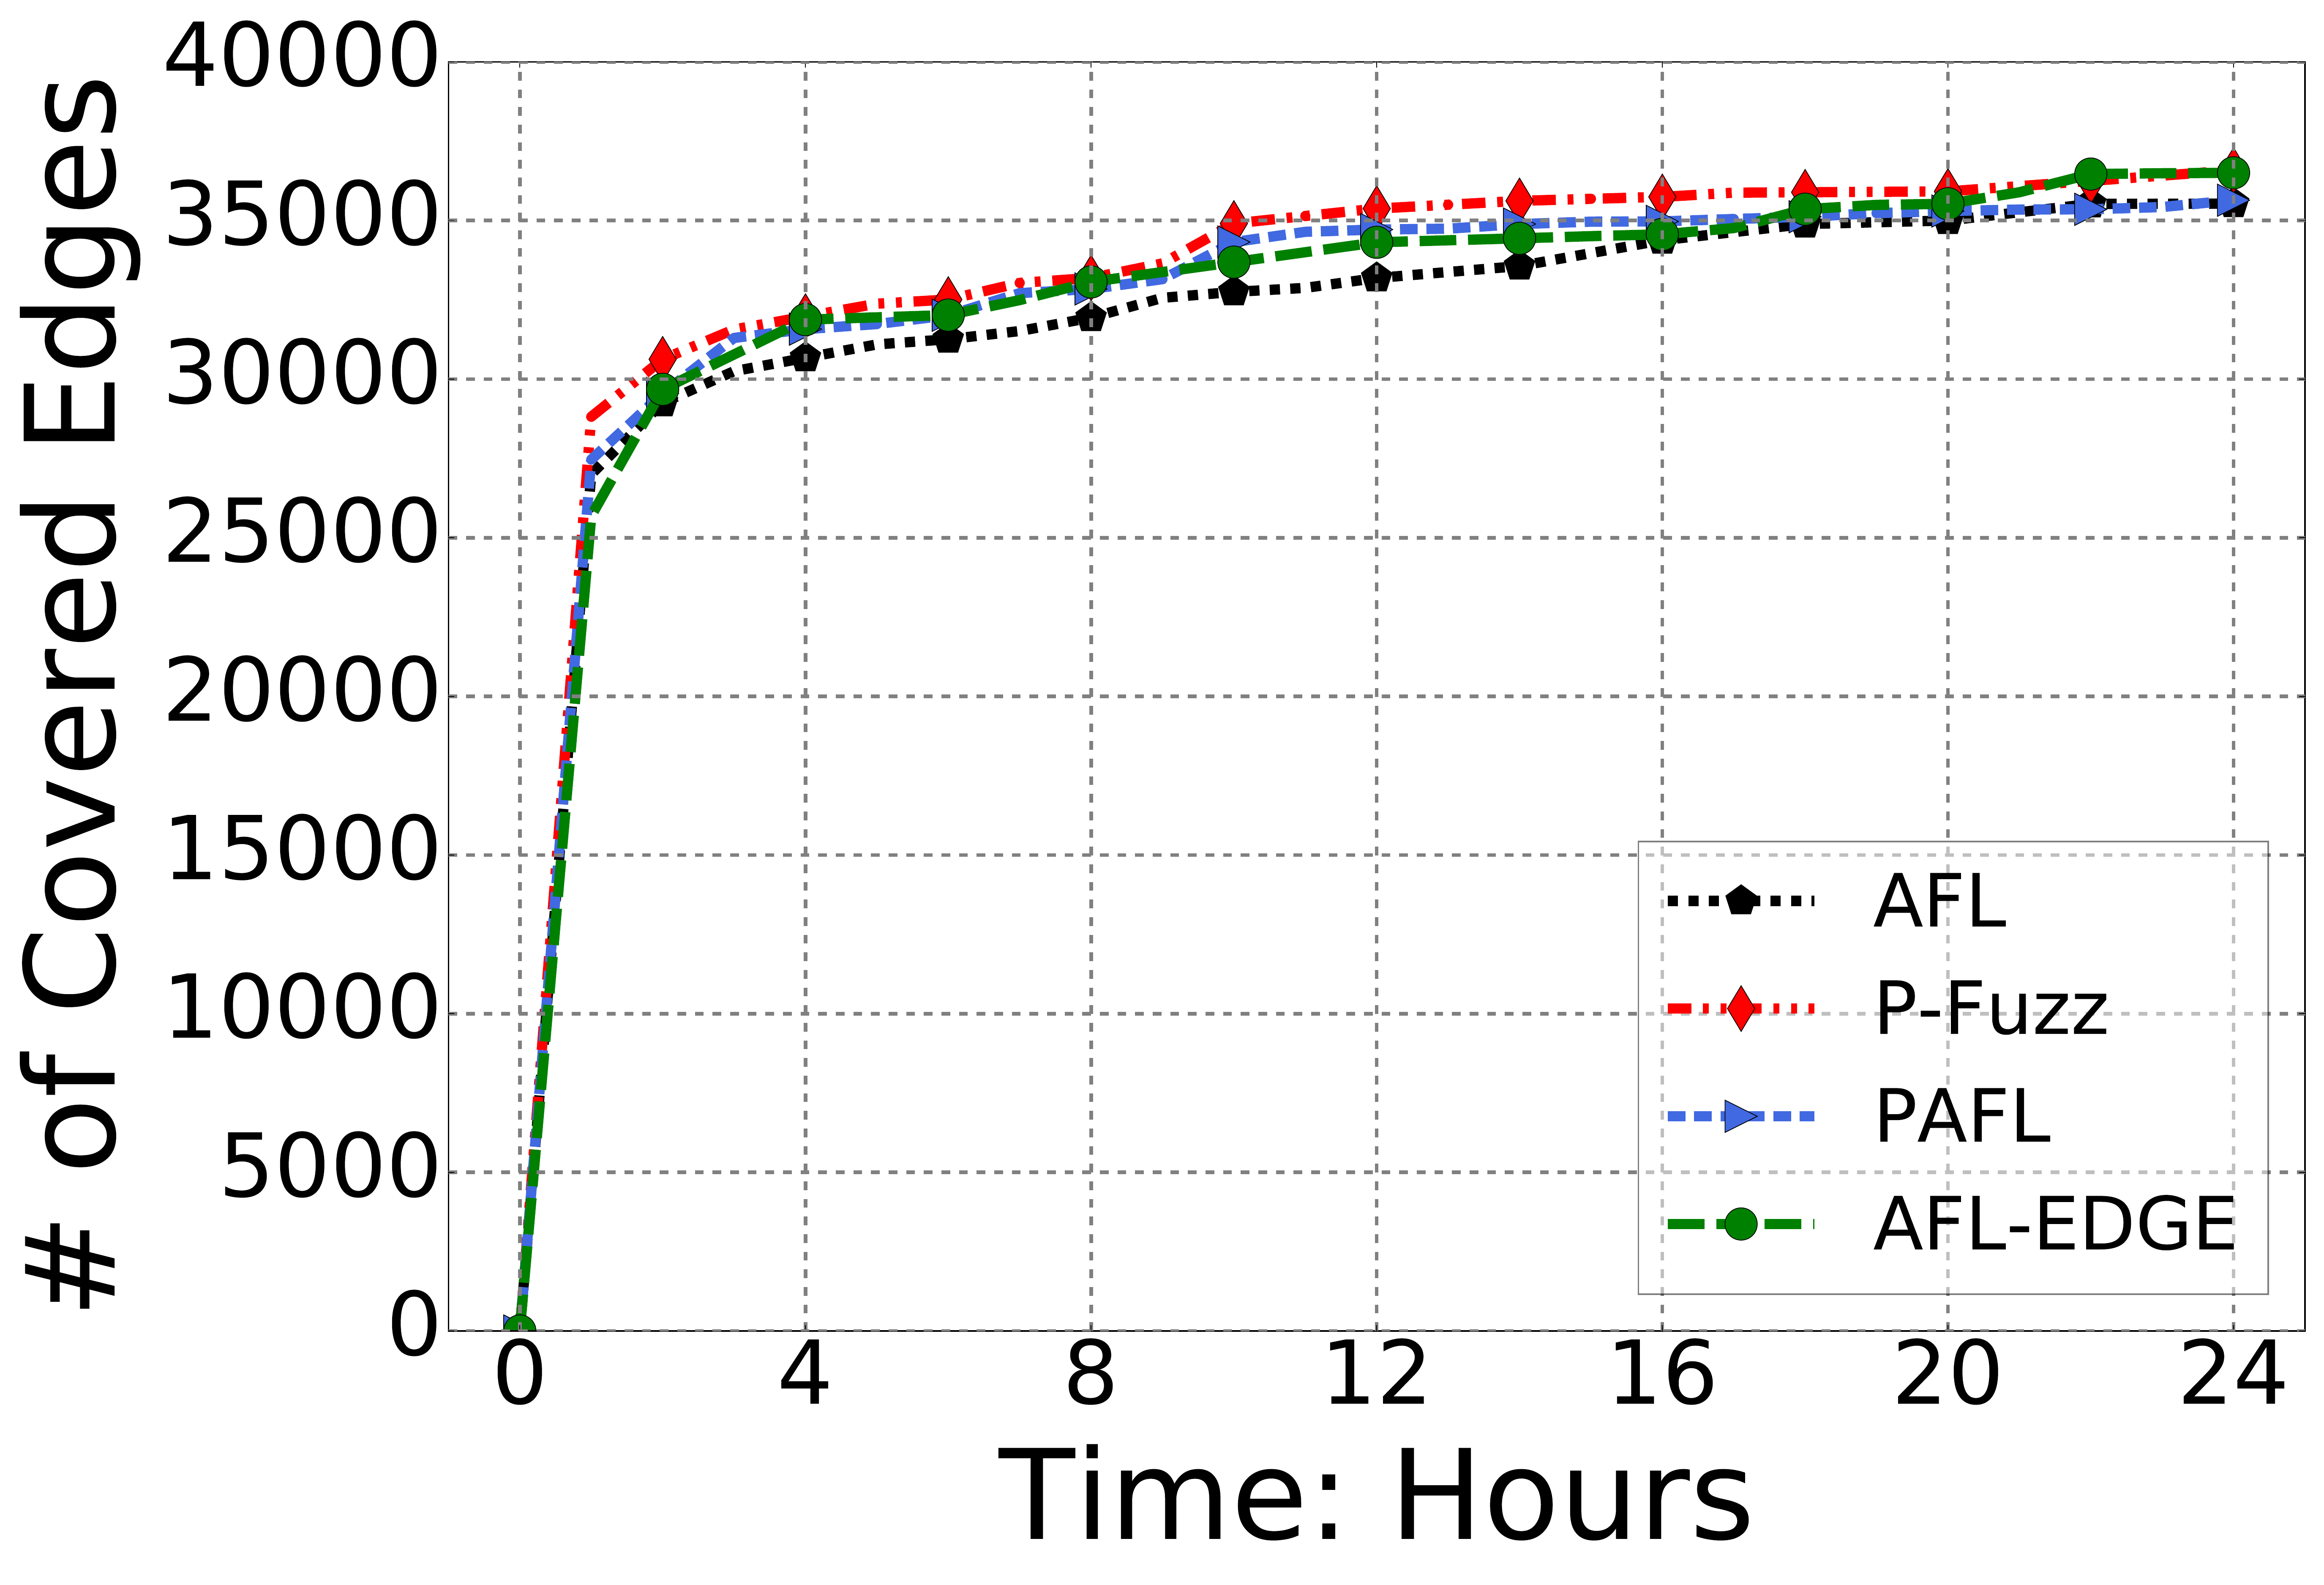} 
         \\
         {\scriptsize\textbf{objdump} \scriptsize 2 instances AFL} &
         {\scriptsize\textbf{objdump} \scriptsize 4 instances AFL} &
         {\scriptsize\textbf{objdump} \scriptsize 8 instances AFL} 
        %  {\scriptsize\textbf{objdump} \scriptsize 2 instance QSYM} &
        %  {\scriptsize\textbf{objdump} \scriptsize 4 instance QSYM} &
        %  {\scriptsize\textbf{objdump} \scriptsize 8 instance QSYM} \\
         \\
         
         \includegraphics[scale=0.075]{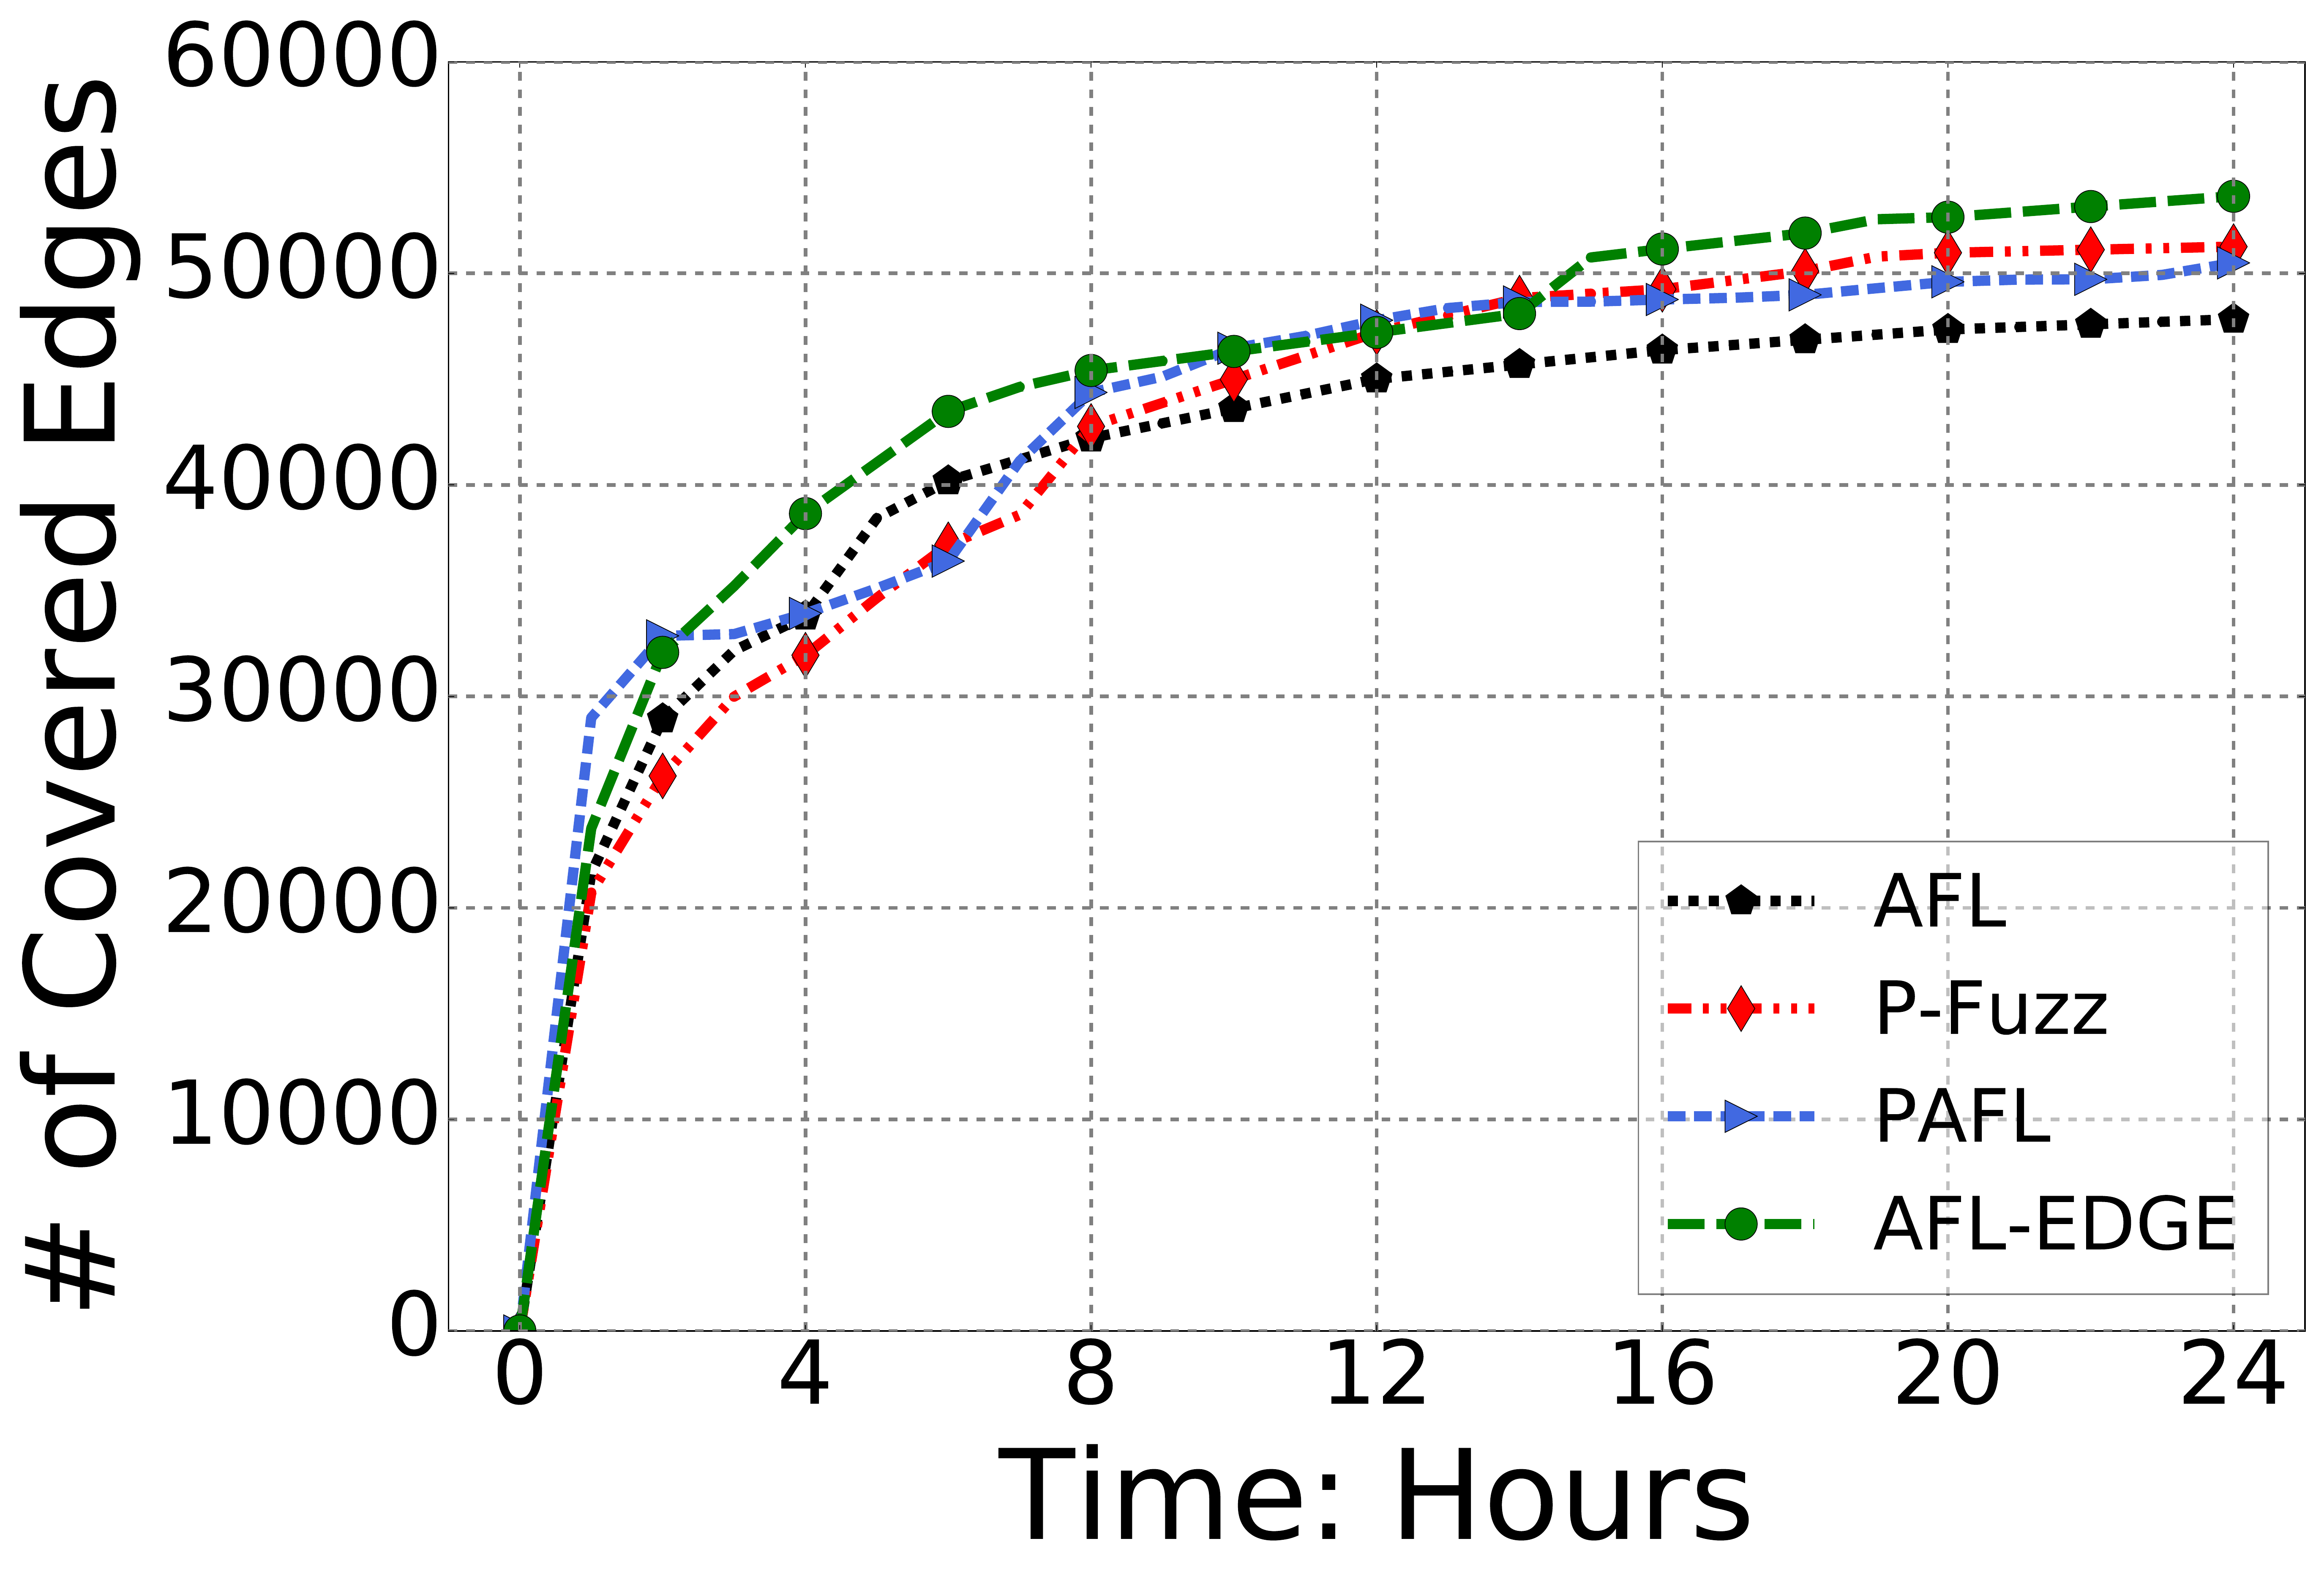} & 
         \includegraphics[scale=0.075]{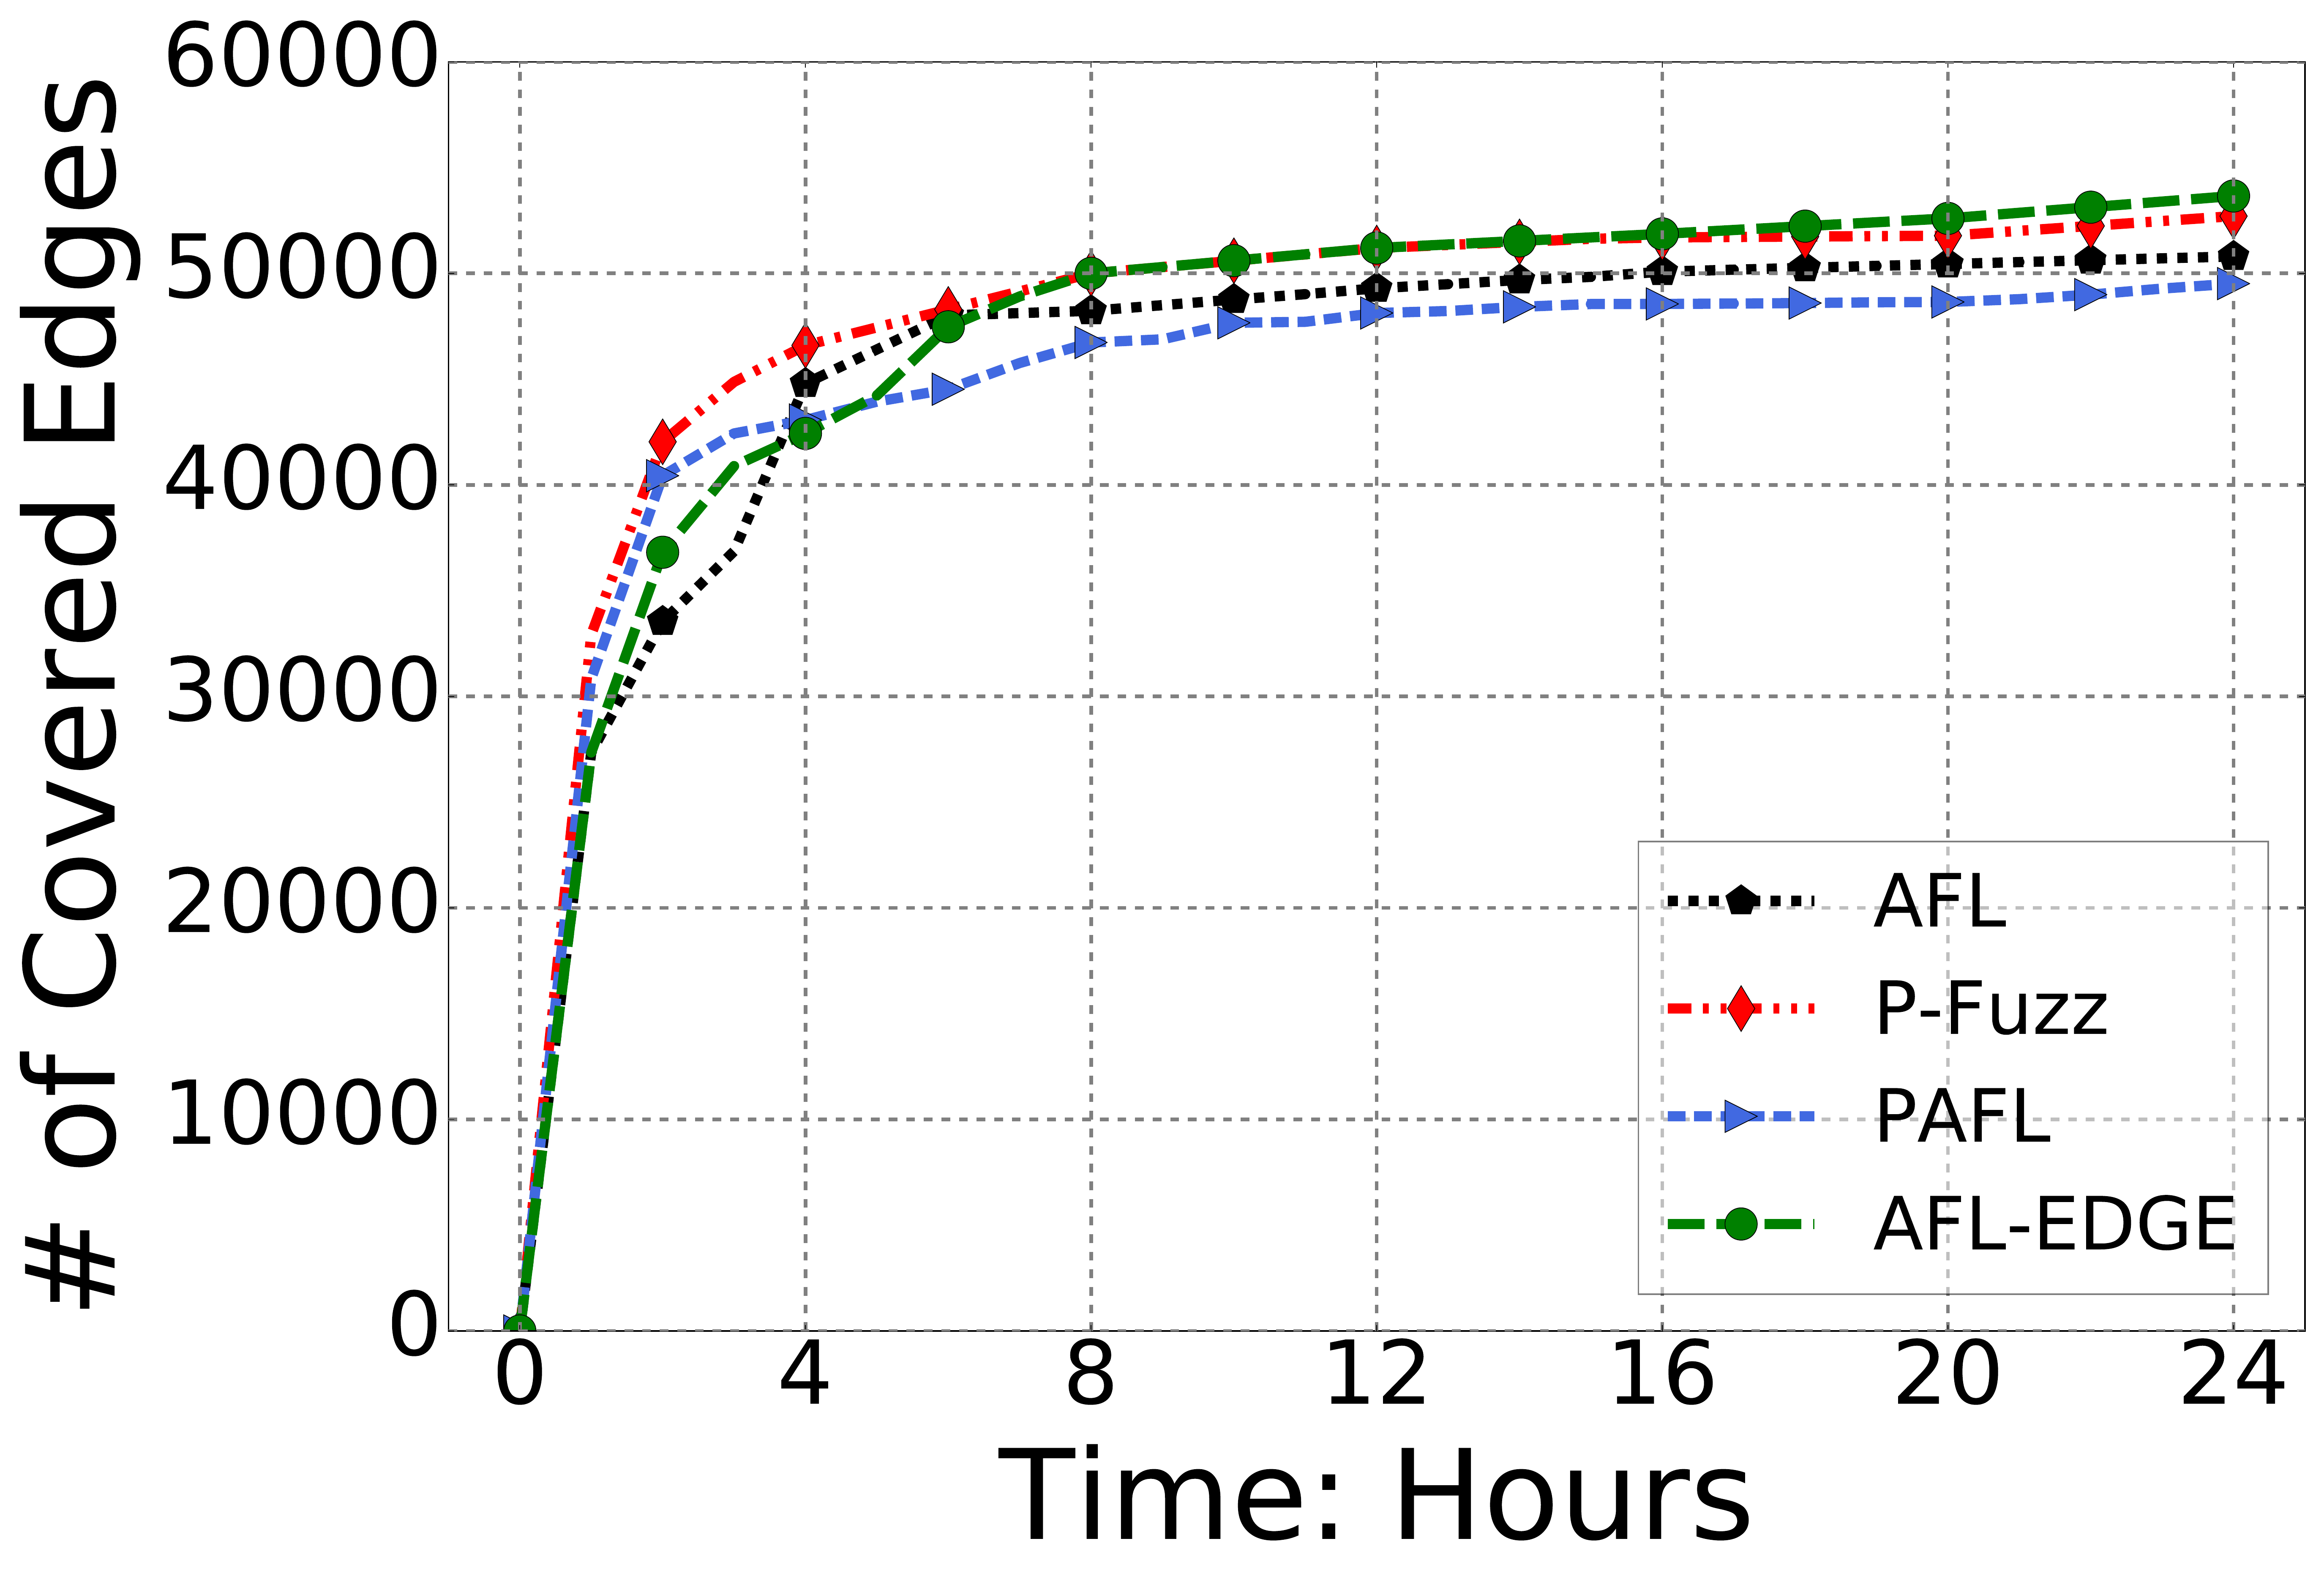} &
         \includegraphics[scale=0.075]{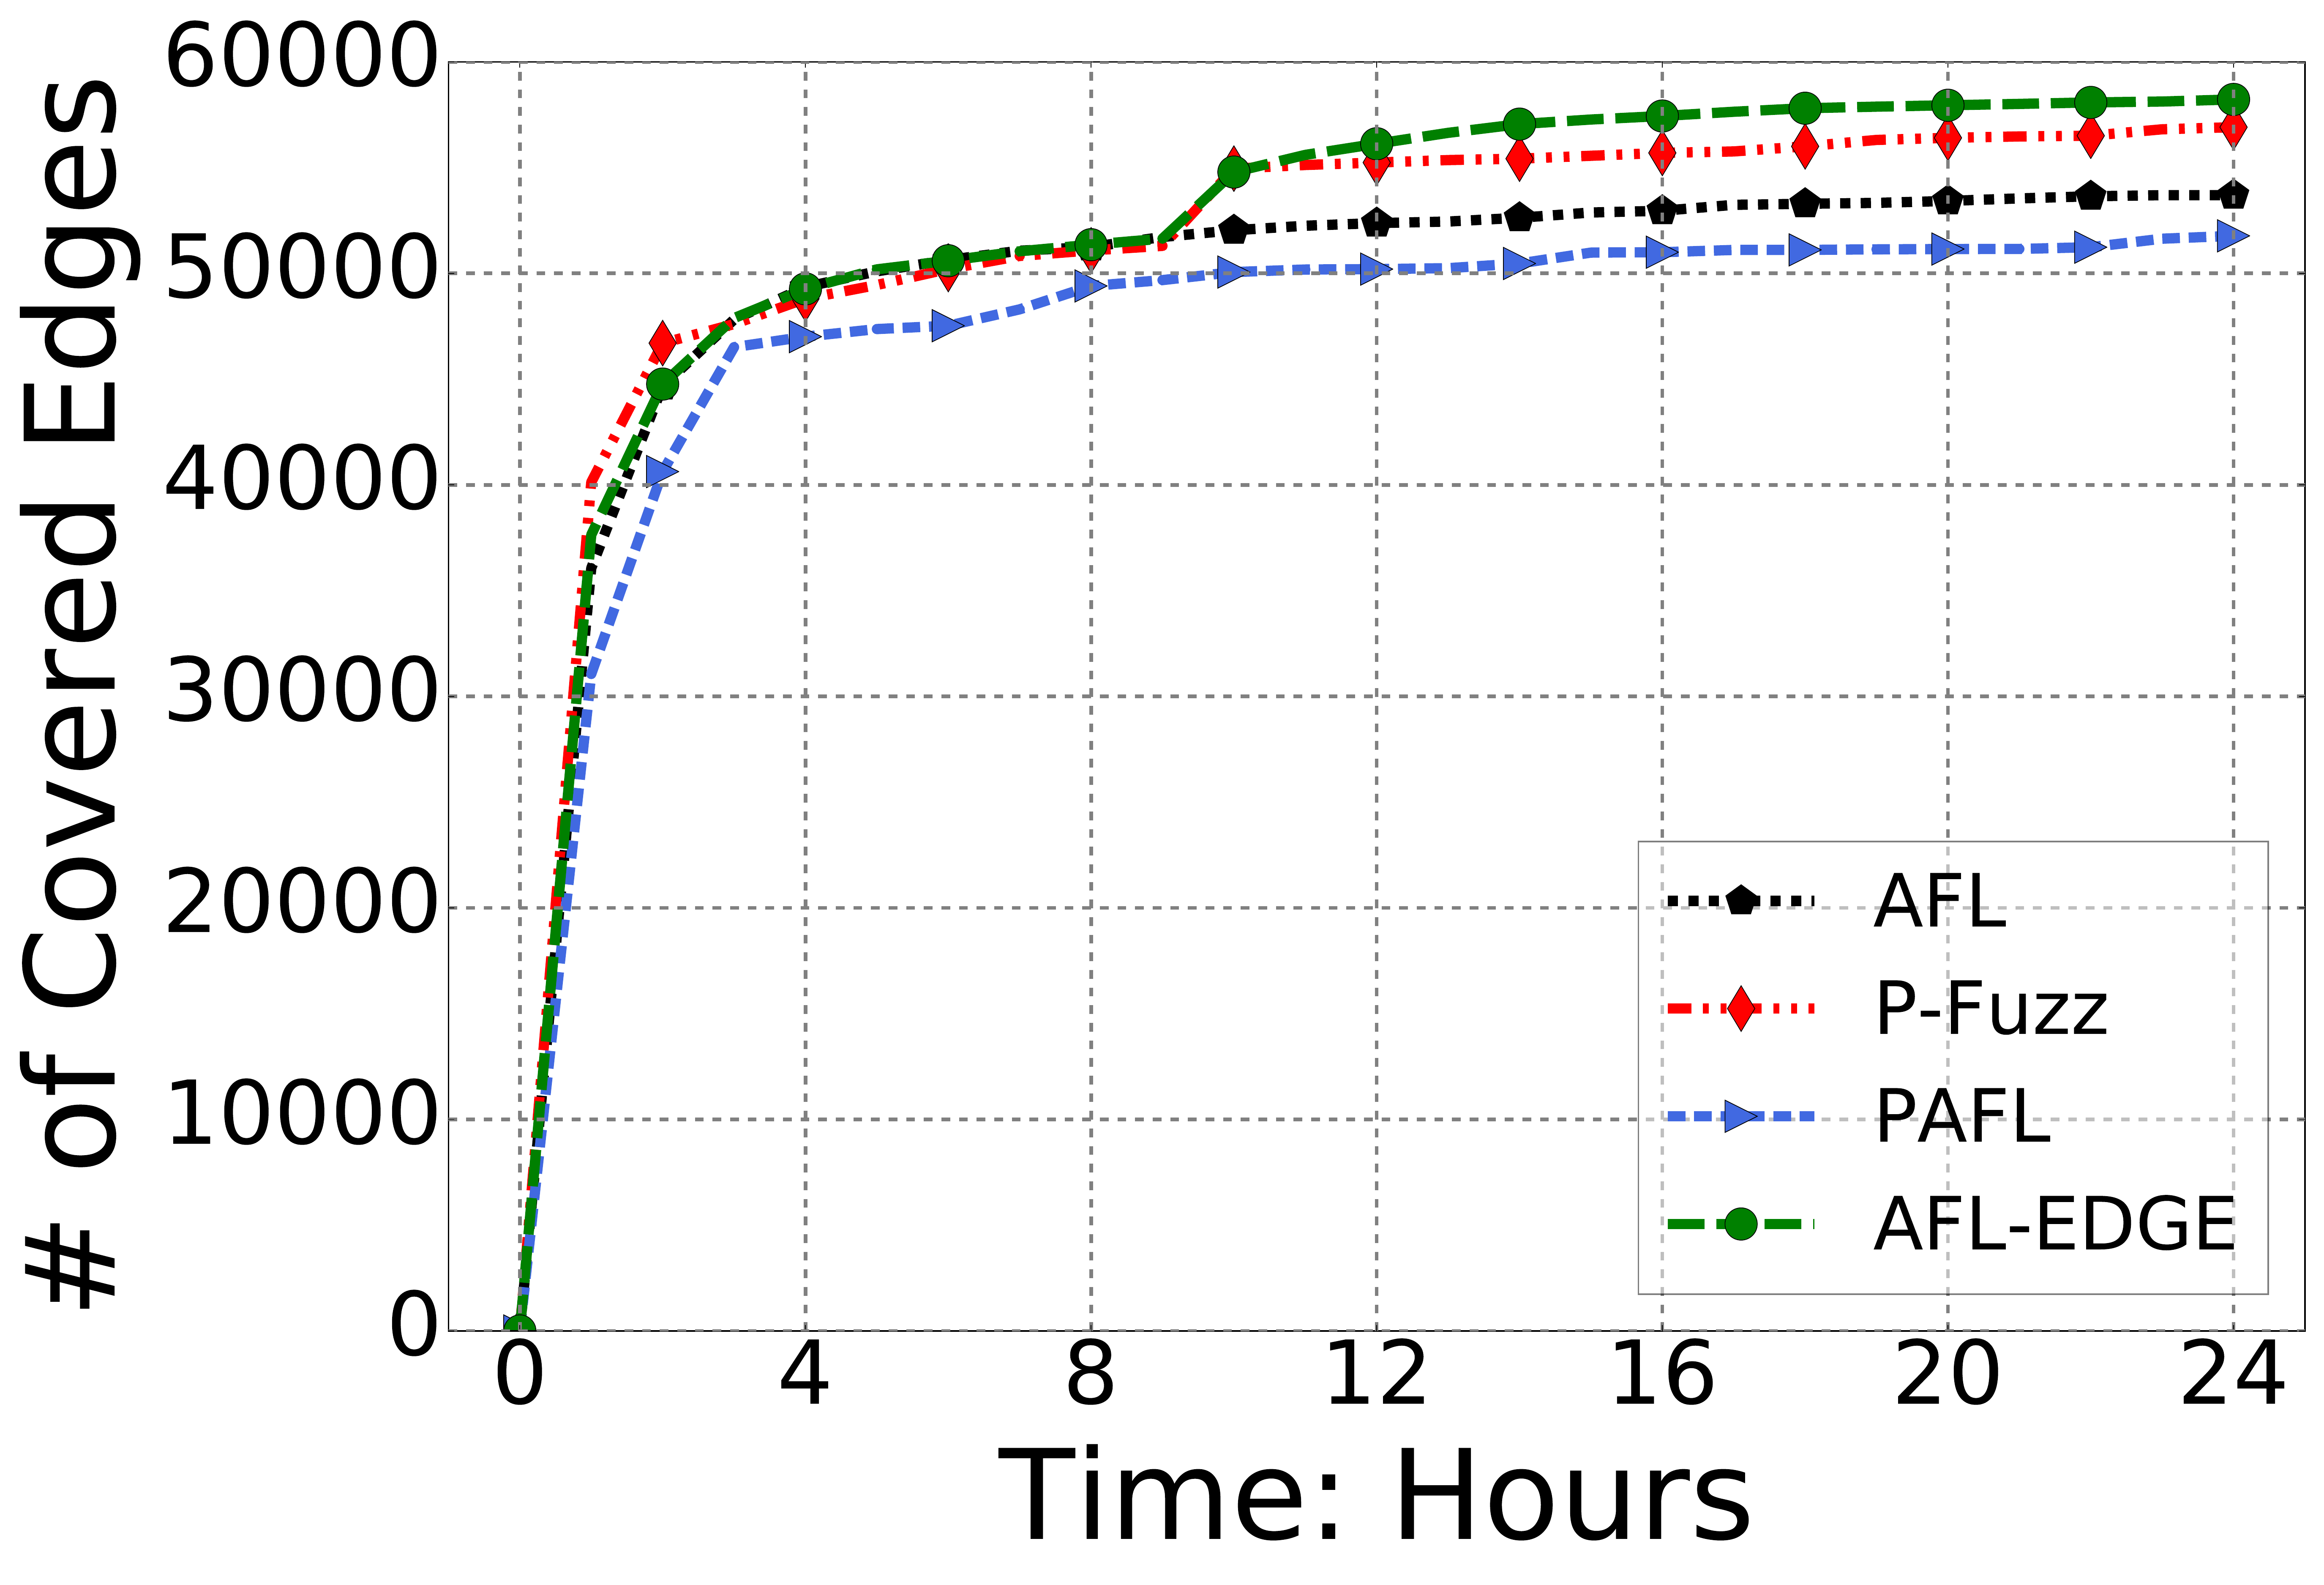} 
         \\
         {\scriptsize\textbf{readelf} \scriptsize 2 instances AFL} &
         {\scriptsize\textbf{readelf} \scriptsize 4 instances AFL} &
         {\scriptsize\textbf{readelf} \scriptsize 8 instances AFL} 
        %  {\scriptsize\textbf{readelf} \scriptsize 2 instance QSYM} &
        %  {\scriptsize\textbf{readelf} \scriptsize 4 instance QSYM} &
        %  {\scriptsize\textbf{readelf} \scriptsize 8 instance QSYM} \\
         \\
         \includegraphics[scale=0.075]{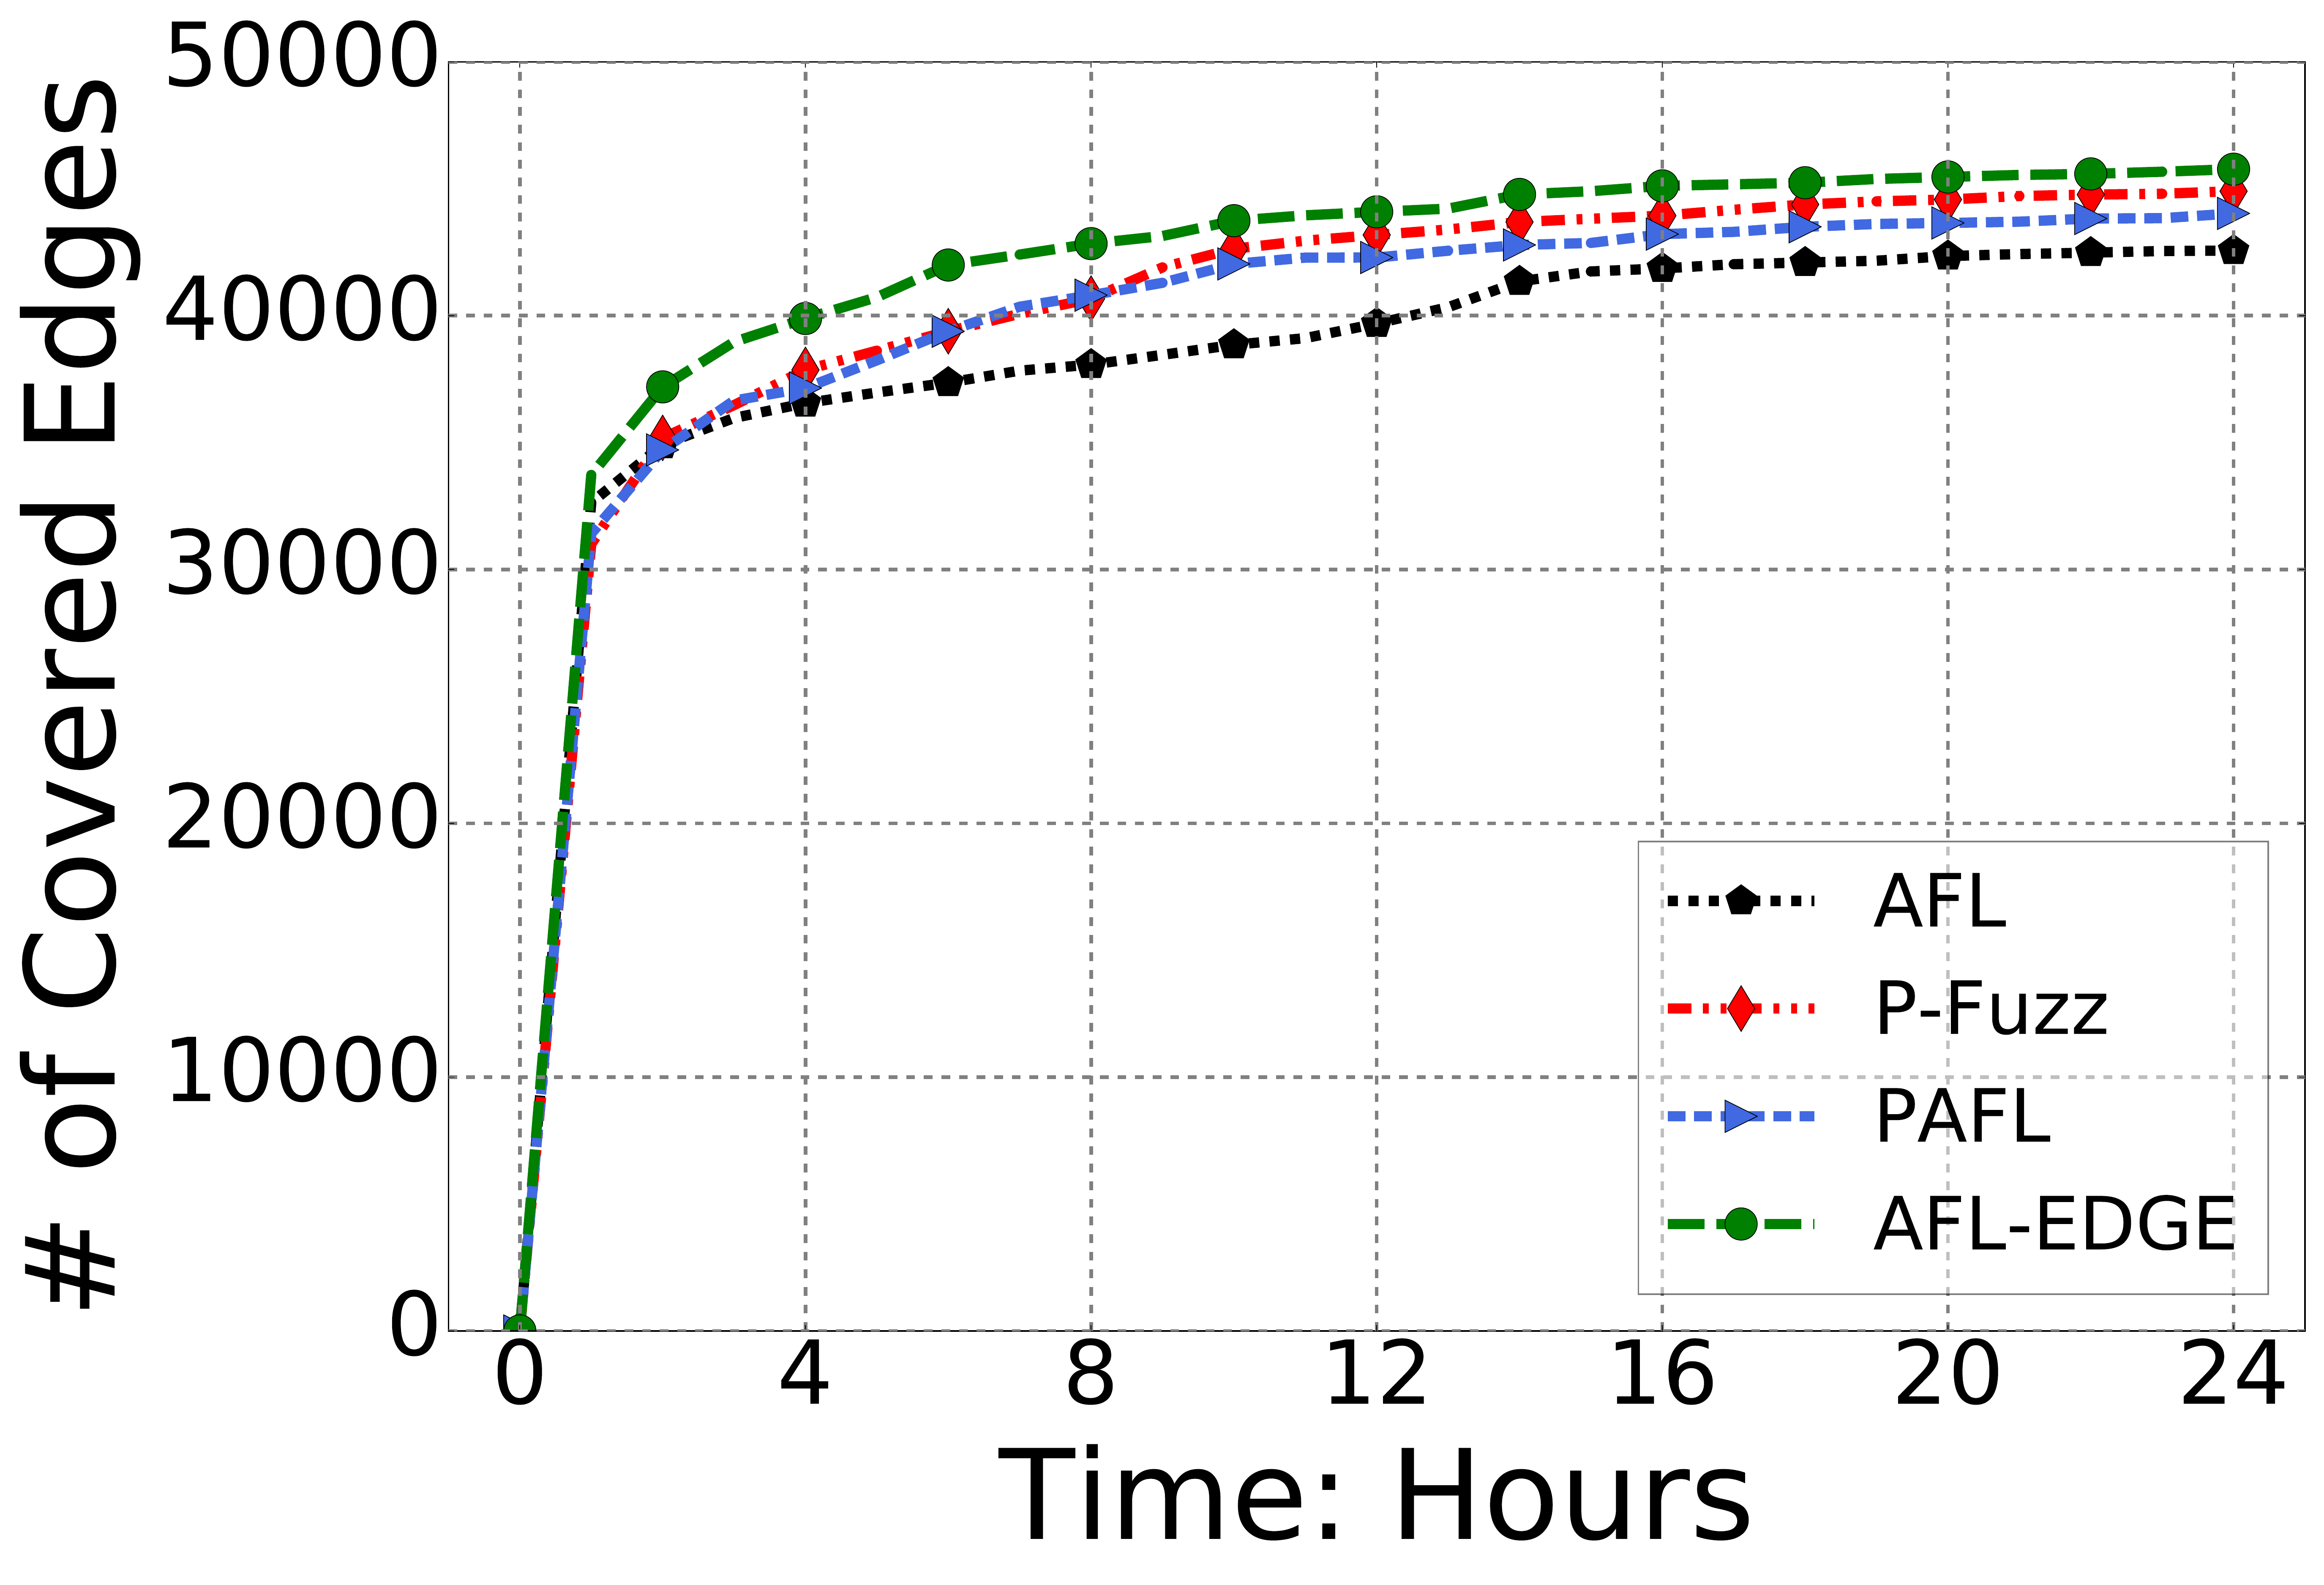} & 
         \includegraphics[scale=0.075]{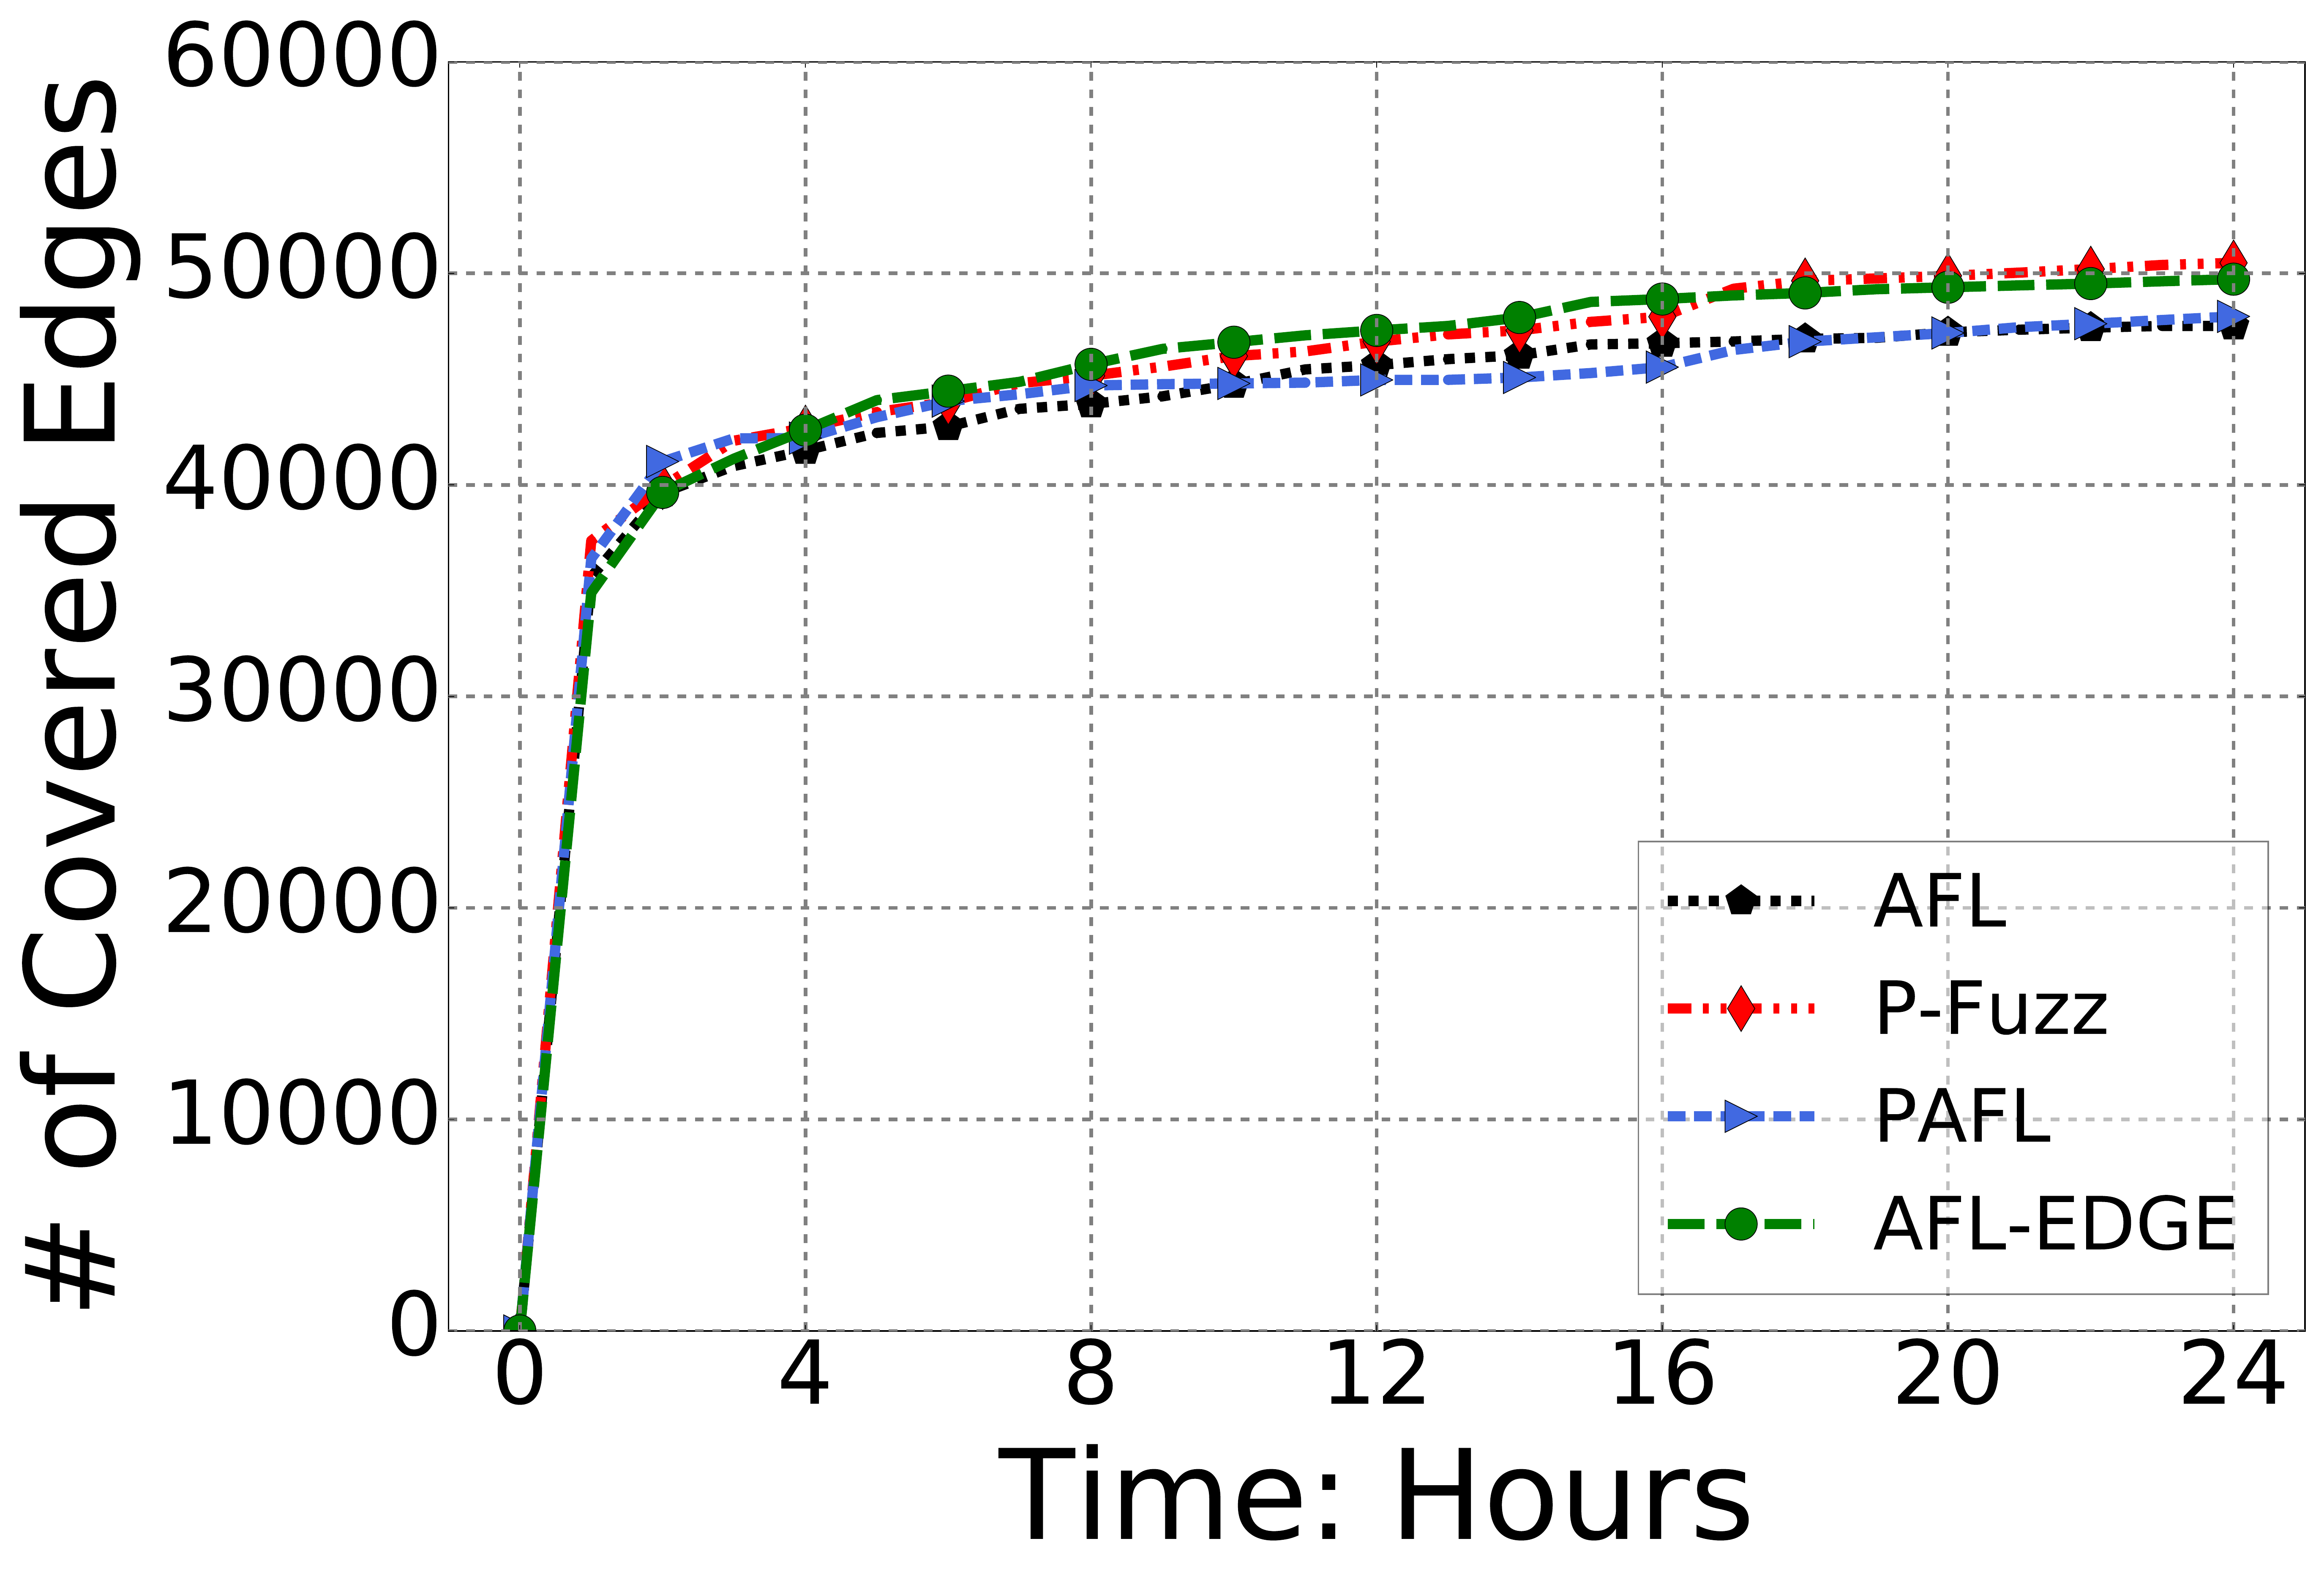} &
         \includegraphics[scale=0.075]{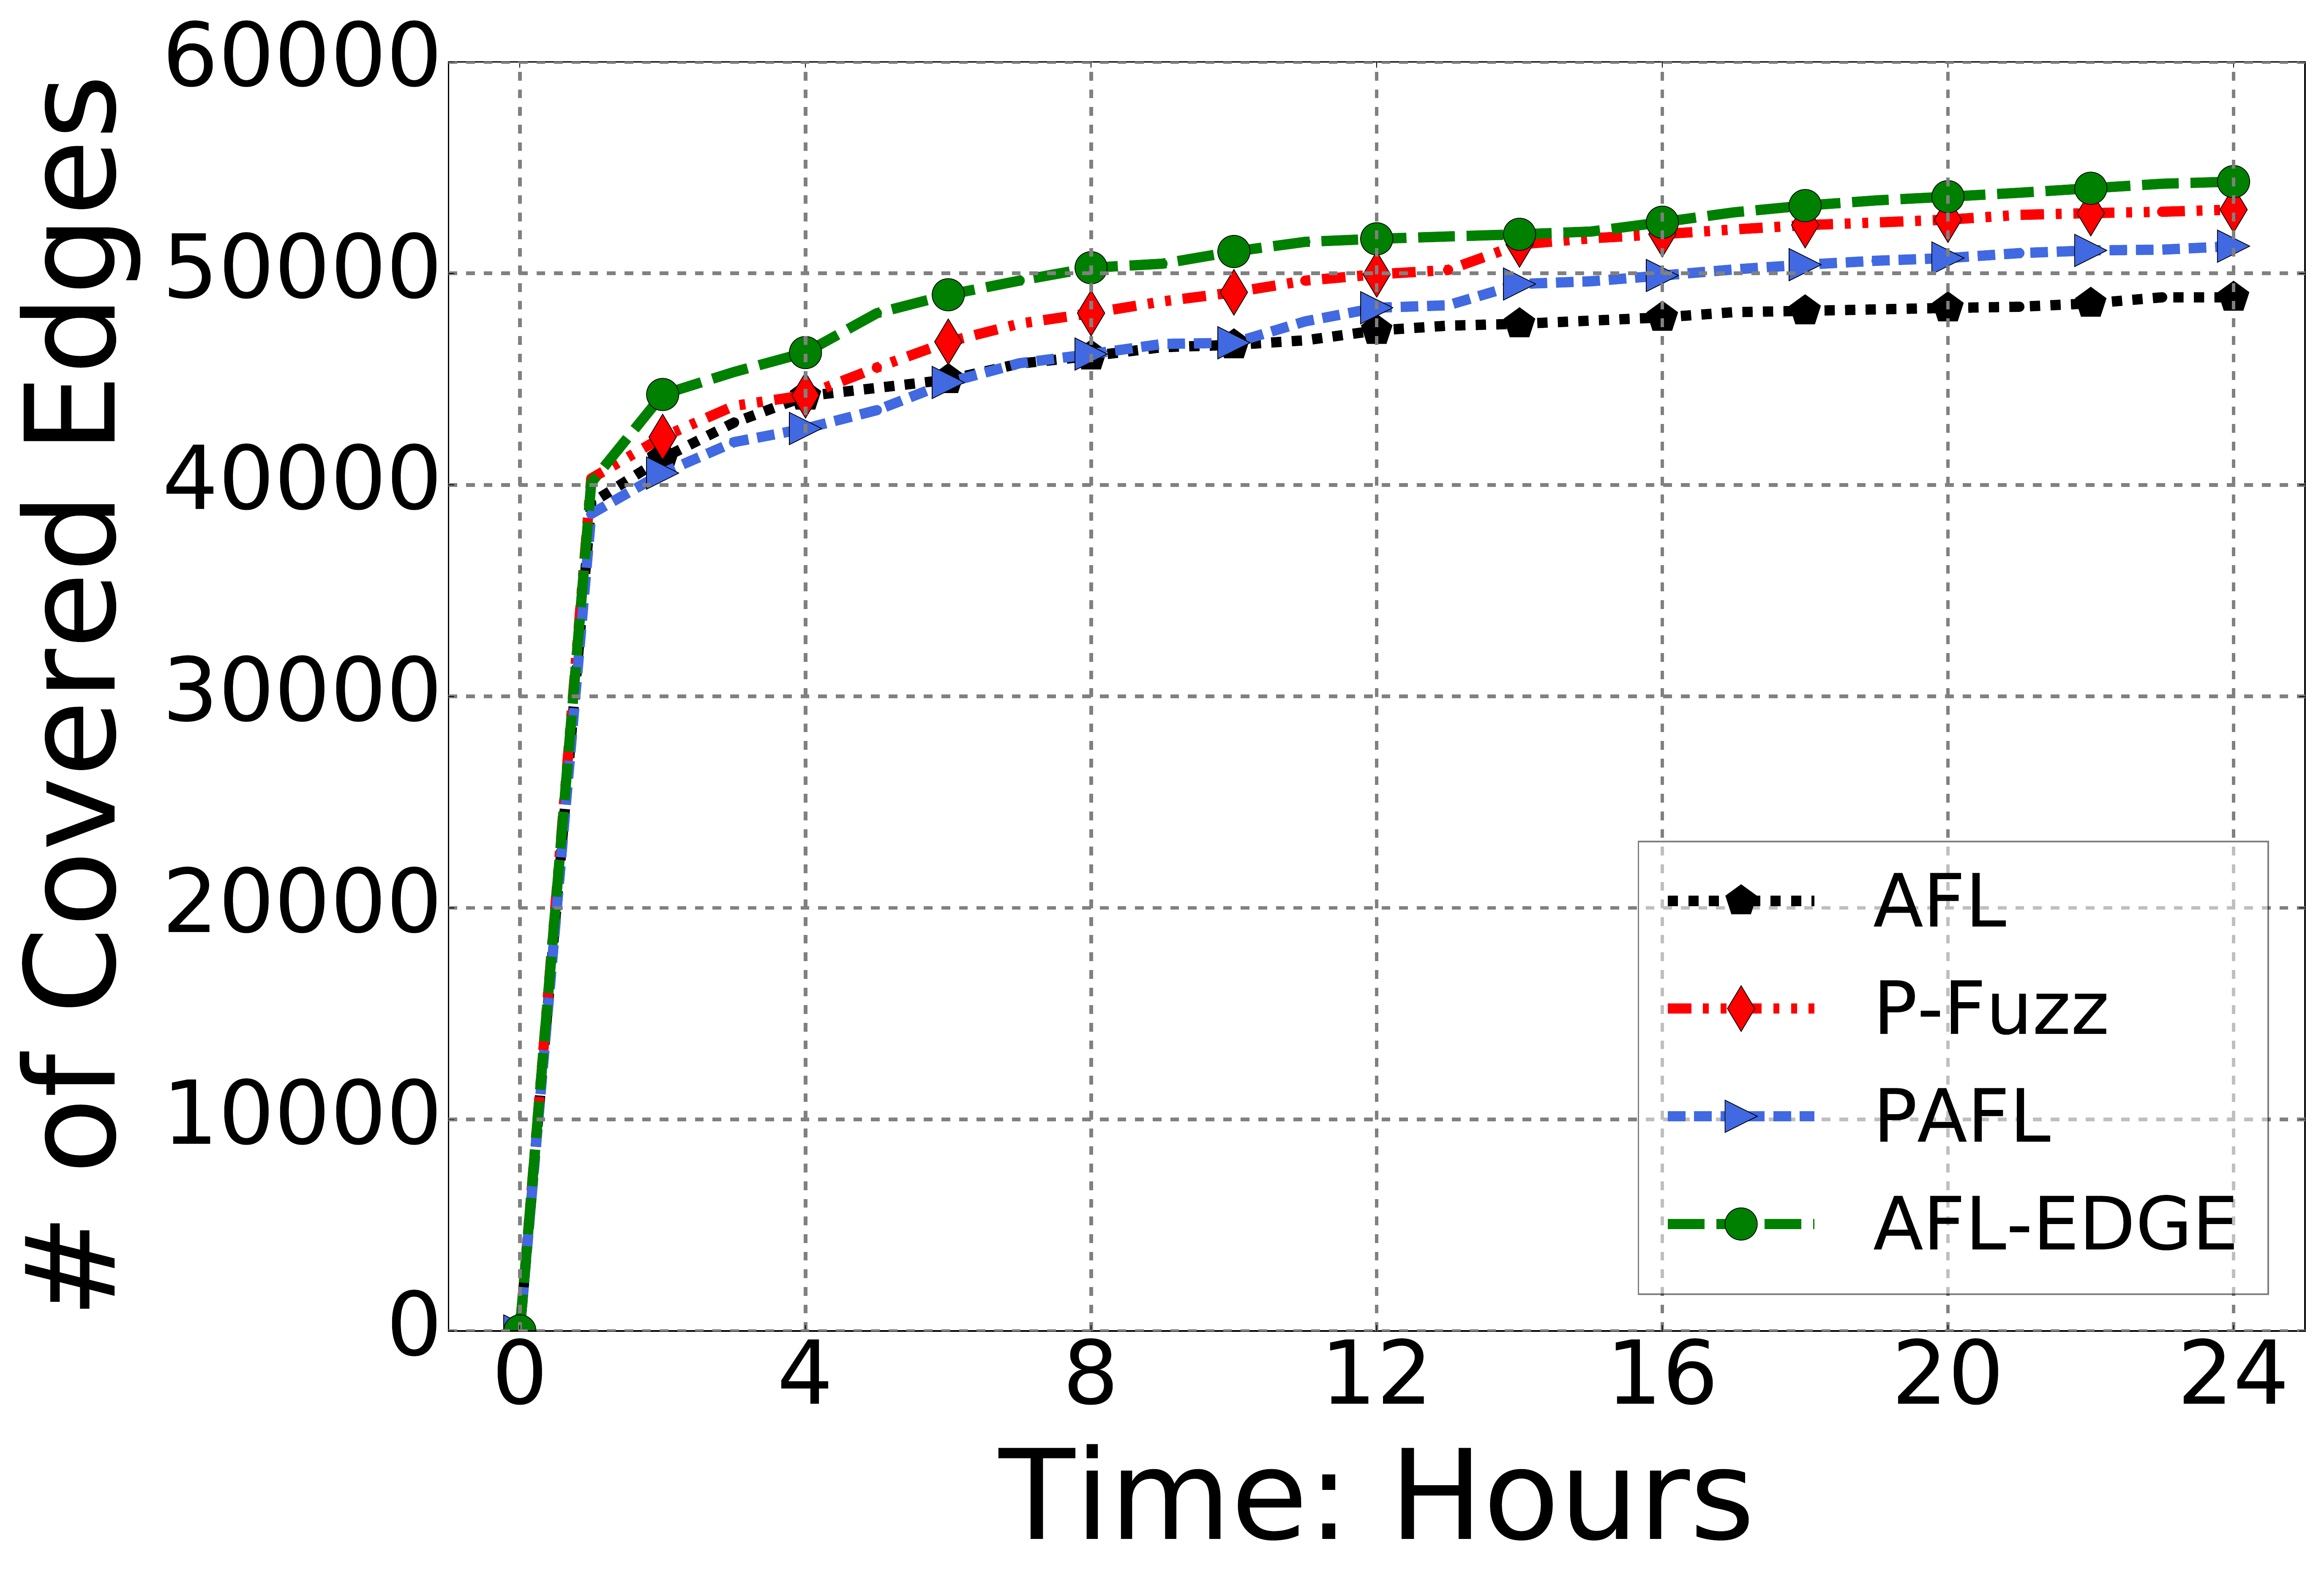} 
         \\
         {\scriptsize\textbf{tiff2pdf} \scriptsize 2 instances AFL} &
         {\scriptsize\textbf{tiff2pdf} \scriptsize 4 instances AFL} &
         {\scriptsize\textbf{tiff2pdf} \scriptsize 8 instances AFL} 
        %  {\scriptsize\textbf{tiff2pdf} \scriptsize 2 instance QSYM} &
        %  {\scriptsize\textbf{tiff2pdf} \scriptsize 4 instance QSYM} &
        %  {\scriptsize\textbf{tiff2pdf} \scriptsize 8 instance QSYM} \\
         \\
         \includegraphics[scale=0.075]{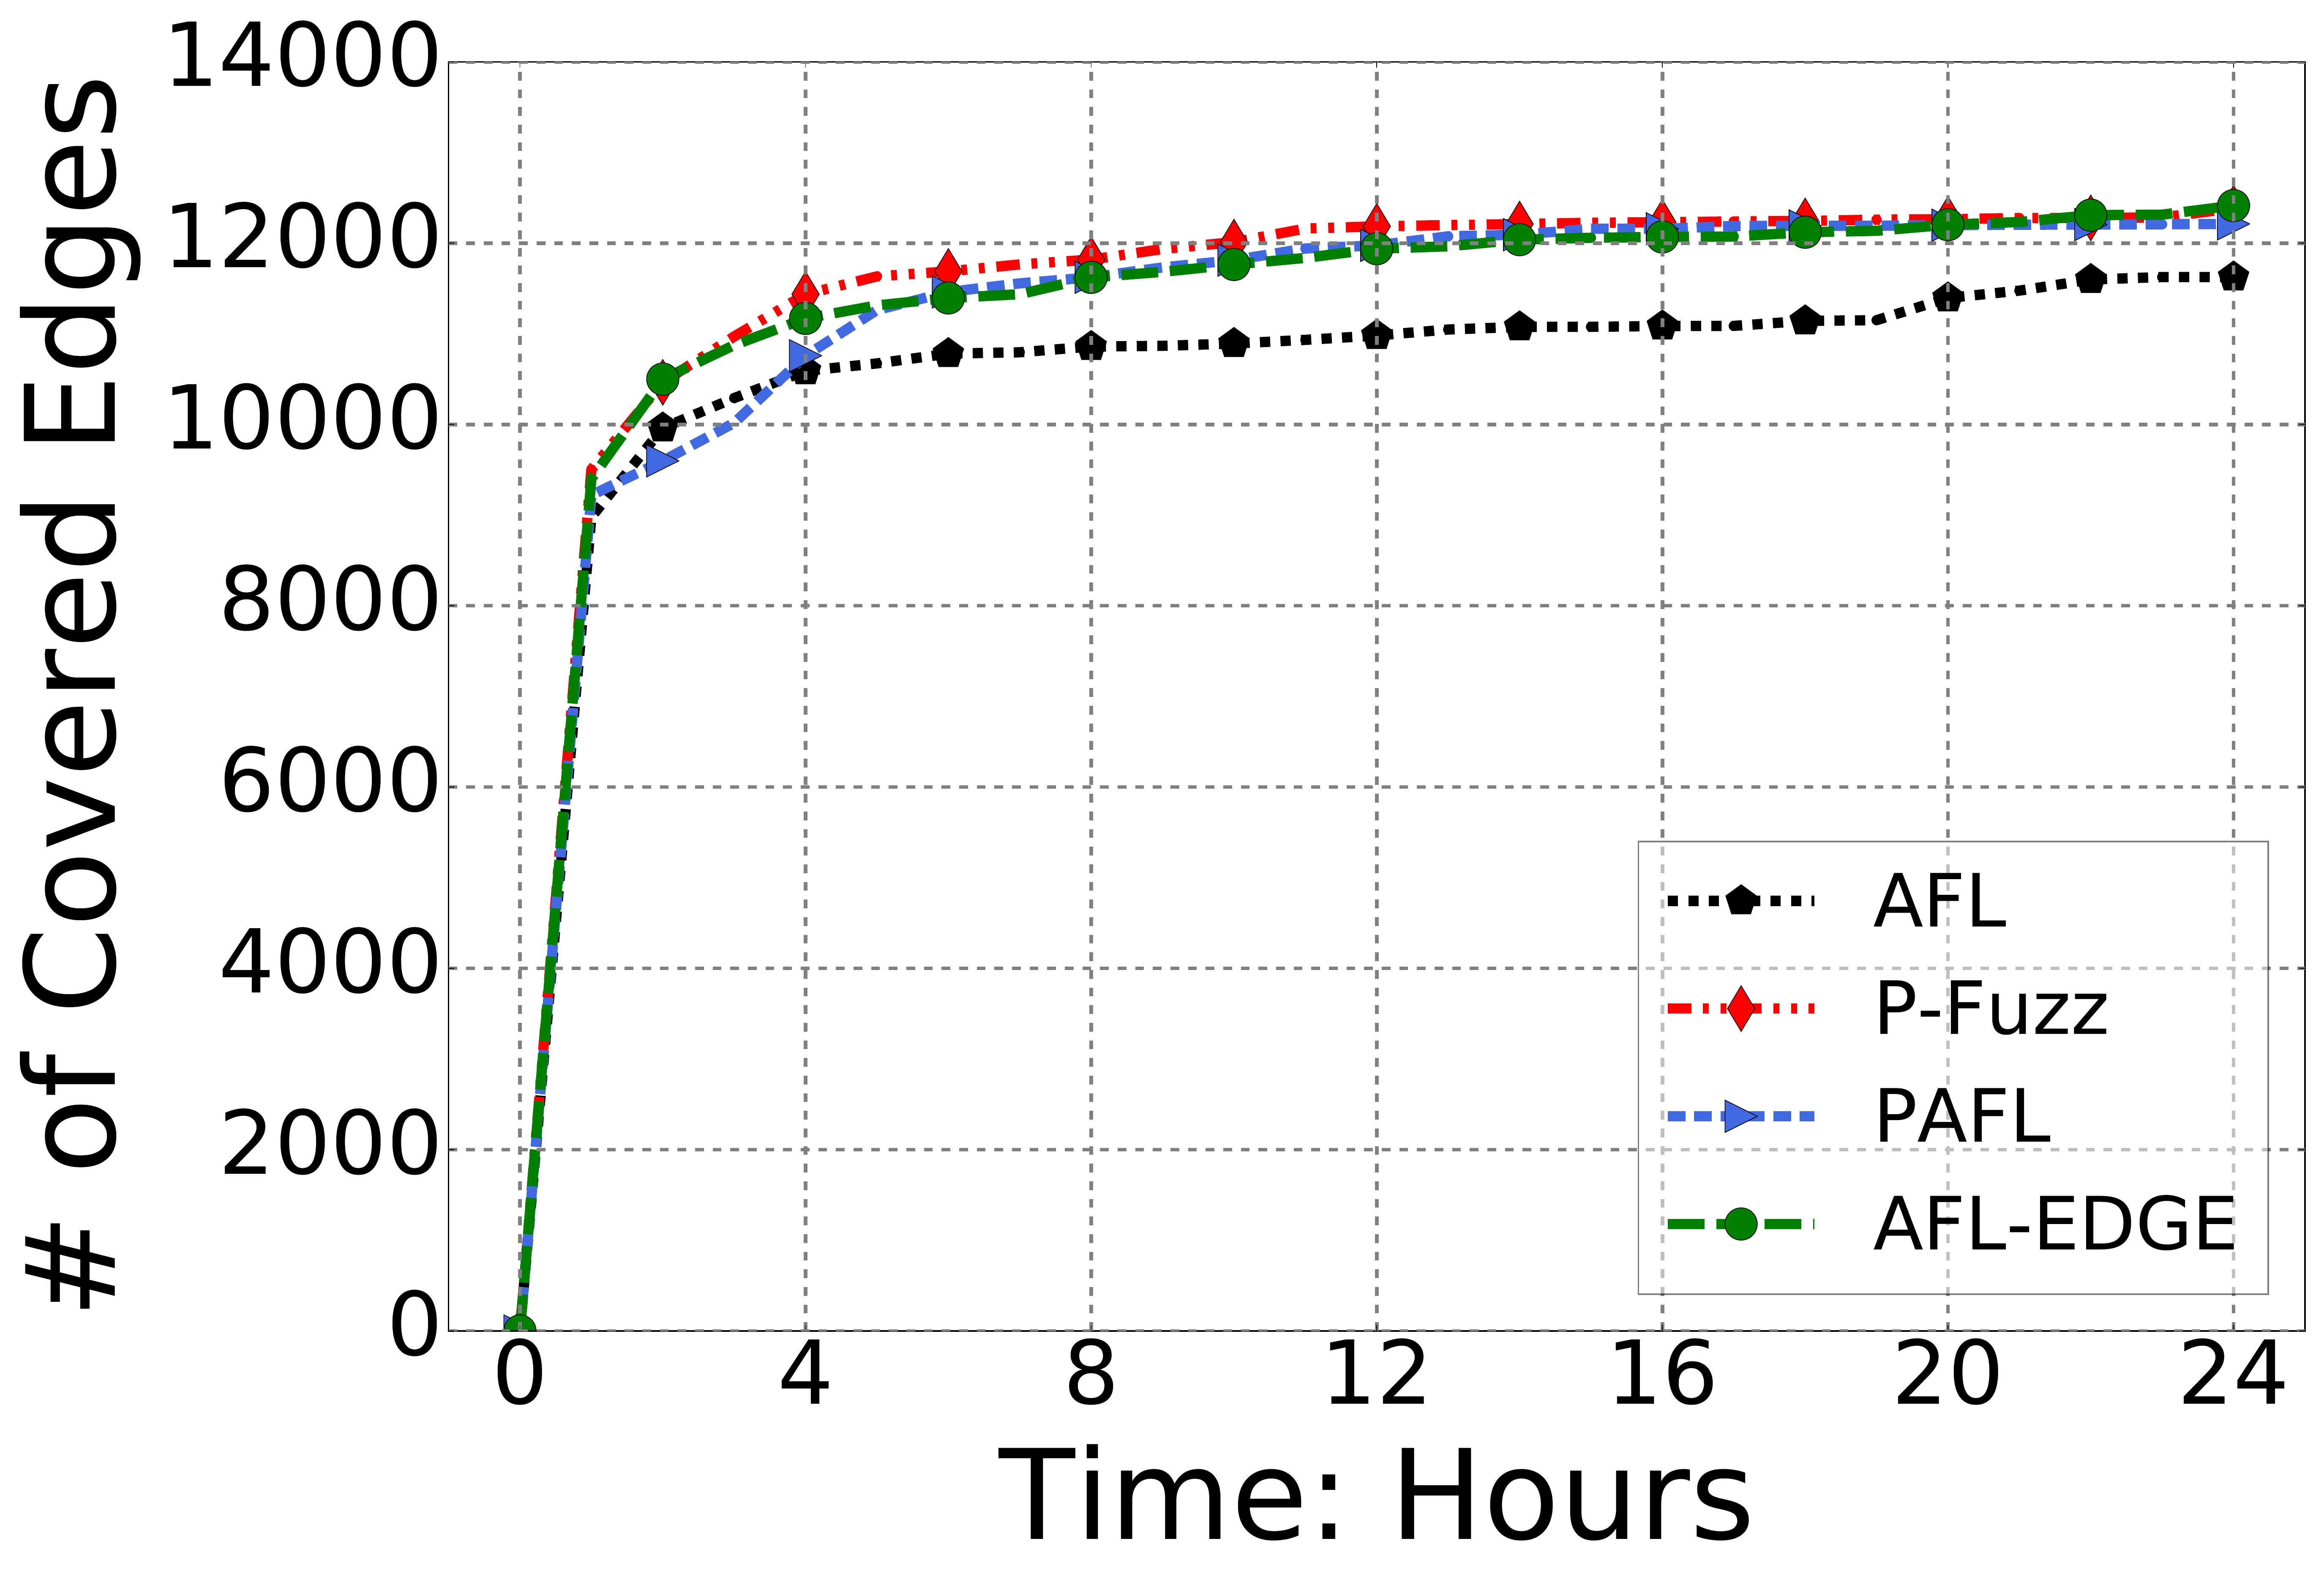} & 
         \includegraphics[scale=0.075]{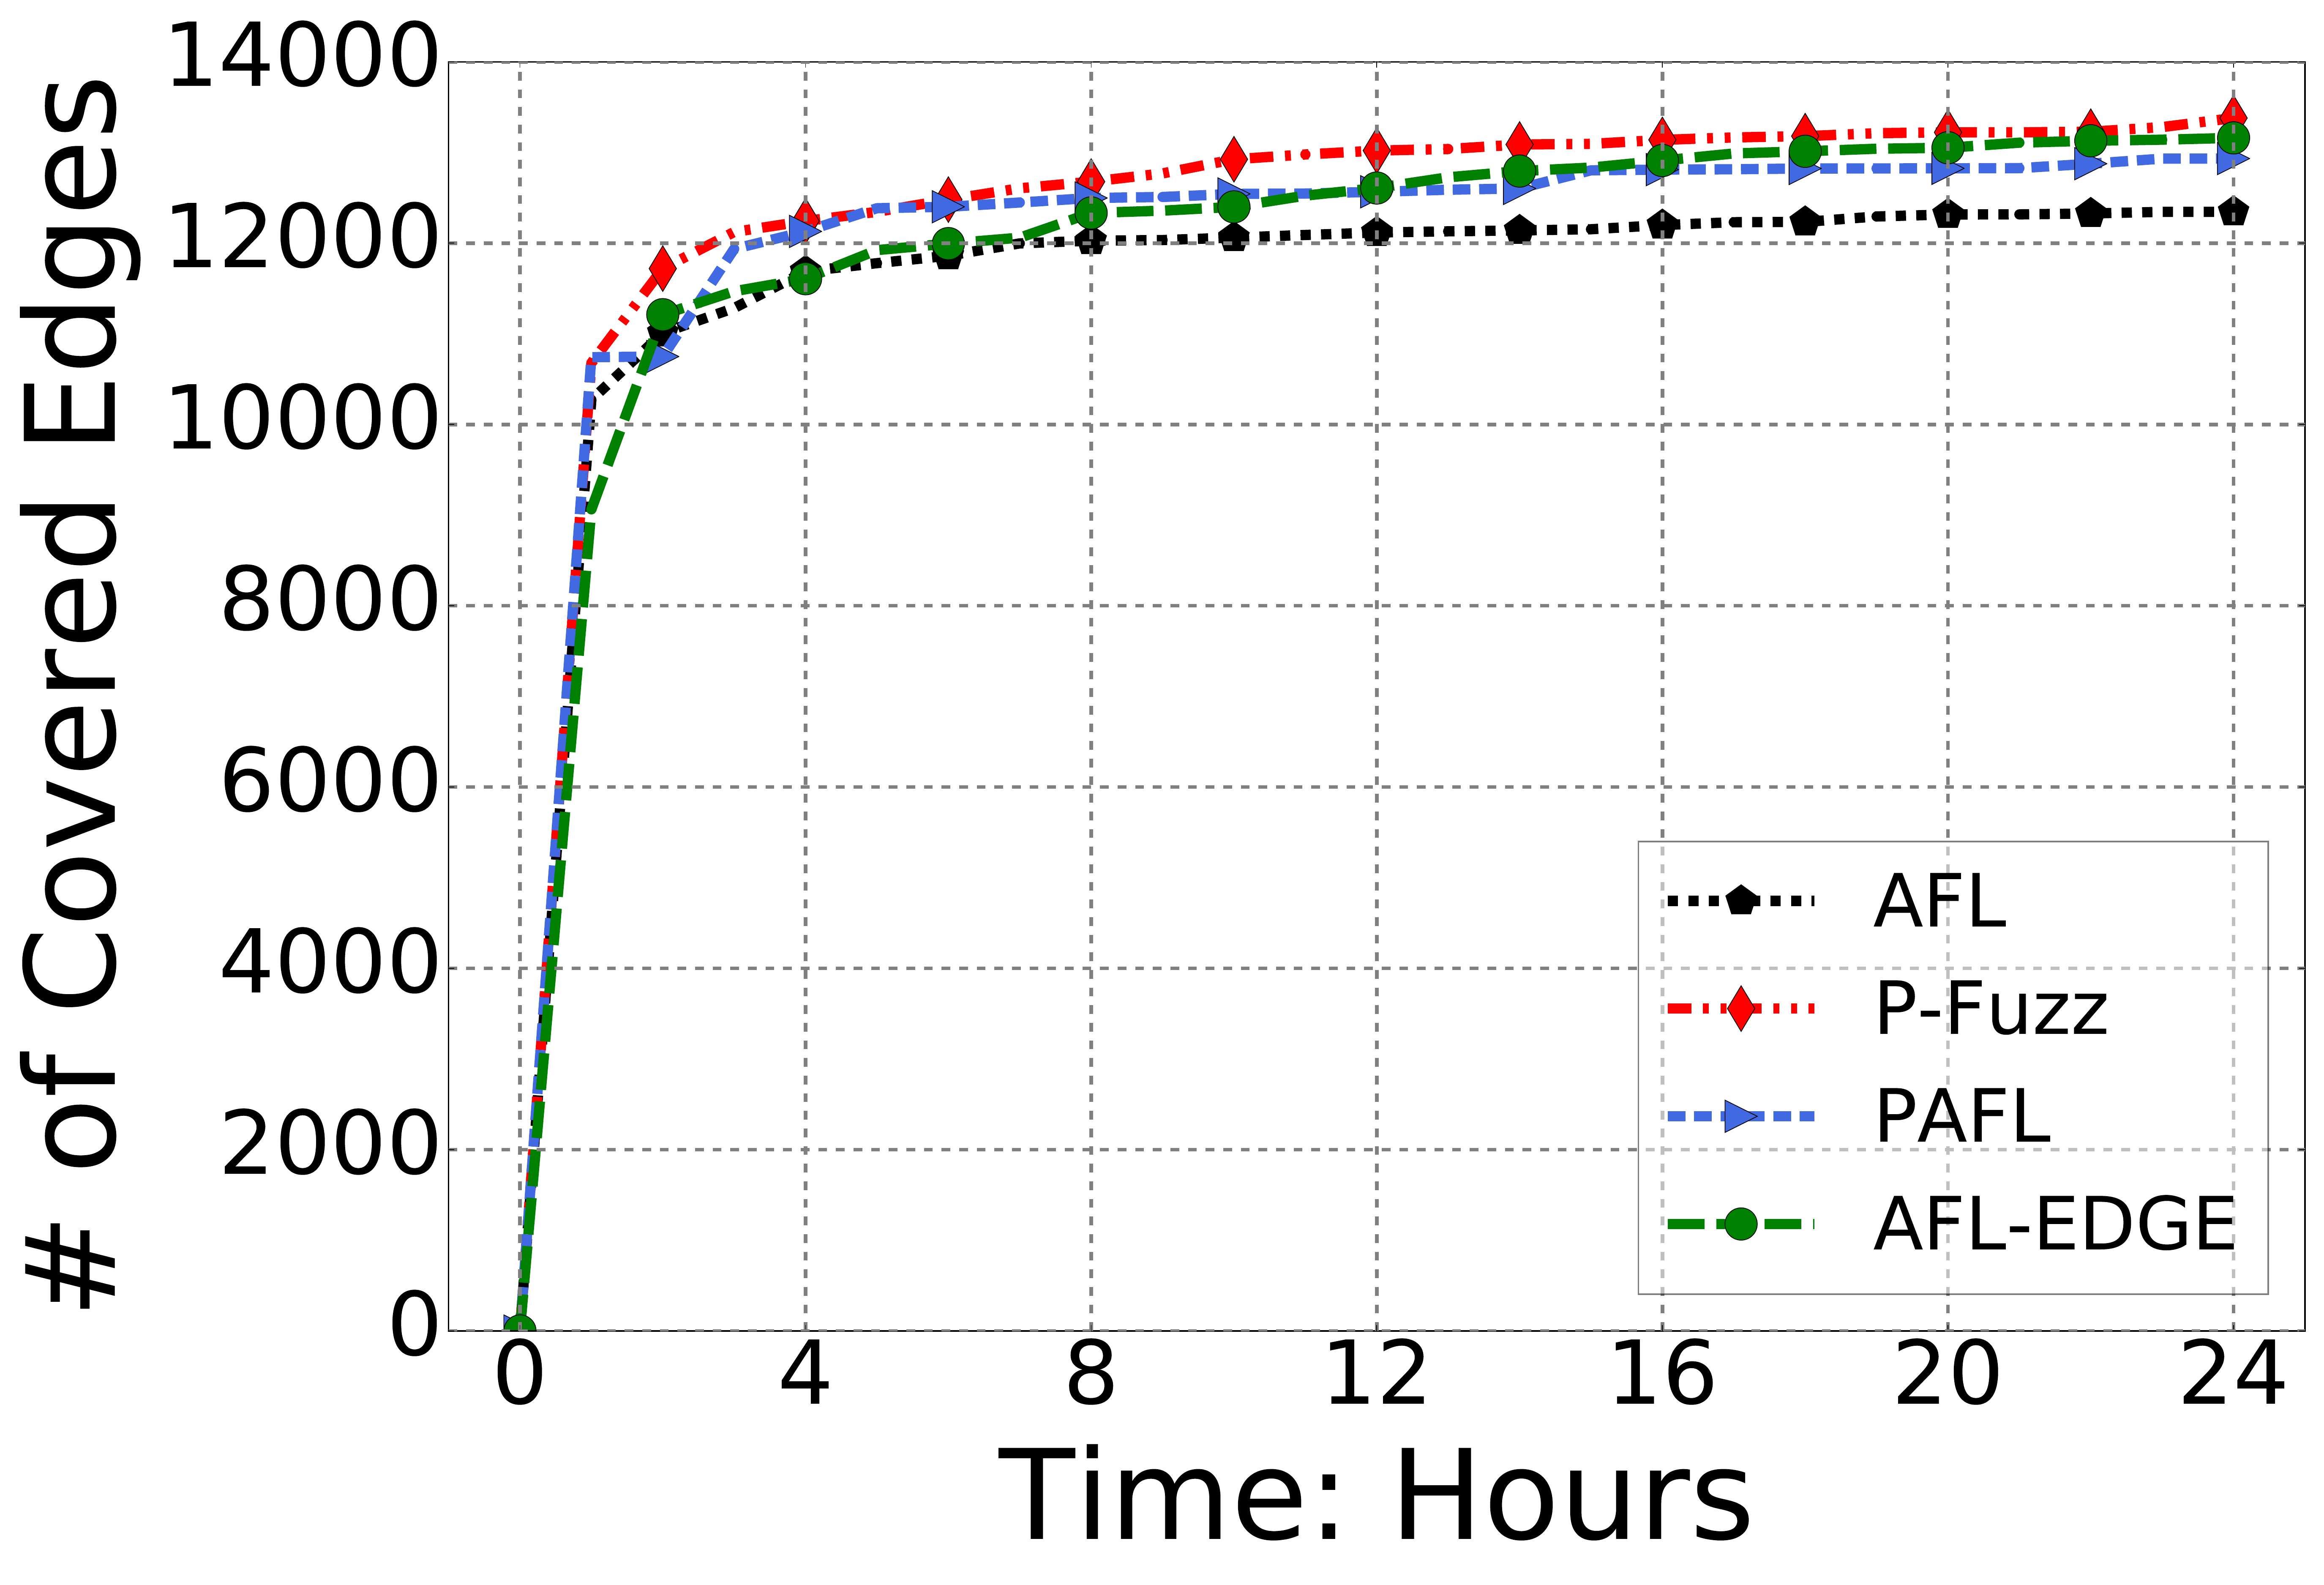} &
         \includegraphics[scale=0.075]{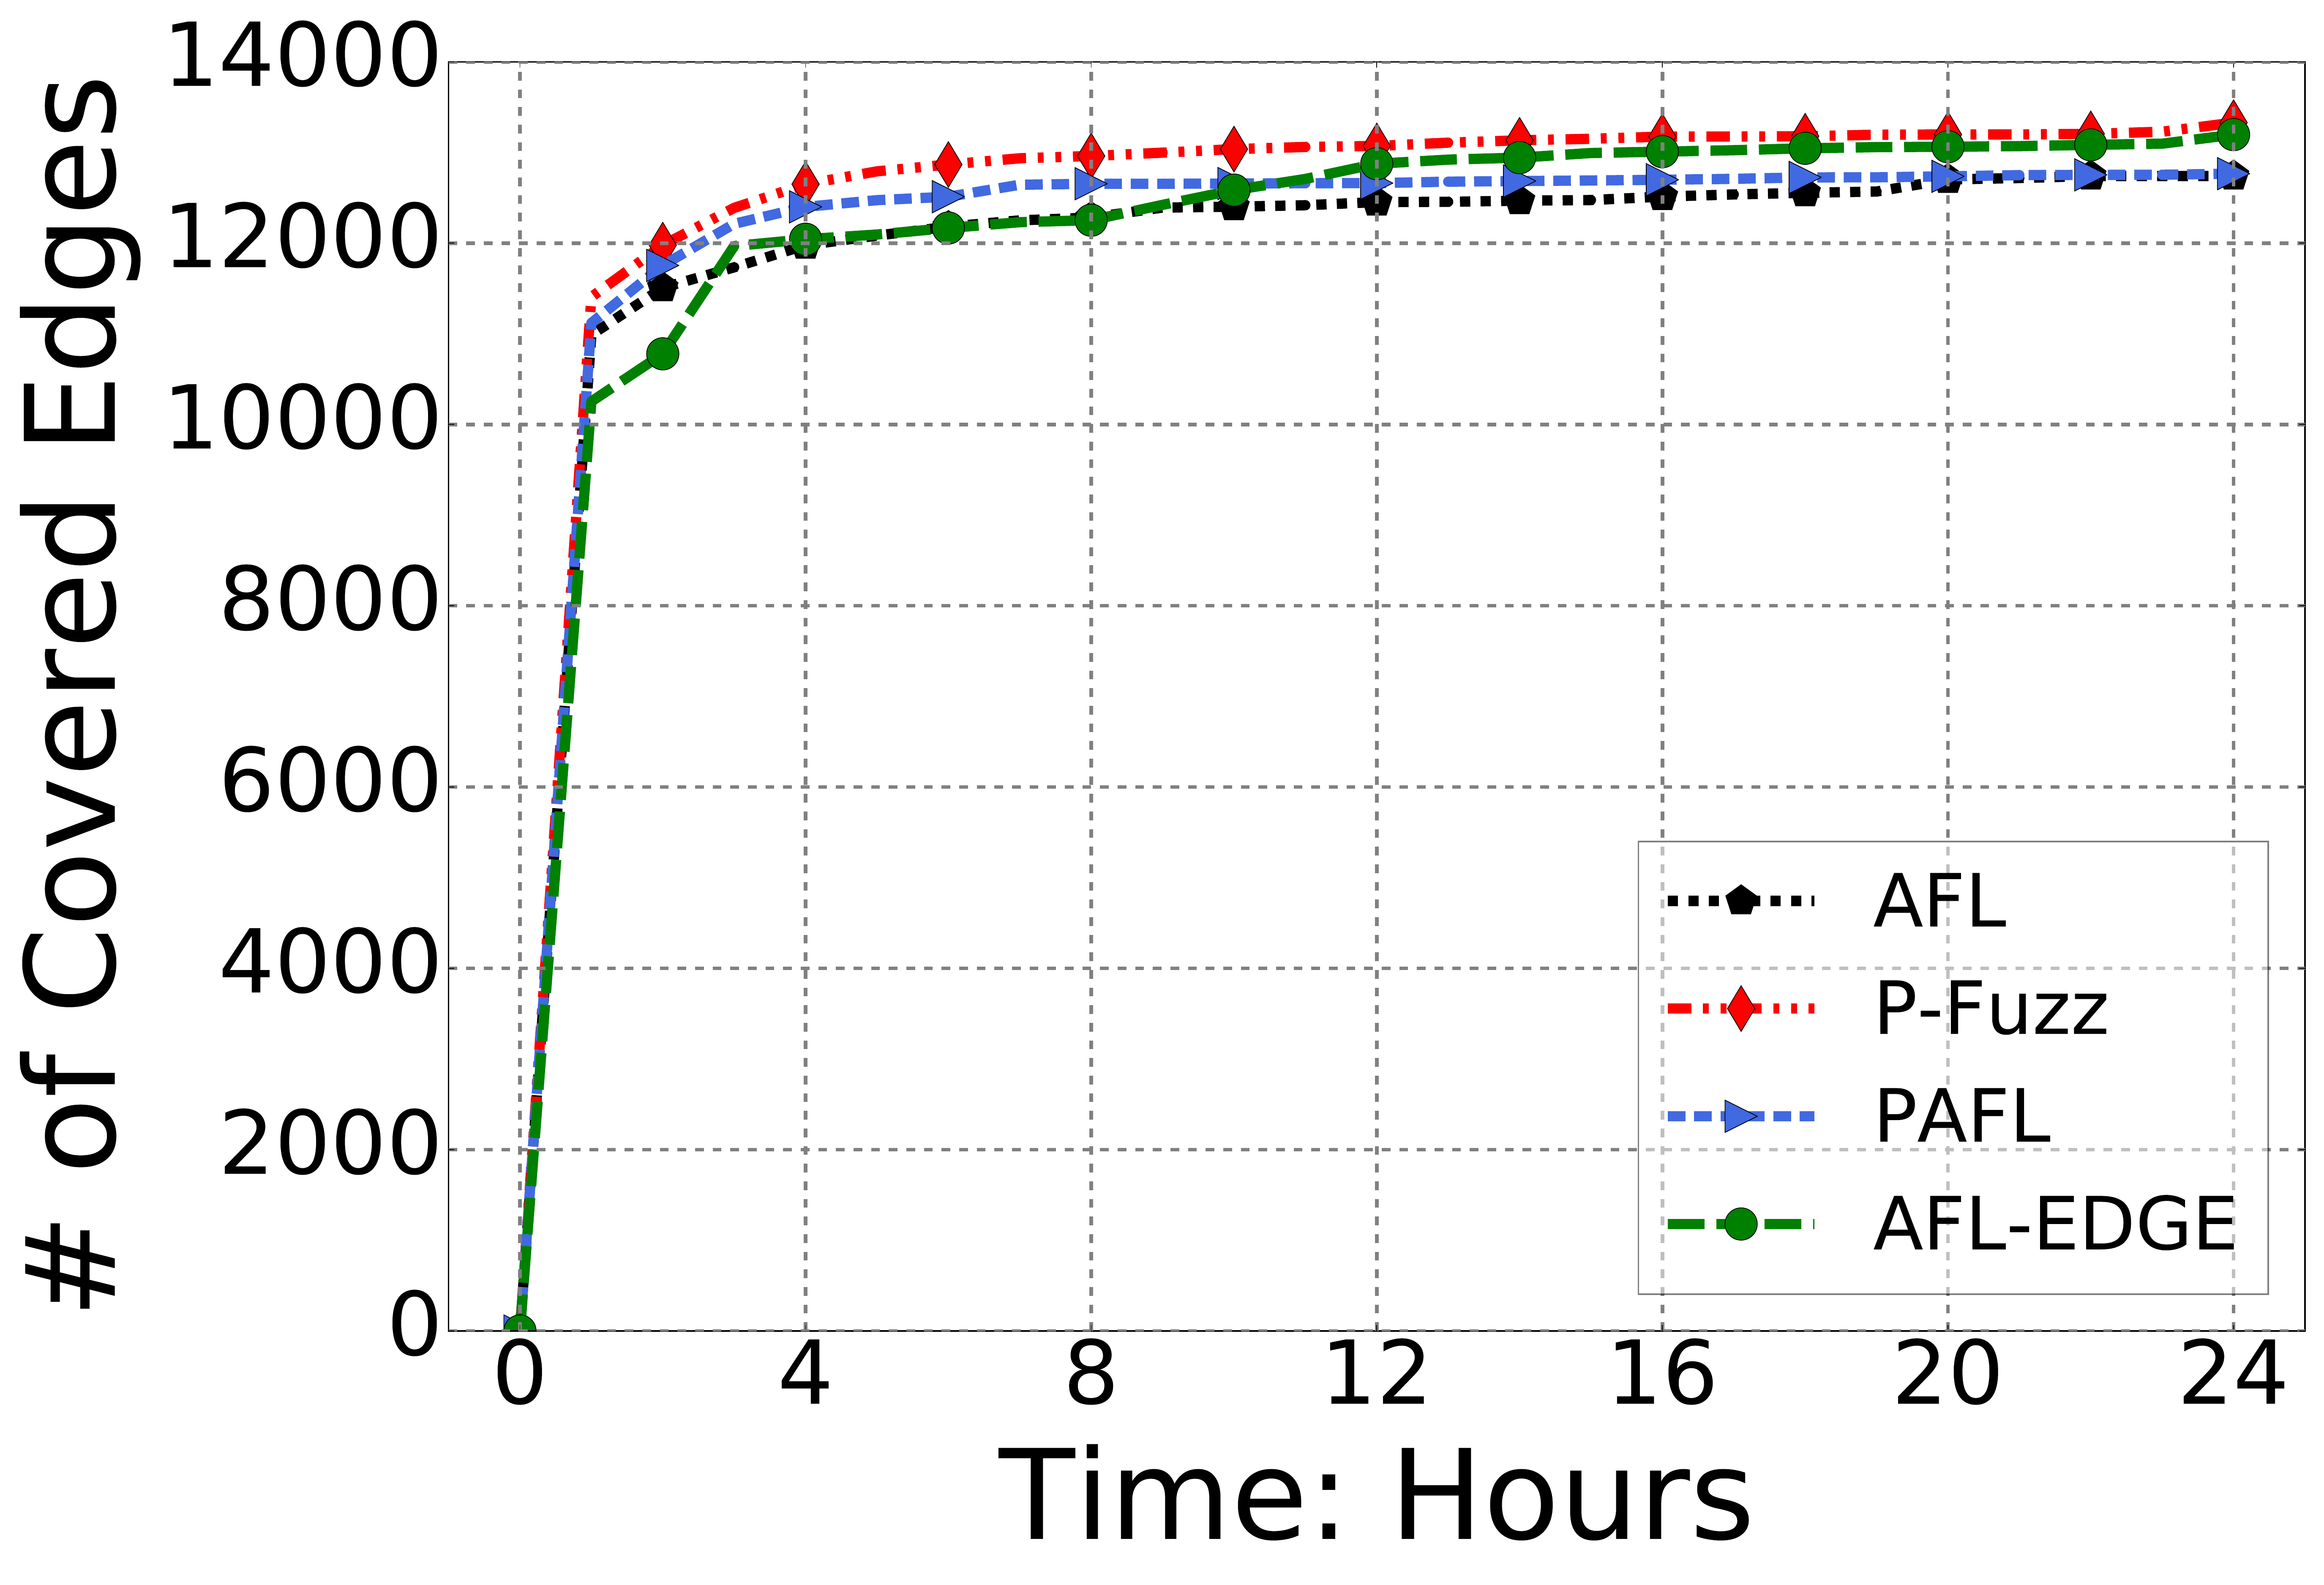} 
         \\
         {\scriptsize\textbf{nm-new} \scriptsize 2 instances AFL} &
         {\scriptsize\textbf{nm-new} \scriptsize 4 instances AFL} &
         {\scriptsize\textbf{nm-new} \scriptsize 8 instances AFL} 
        %  {\scriptsize\textbf{nm-new} \scriptsize 2 instance QSYM} &
        %  {\scriptsize\textbf{nm-new} \scriptsize 4 instance QSYM} &
        %  {\scriptsize\textbf{nm-new} \scriptsize 8 instance QSYM} \\
         \\
         \includegraphics[scale=0.075]{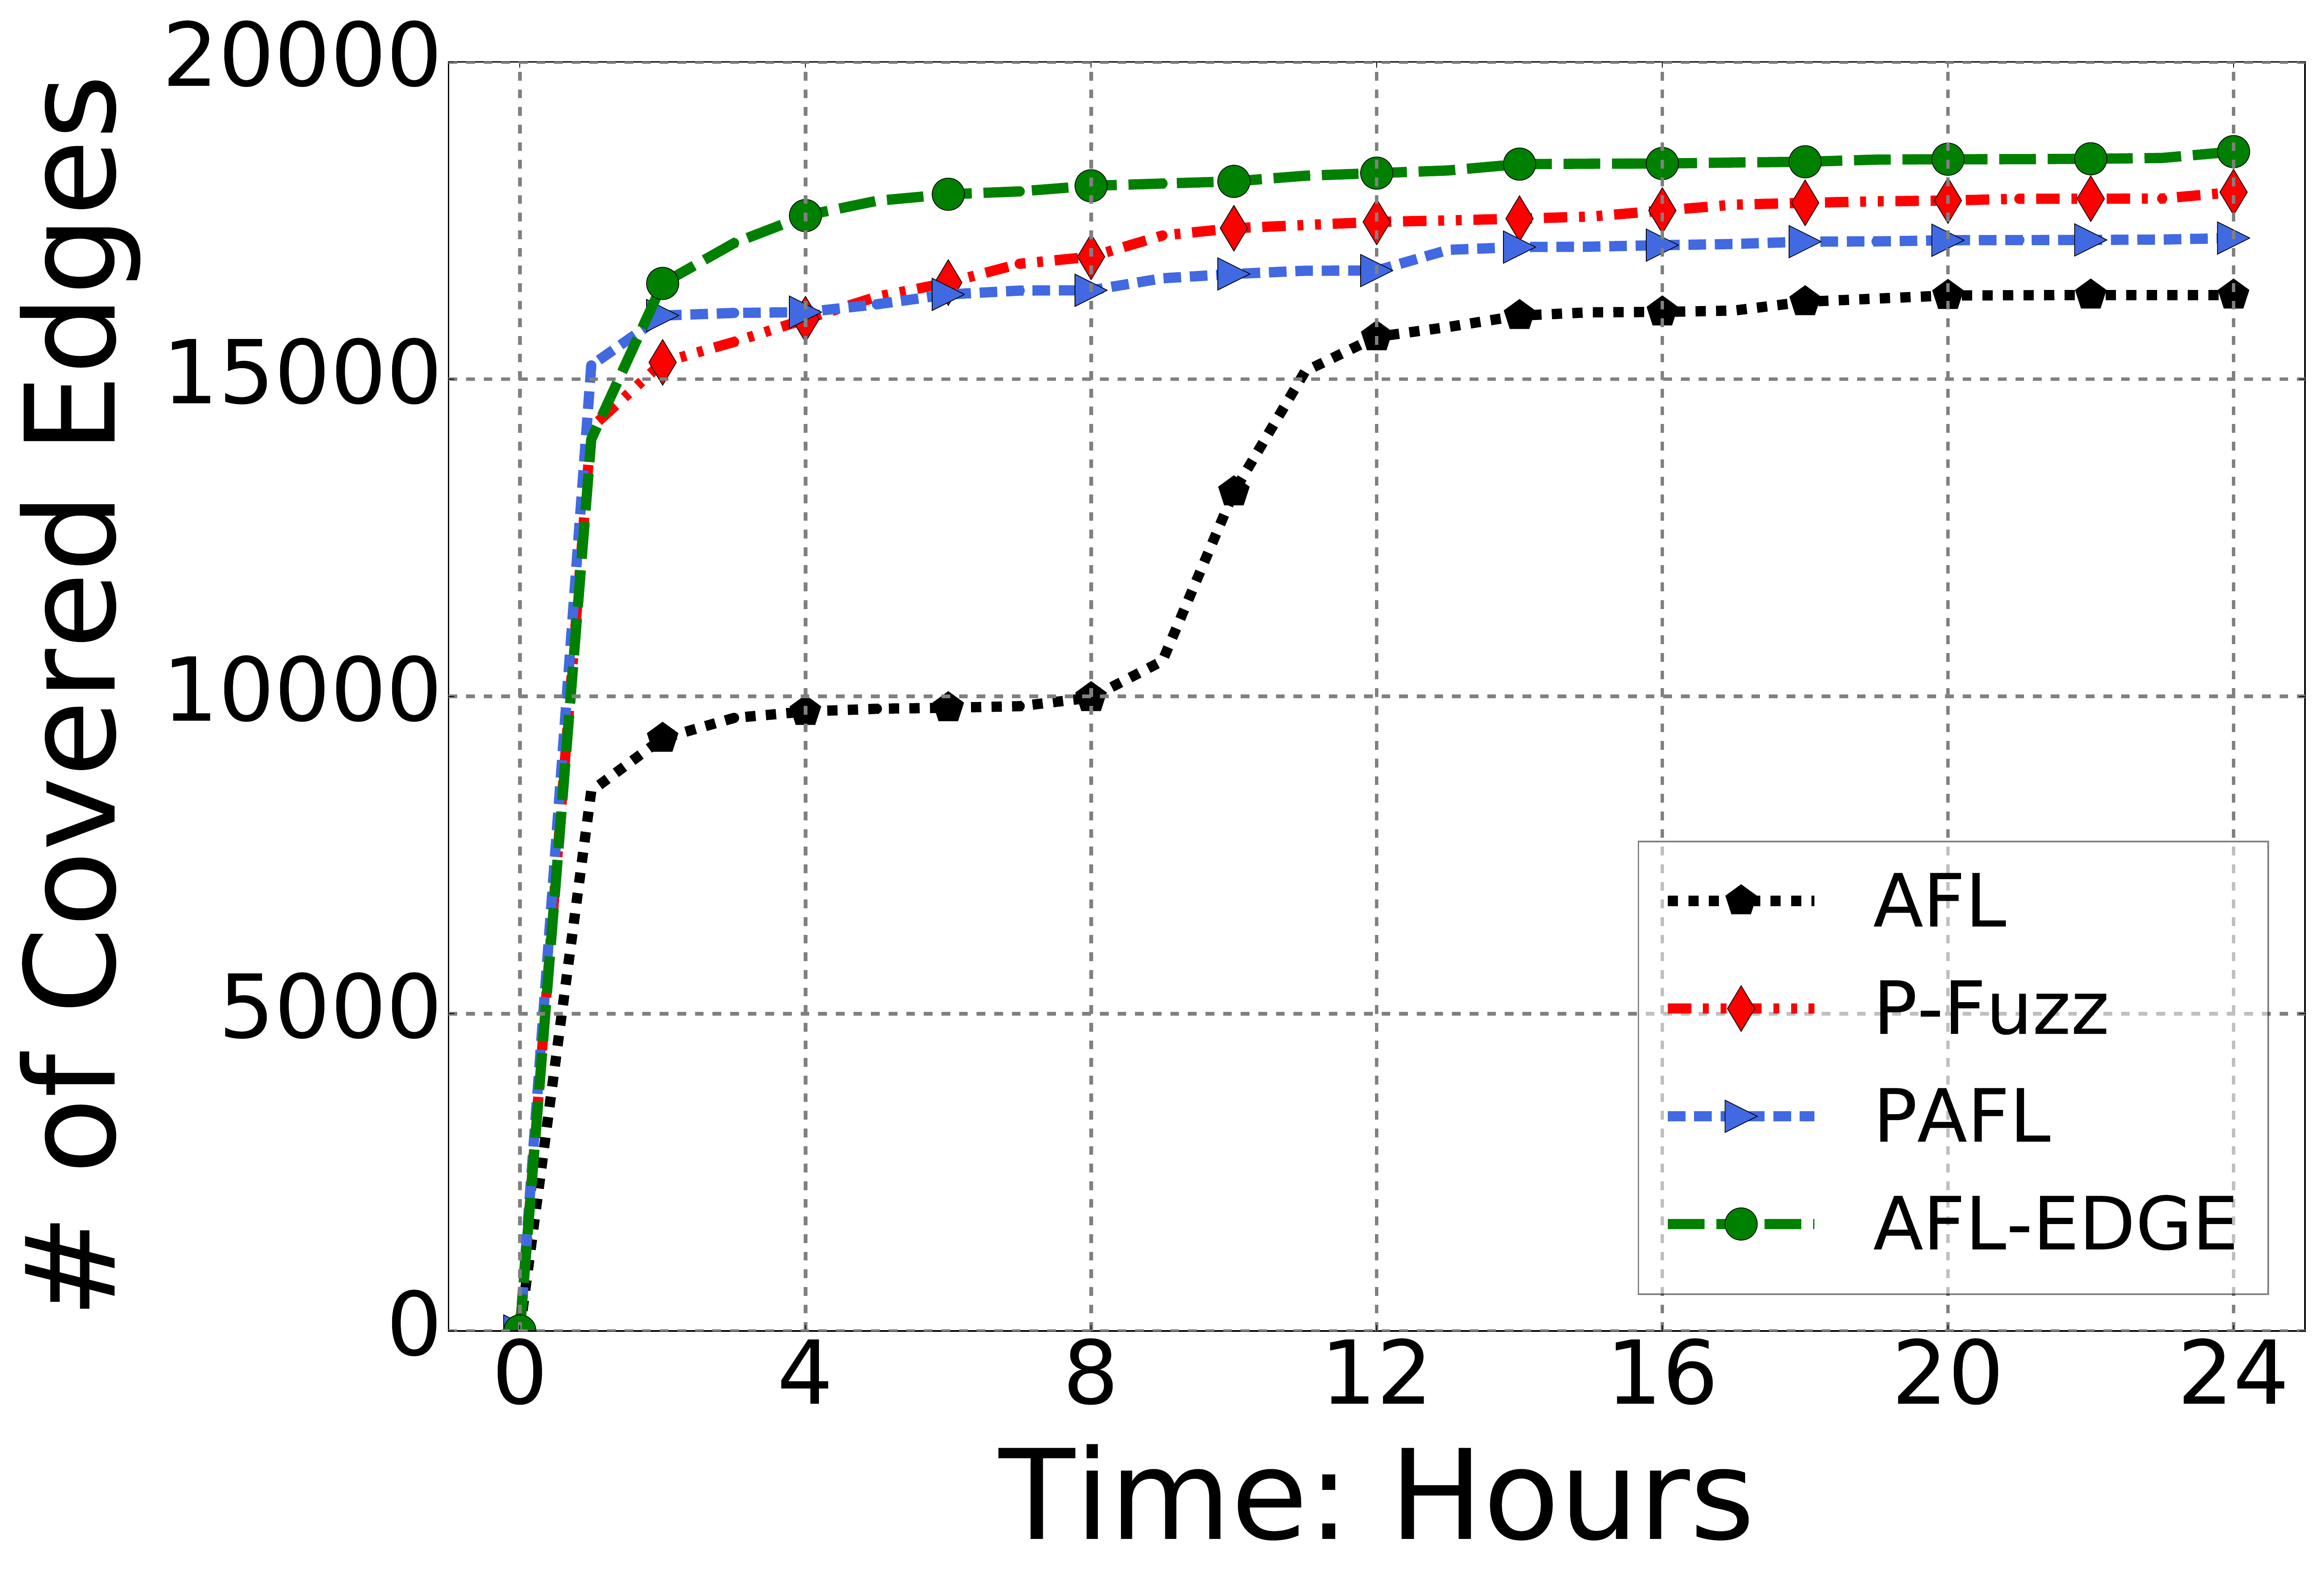} & 
         \includegraphics[scale=0.075]{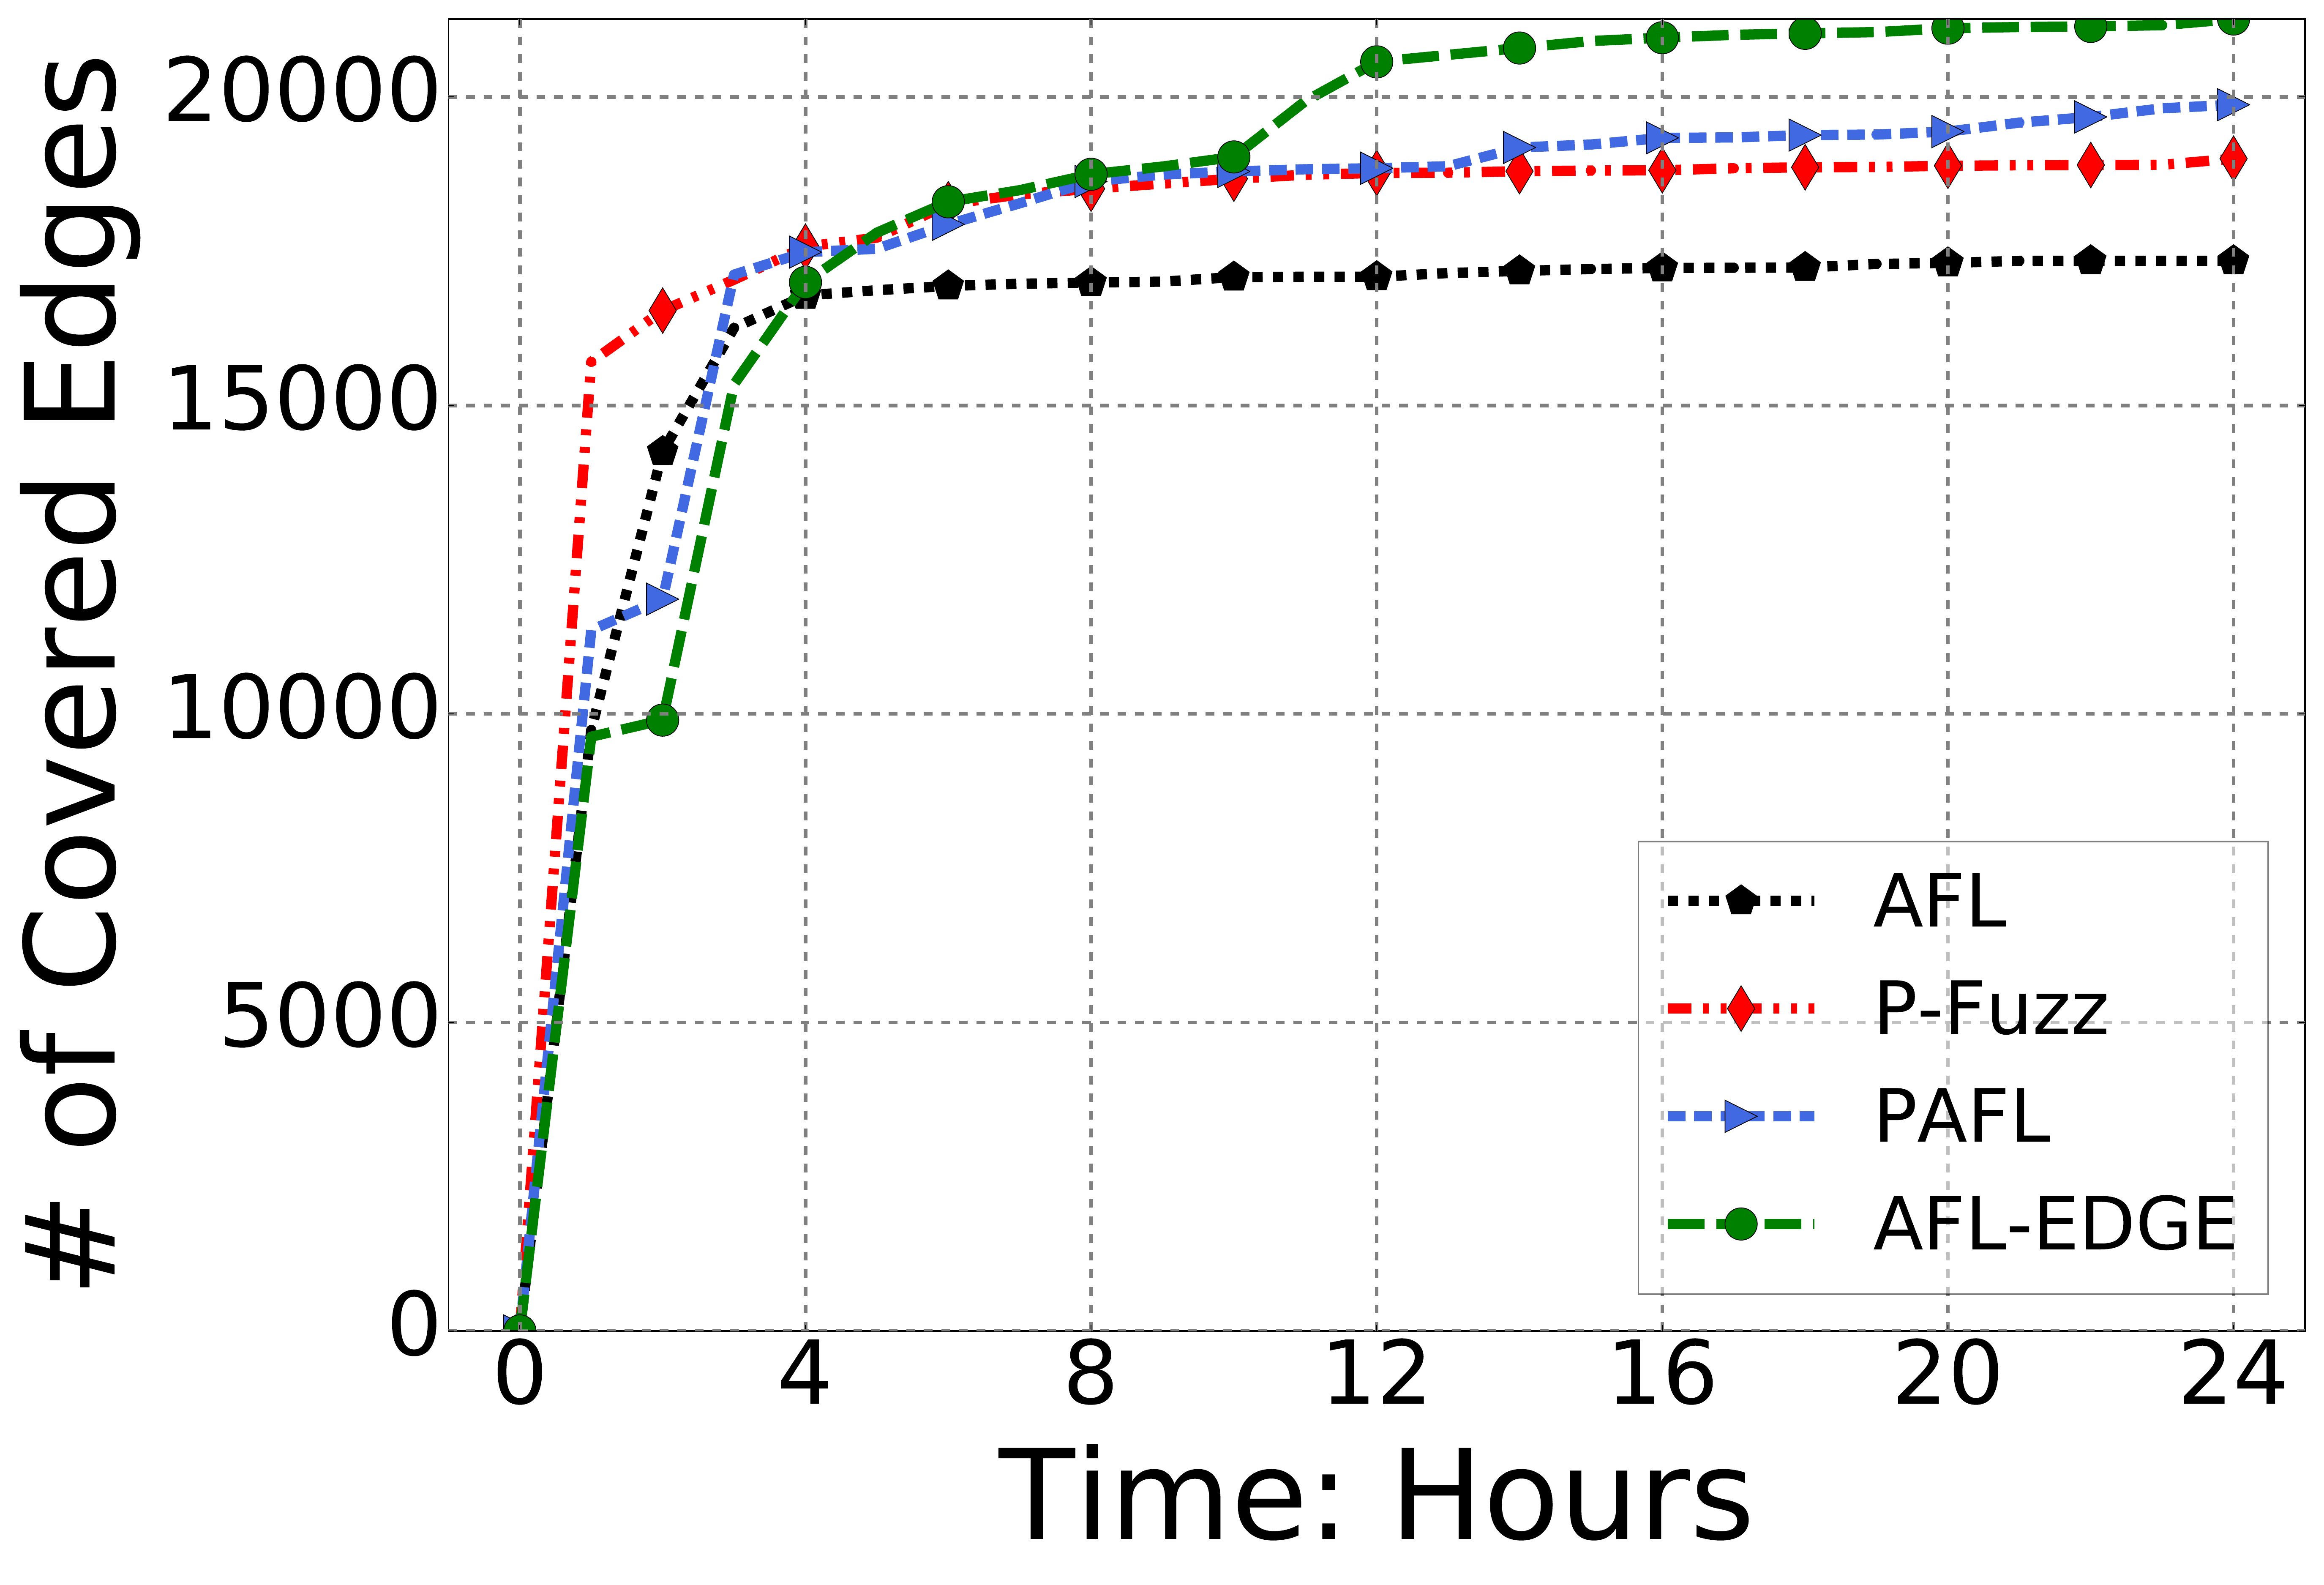} &
         \includegraphics[scale=0.075]{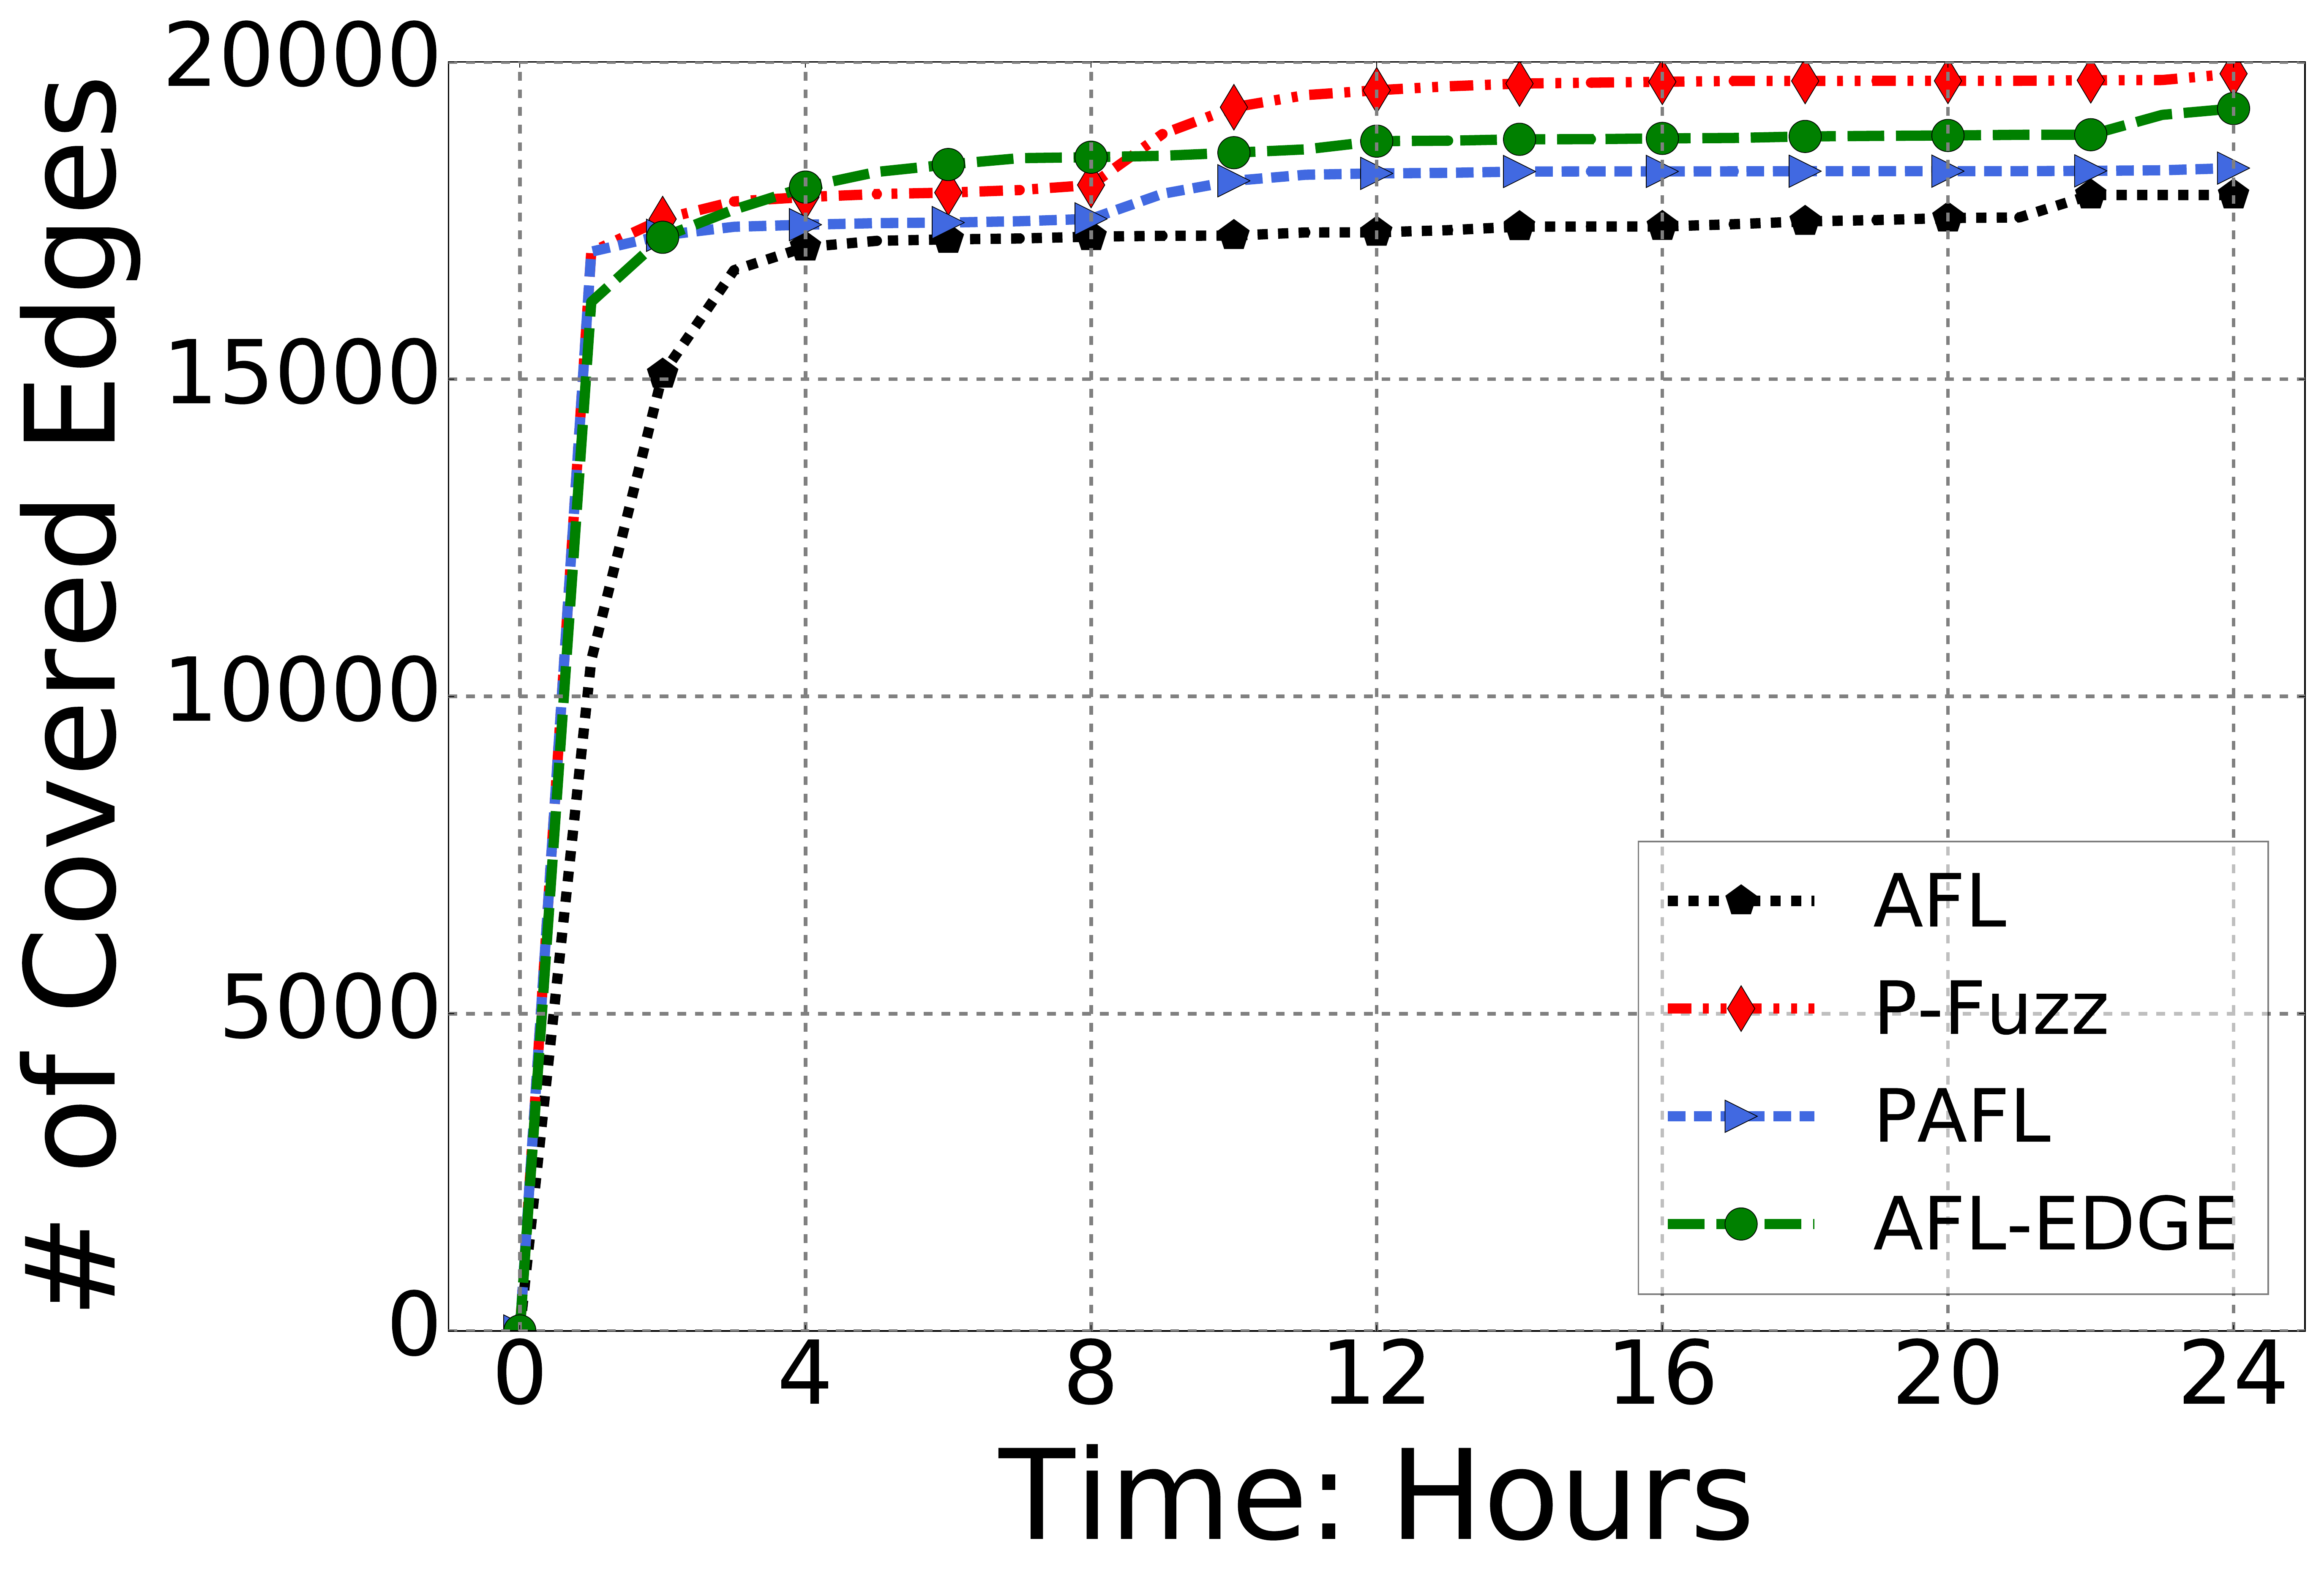}  
         \\
         {\scriptsize\textbf{nasm} \scriptsize 2 instances AFL} &
         {\scriptsize\textbf{nasm} \scriptsize 4 instances AFL} &
         {\scriptsize\textbf{nasm} \scriptsize 8 instances AFL} 
        %  {\scriptsize\textbf{nasm} \scriptsize 2 instance QSYM} &
        %  {\scriptsize\textbf{nasm} \scriptsize 4 instance QSYM} &
        %  {\scriptsize\textbf{nasm} \scriptsize 8 instance QSYM} \\
         \\
         \includegraphics[scale=0.075]{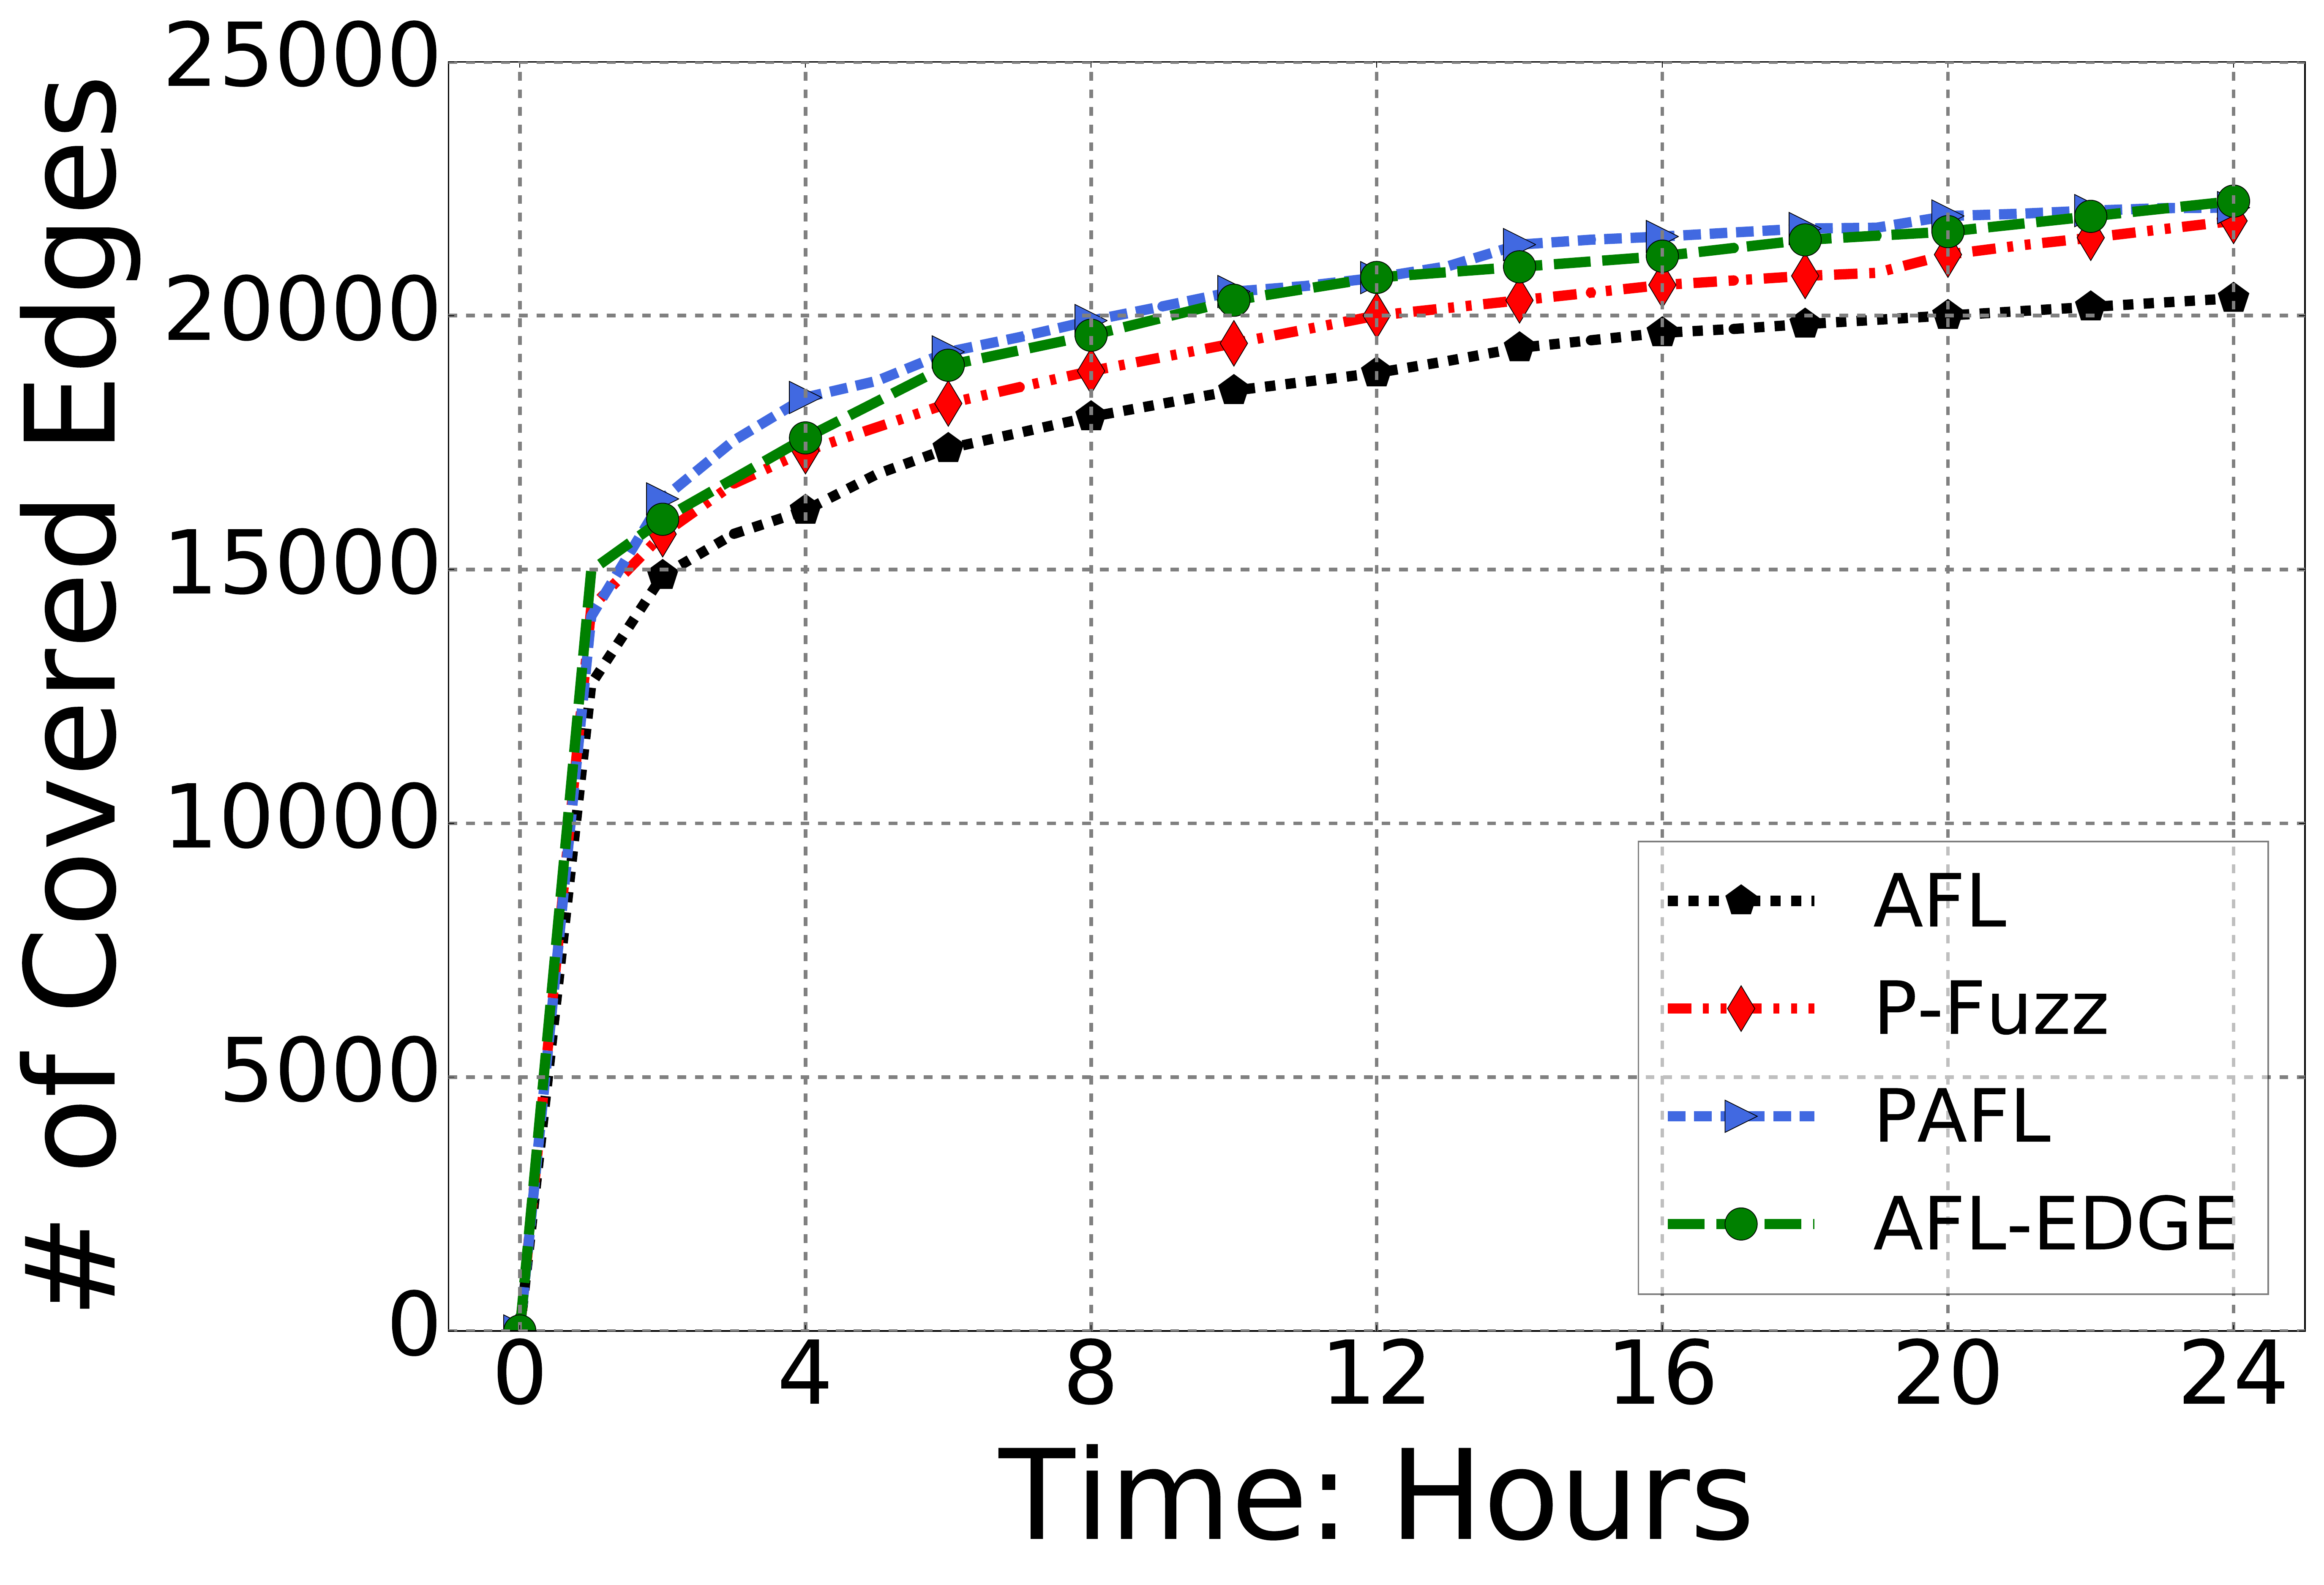} & 
         \includegraphics[scale=0.075]{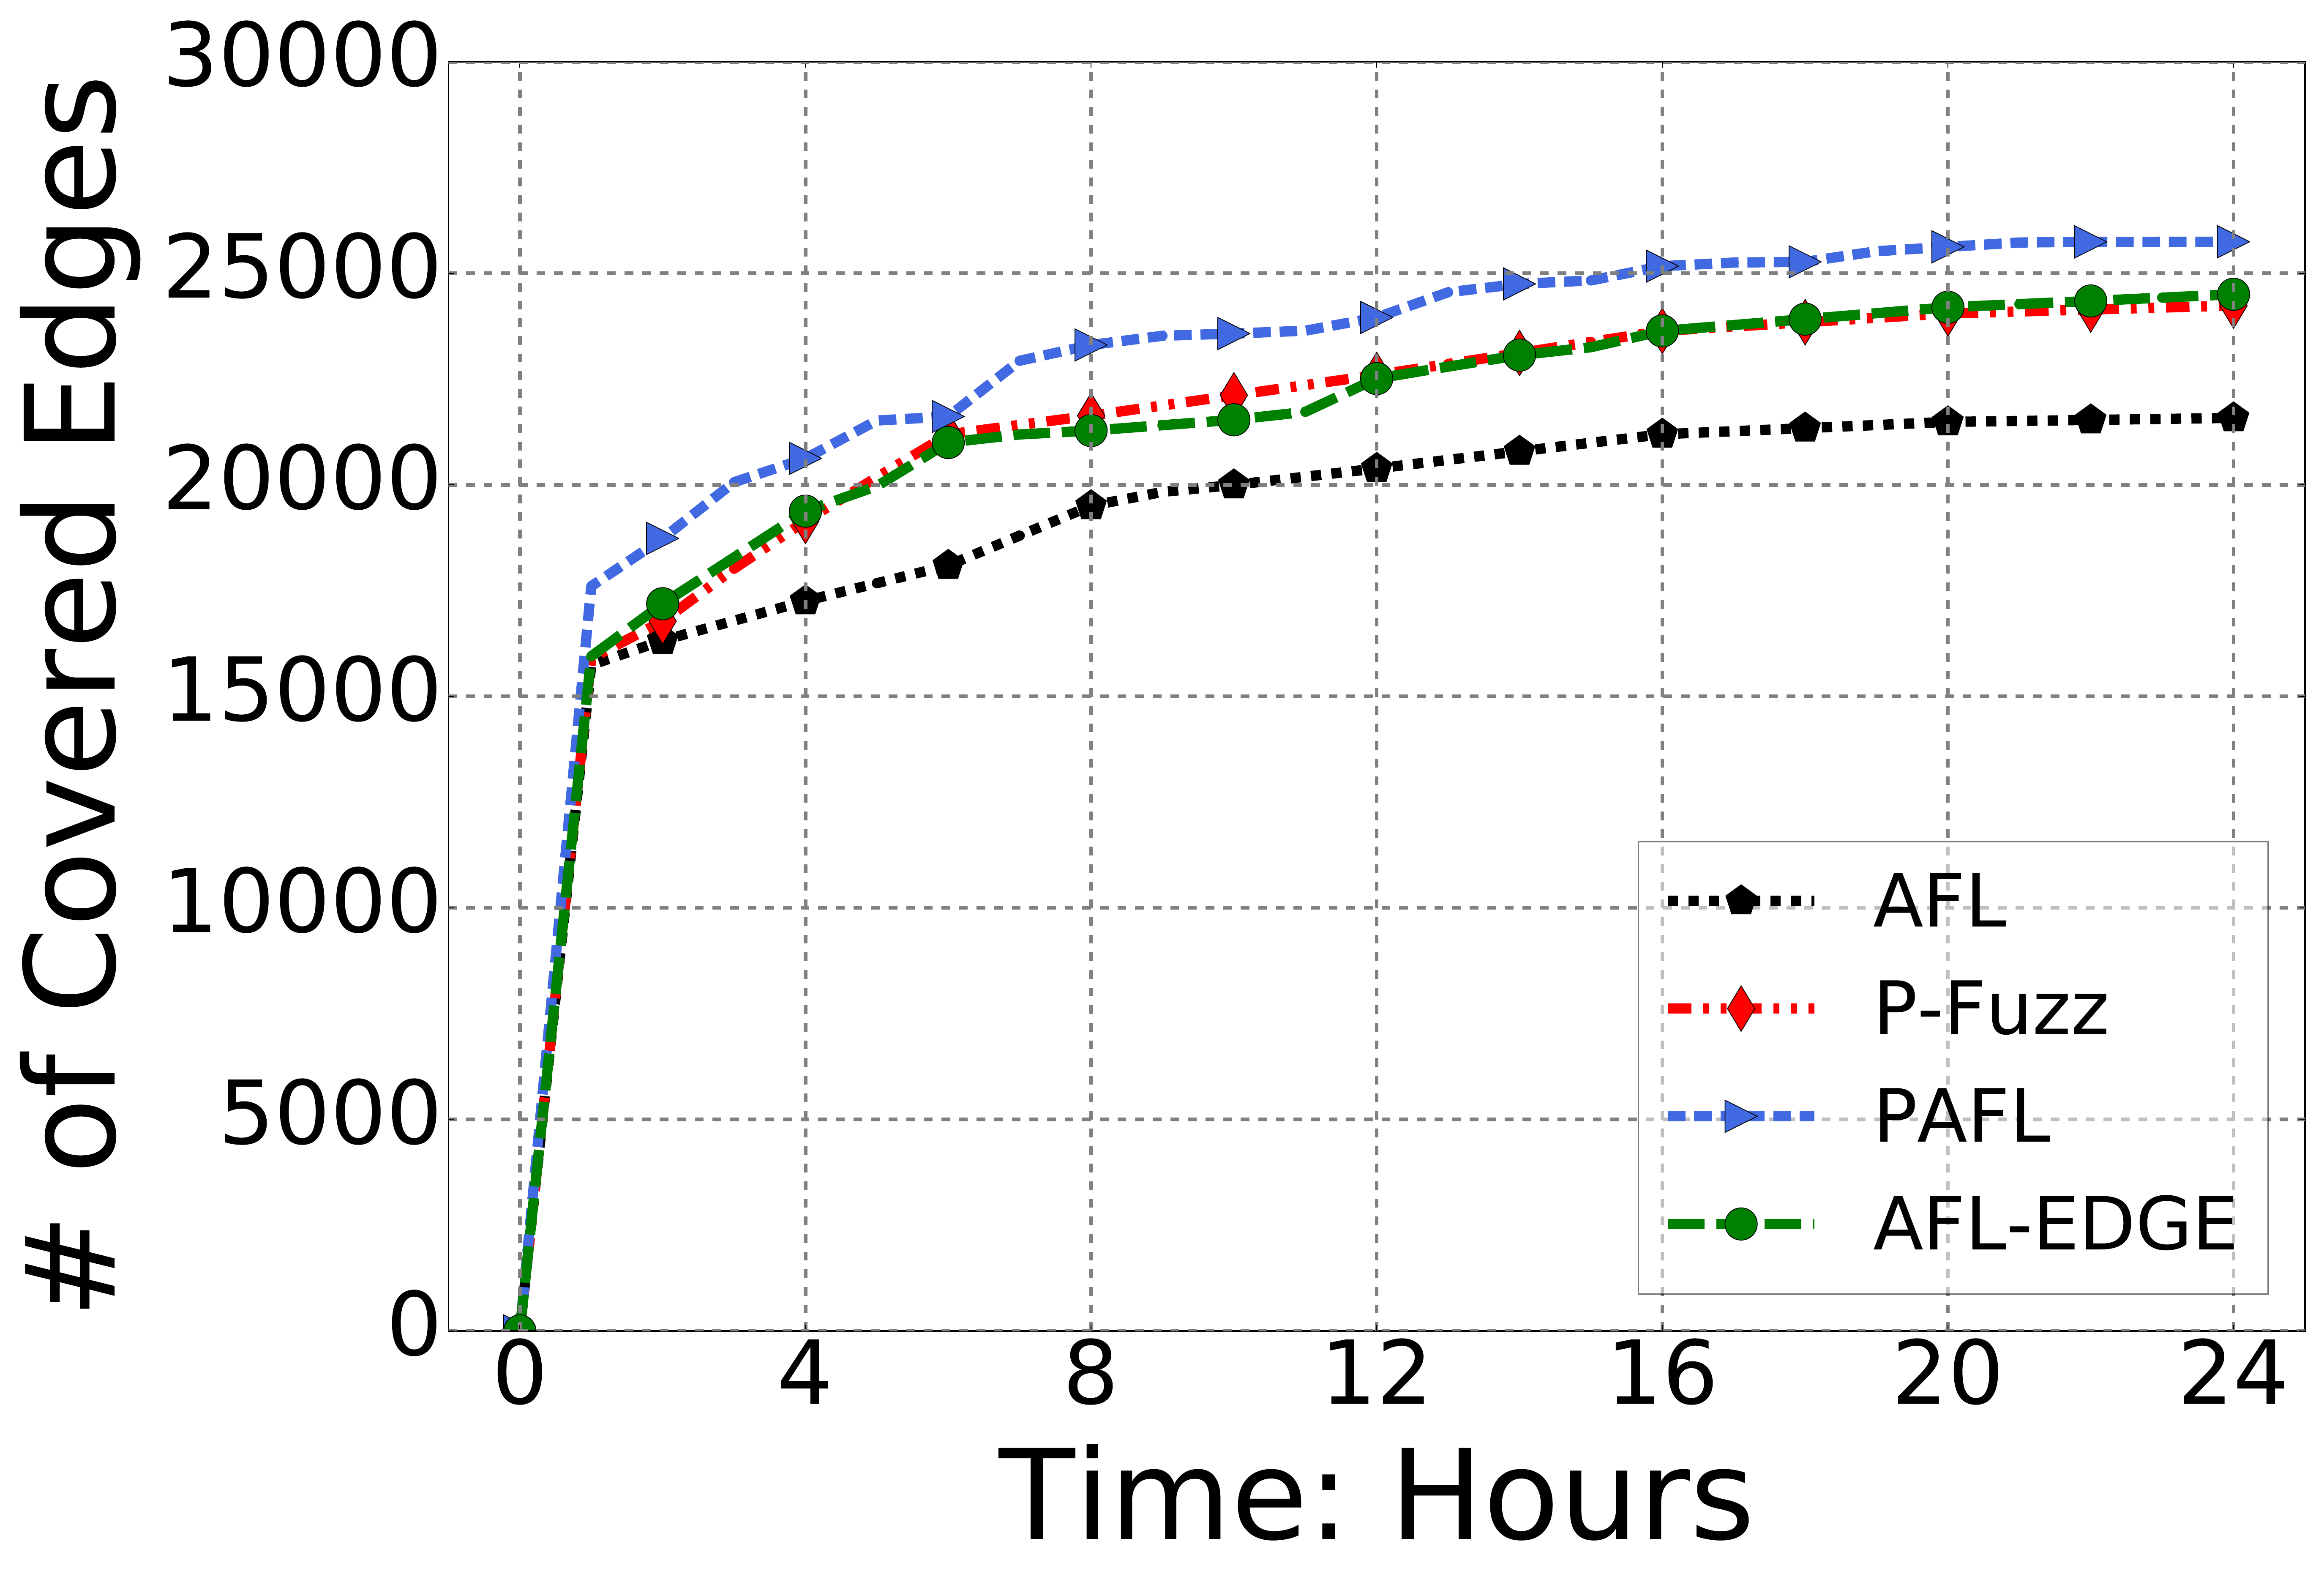} &
         \includegraphics[scale=0.075]{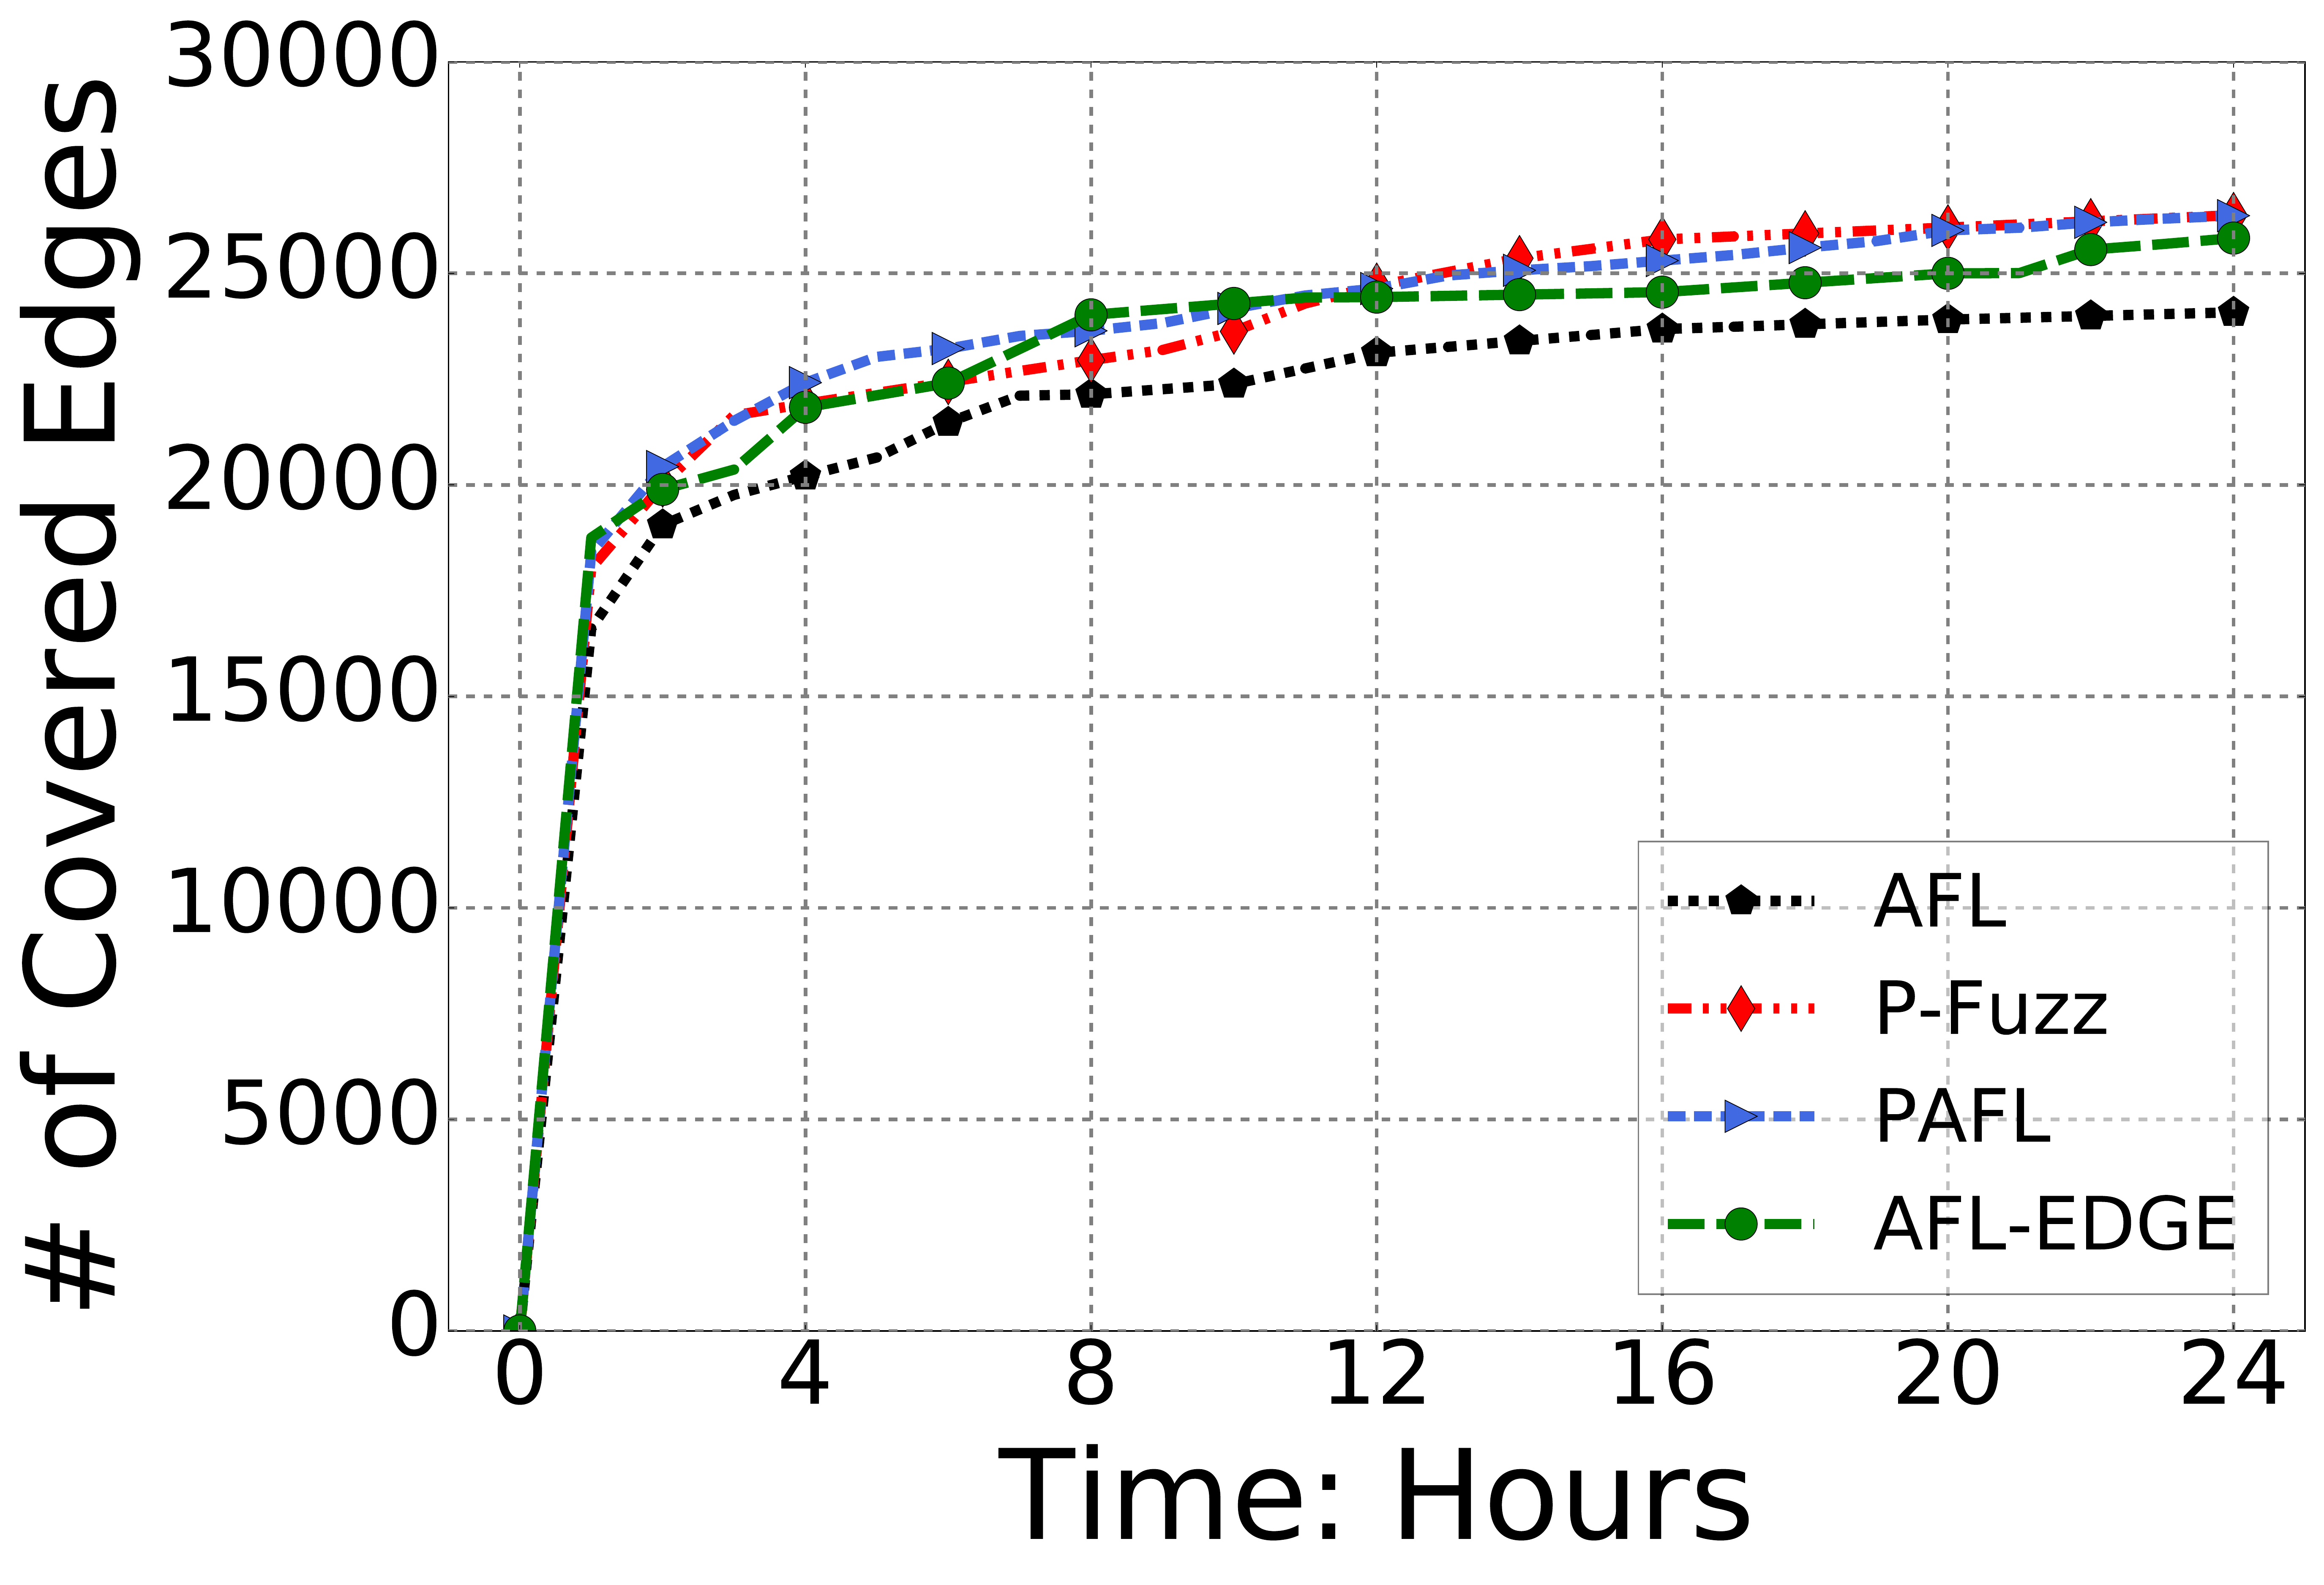} 

         \\
         {\scriptsize\textbf{tiff2ps} \scriptsize 2 instances AFL} &
         {\scriptsize\textbf{tiff2ps} \scriptsize 4 instances AFL} &
         {\scriptsize\textbf{tiff2ps} \scriptsize 8 instances AFL} 
        %  {\scriptsize\textbf{tiff2ps} \scriptsize 2 instance QSYM} &
        %  {\scriptsize\textbf{tiff2ps} \scriptsize 4 instance QSYM} &
        %  {\scriptsize\textbf{tiff2ps} \scriptsize 8 instance QSYM} \\
         \\
         
         \includegraphics[scale=0.075]{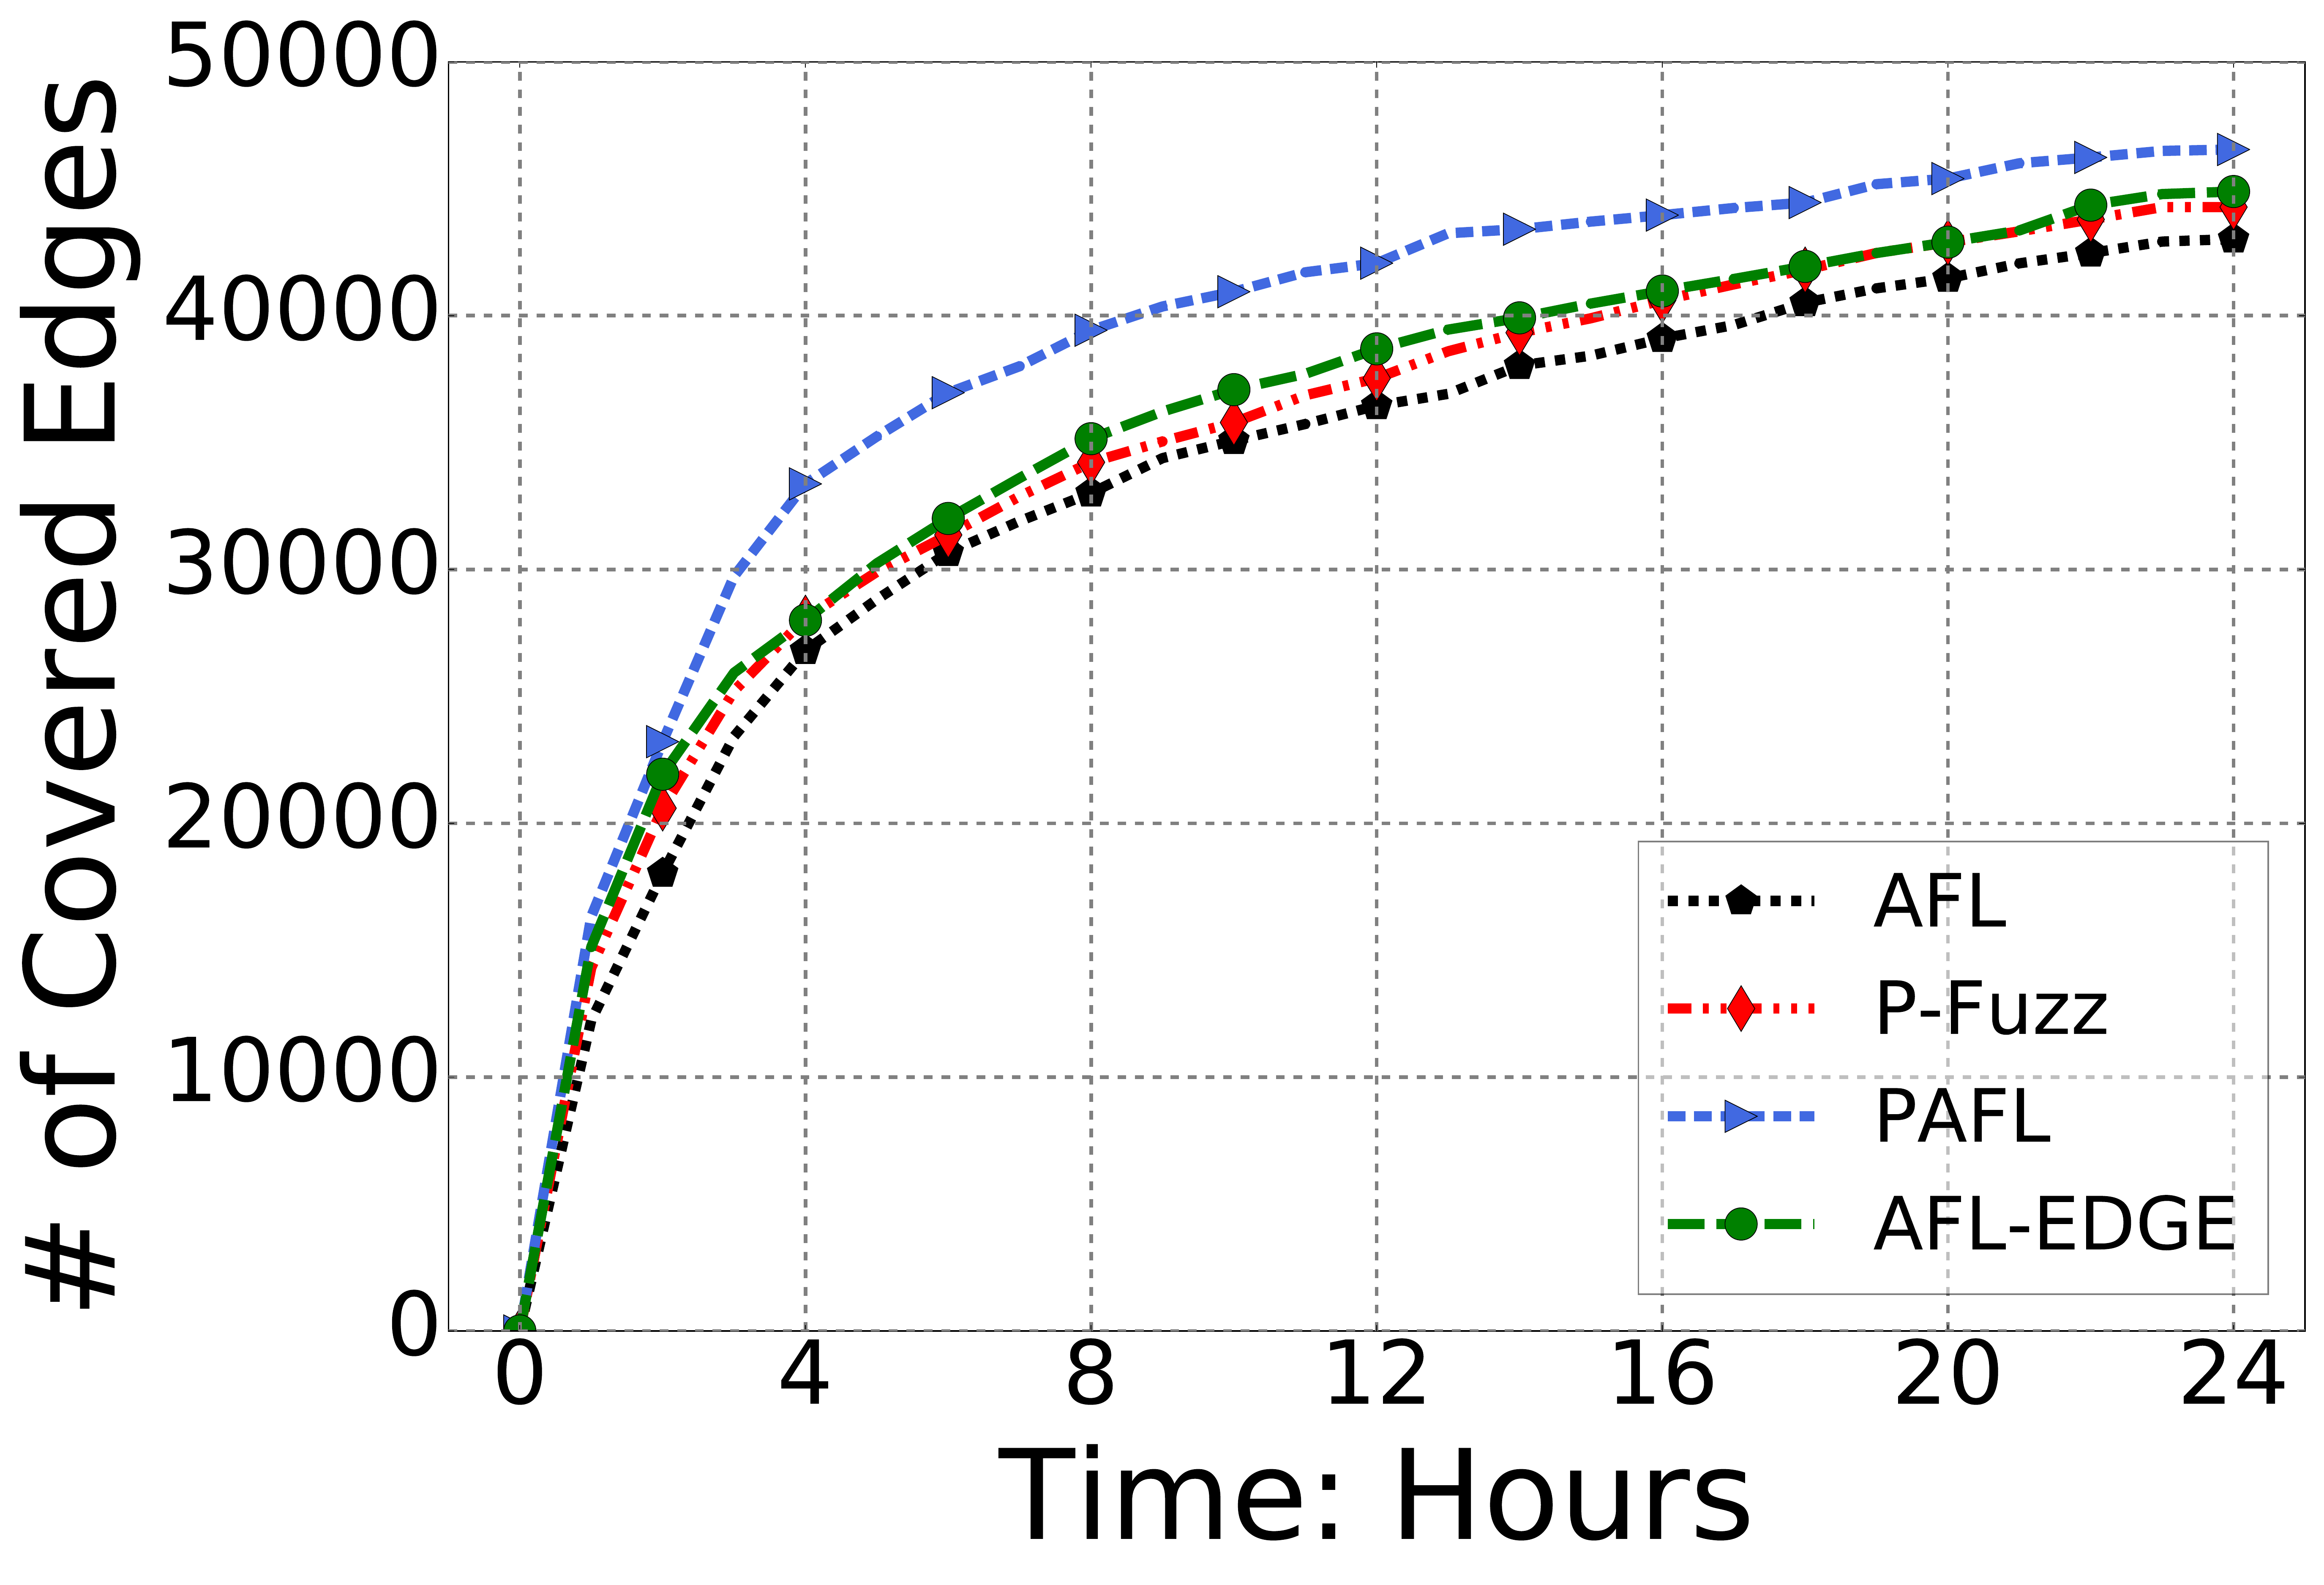} & 
         \includegraphics[scale=0.075]{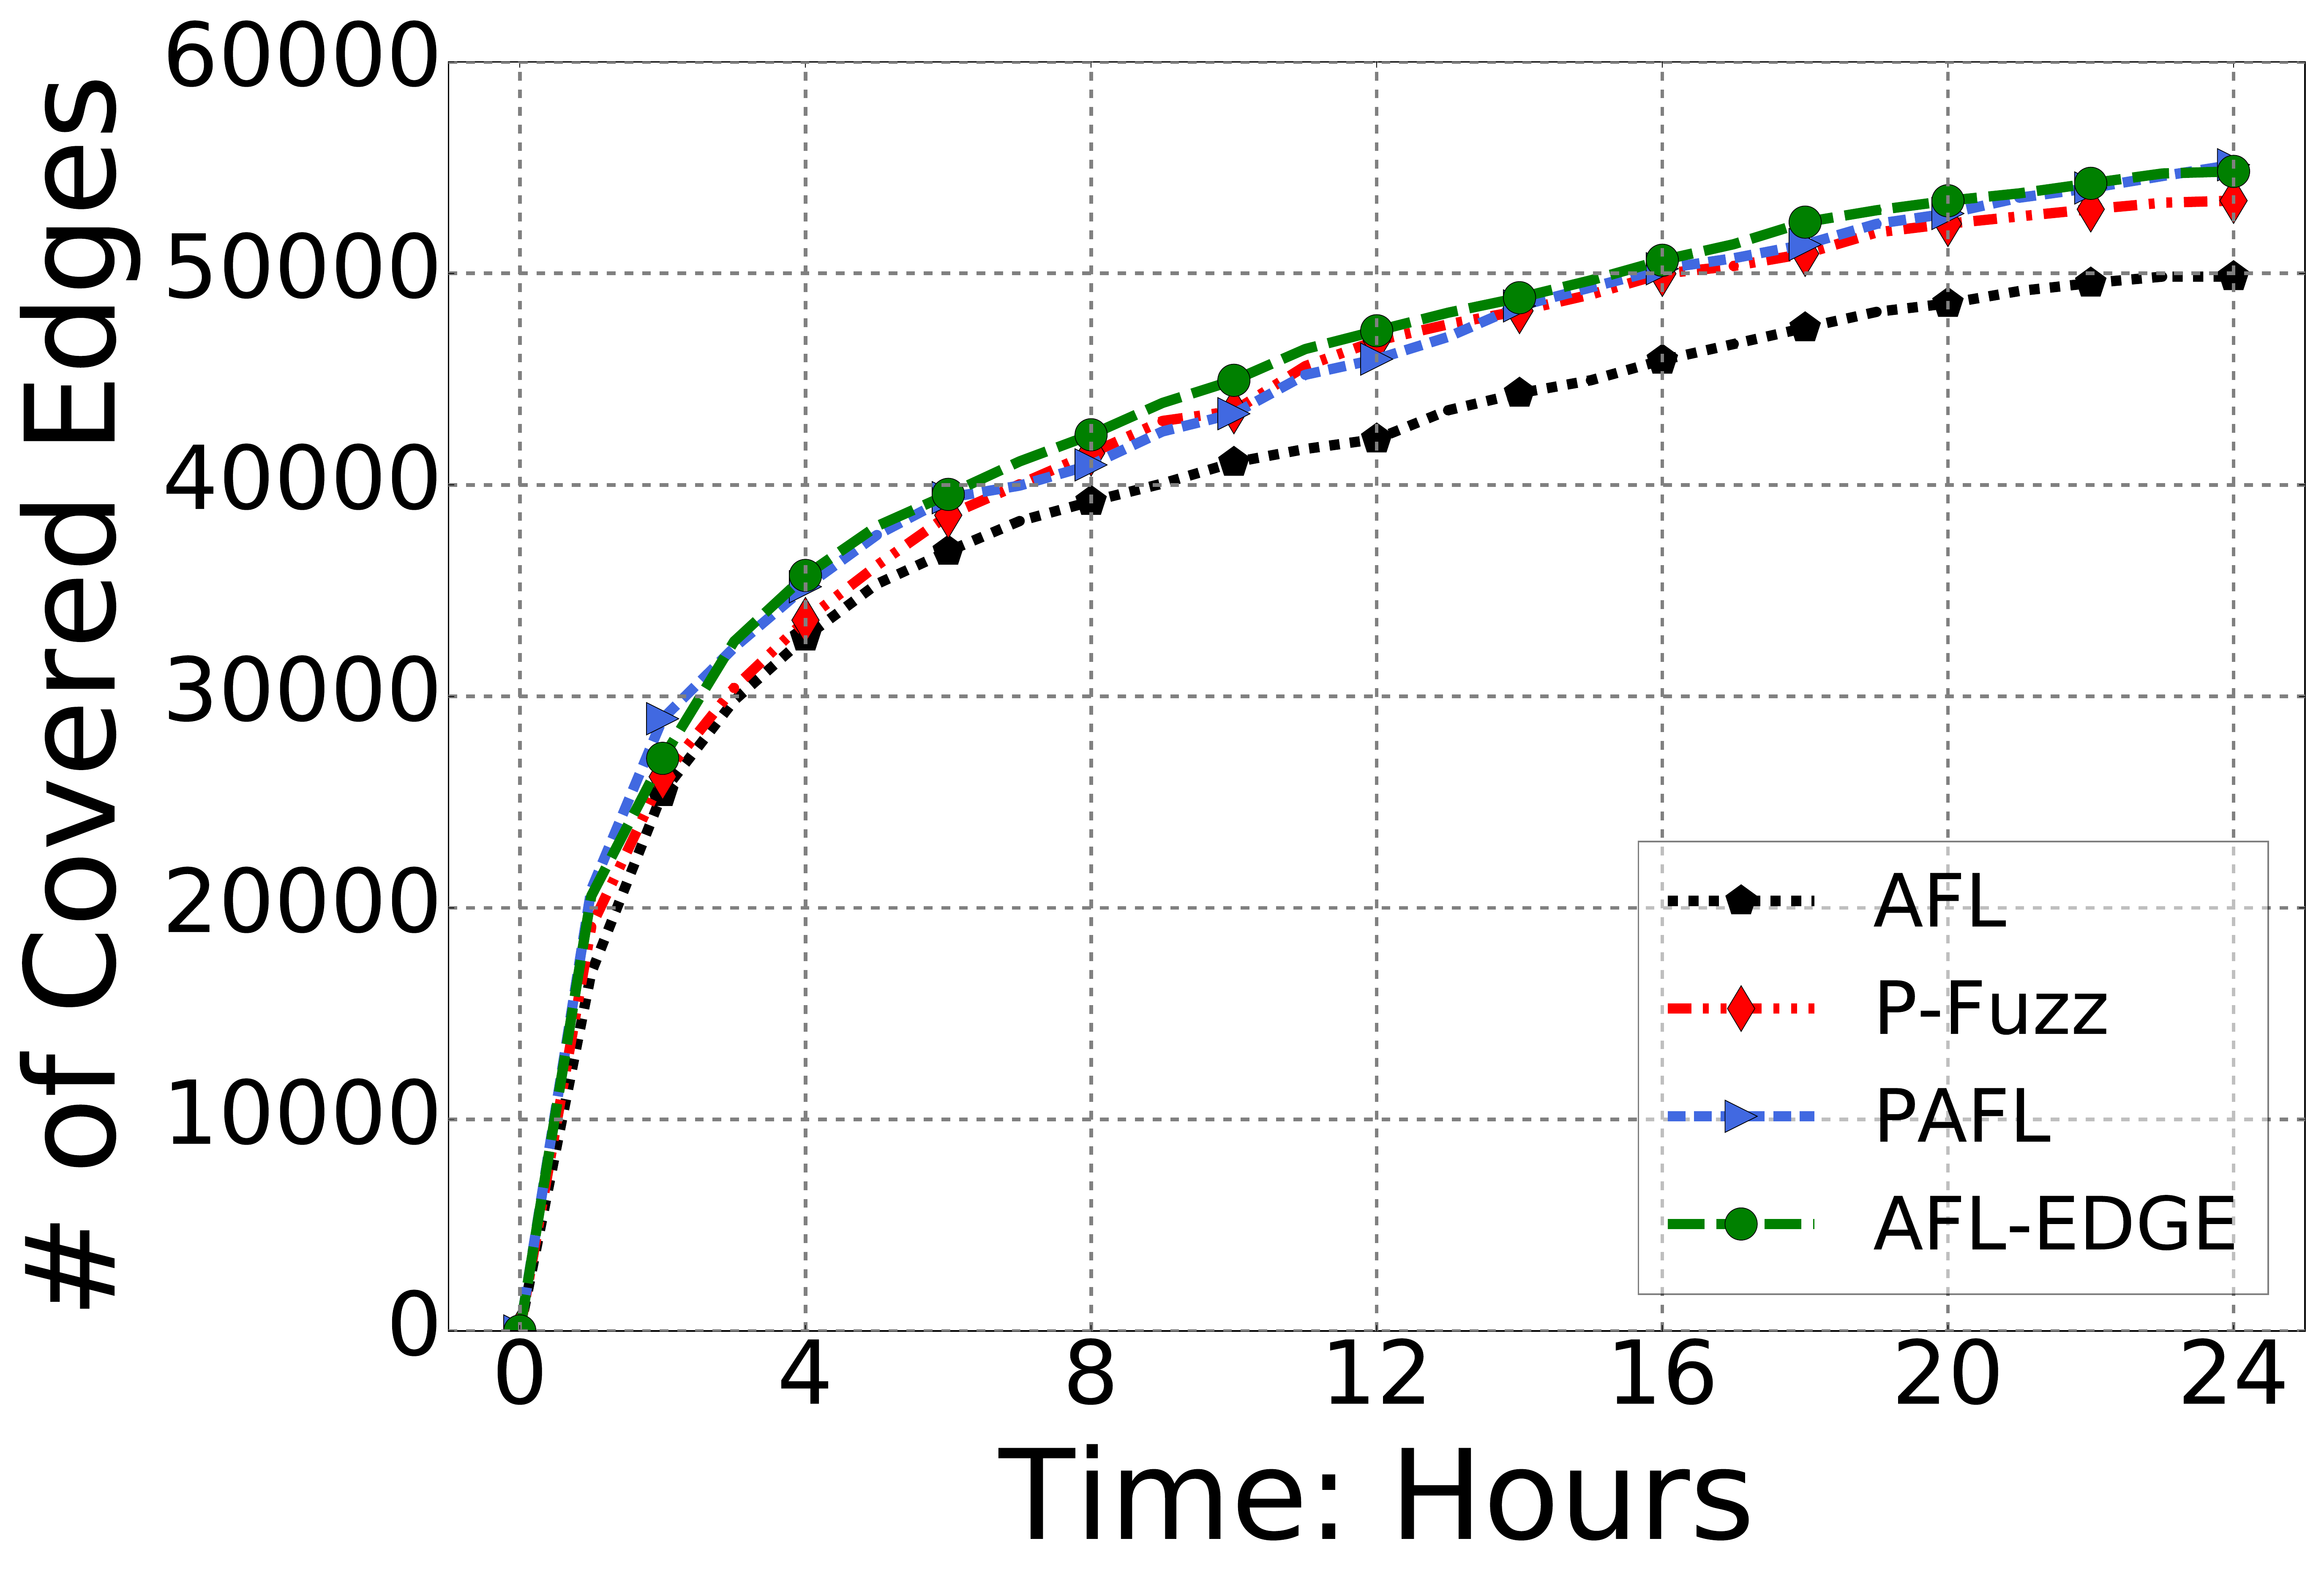} &
         \includegraphics[scale=0.075]{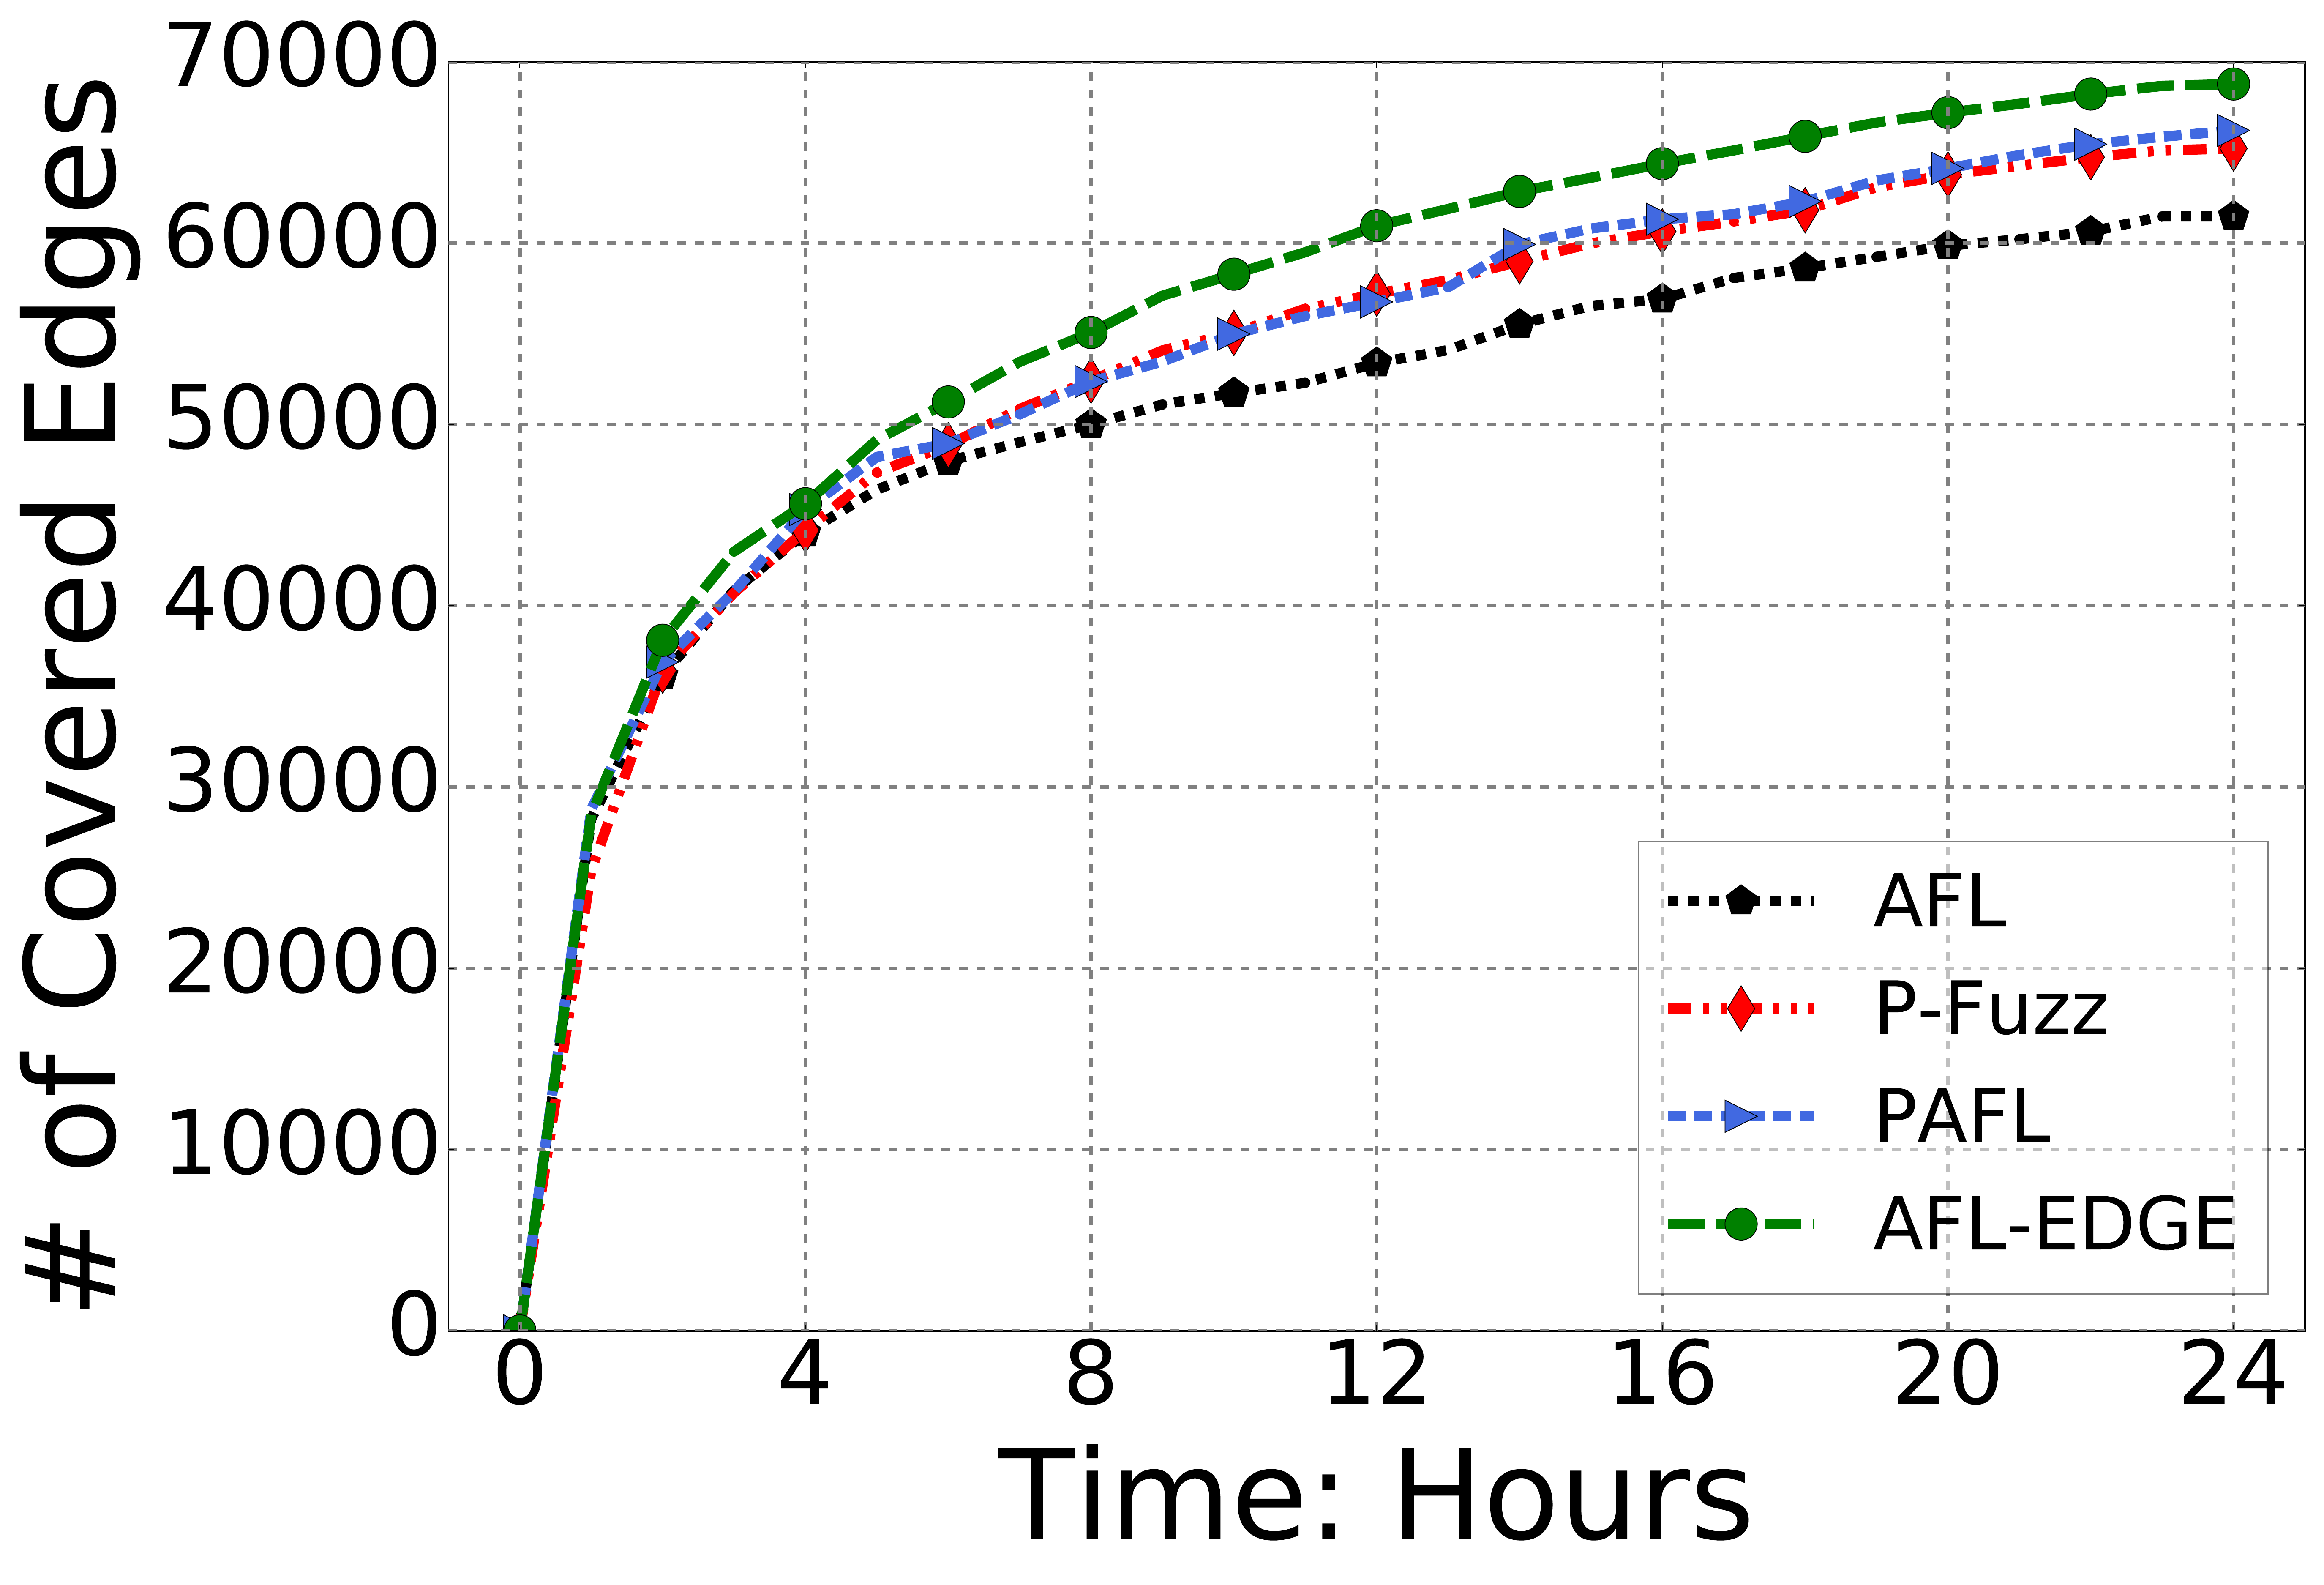}  
         \\
         {\scriptsize\textbf{tcpdump} \scriptsize 2 instances AFL} &
         {\scriptsize\textbf{tcpdump} \scriptsize 4 instances AFL} &
         {\scriptsize\textbf{tcpdump} \scriptsize 8 instances AFL} 
        %  {\scriptsize\textbf{tcpdump} \scriptsize 2 instance QSYM} &
        %  {\scriptsize\textbf{tcpdump} \scriptsize 4 instance QSYM} &
        %  {\scriptsize\textbf{tcpdump} \scriptsize 8 instance QSYM} \\
         \\
         \includegraphics[scale=0.075]{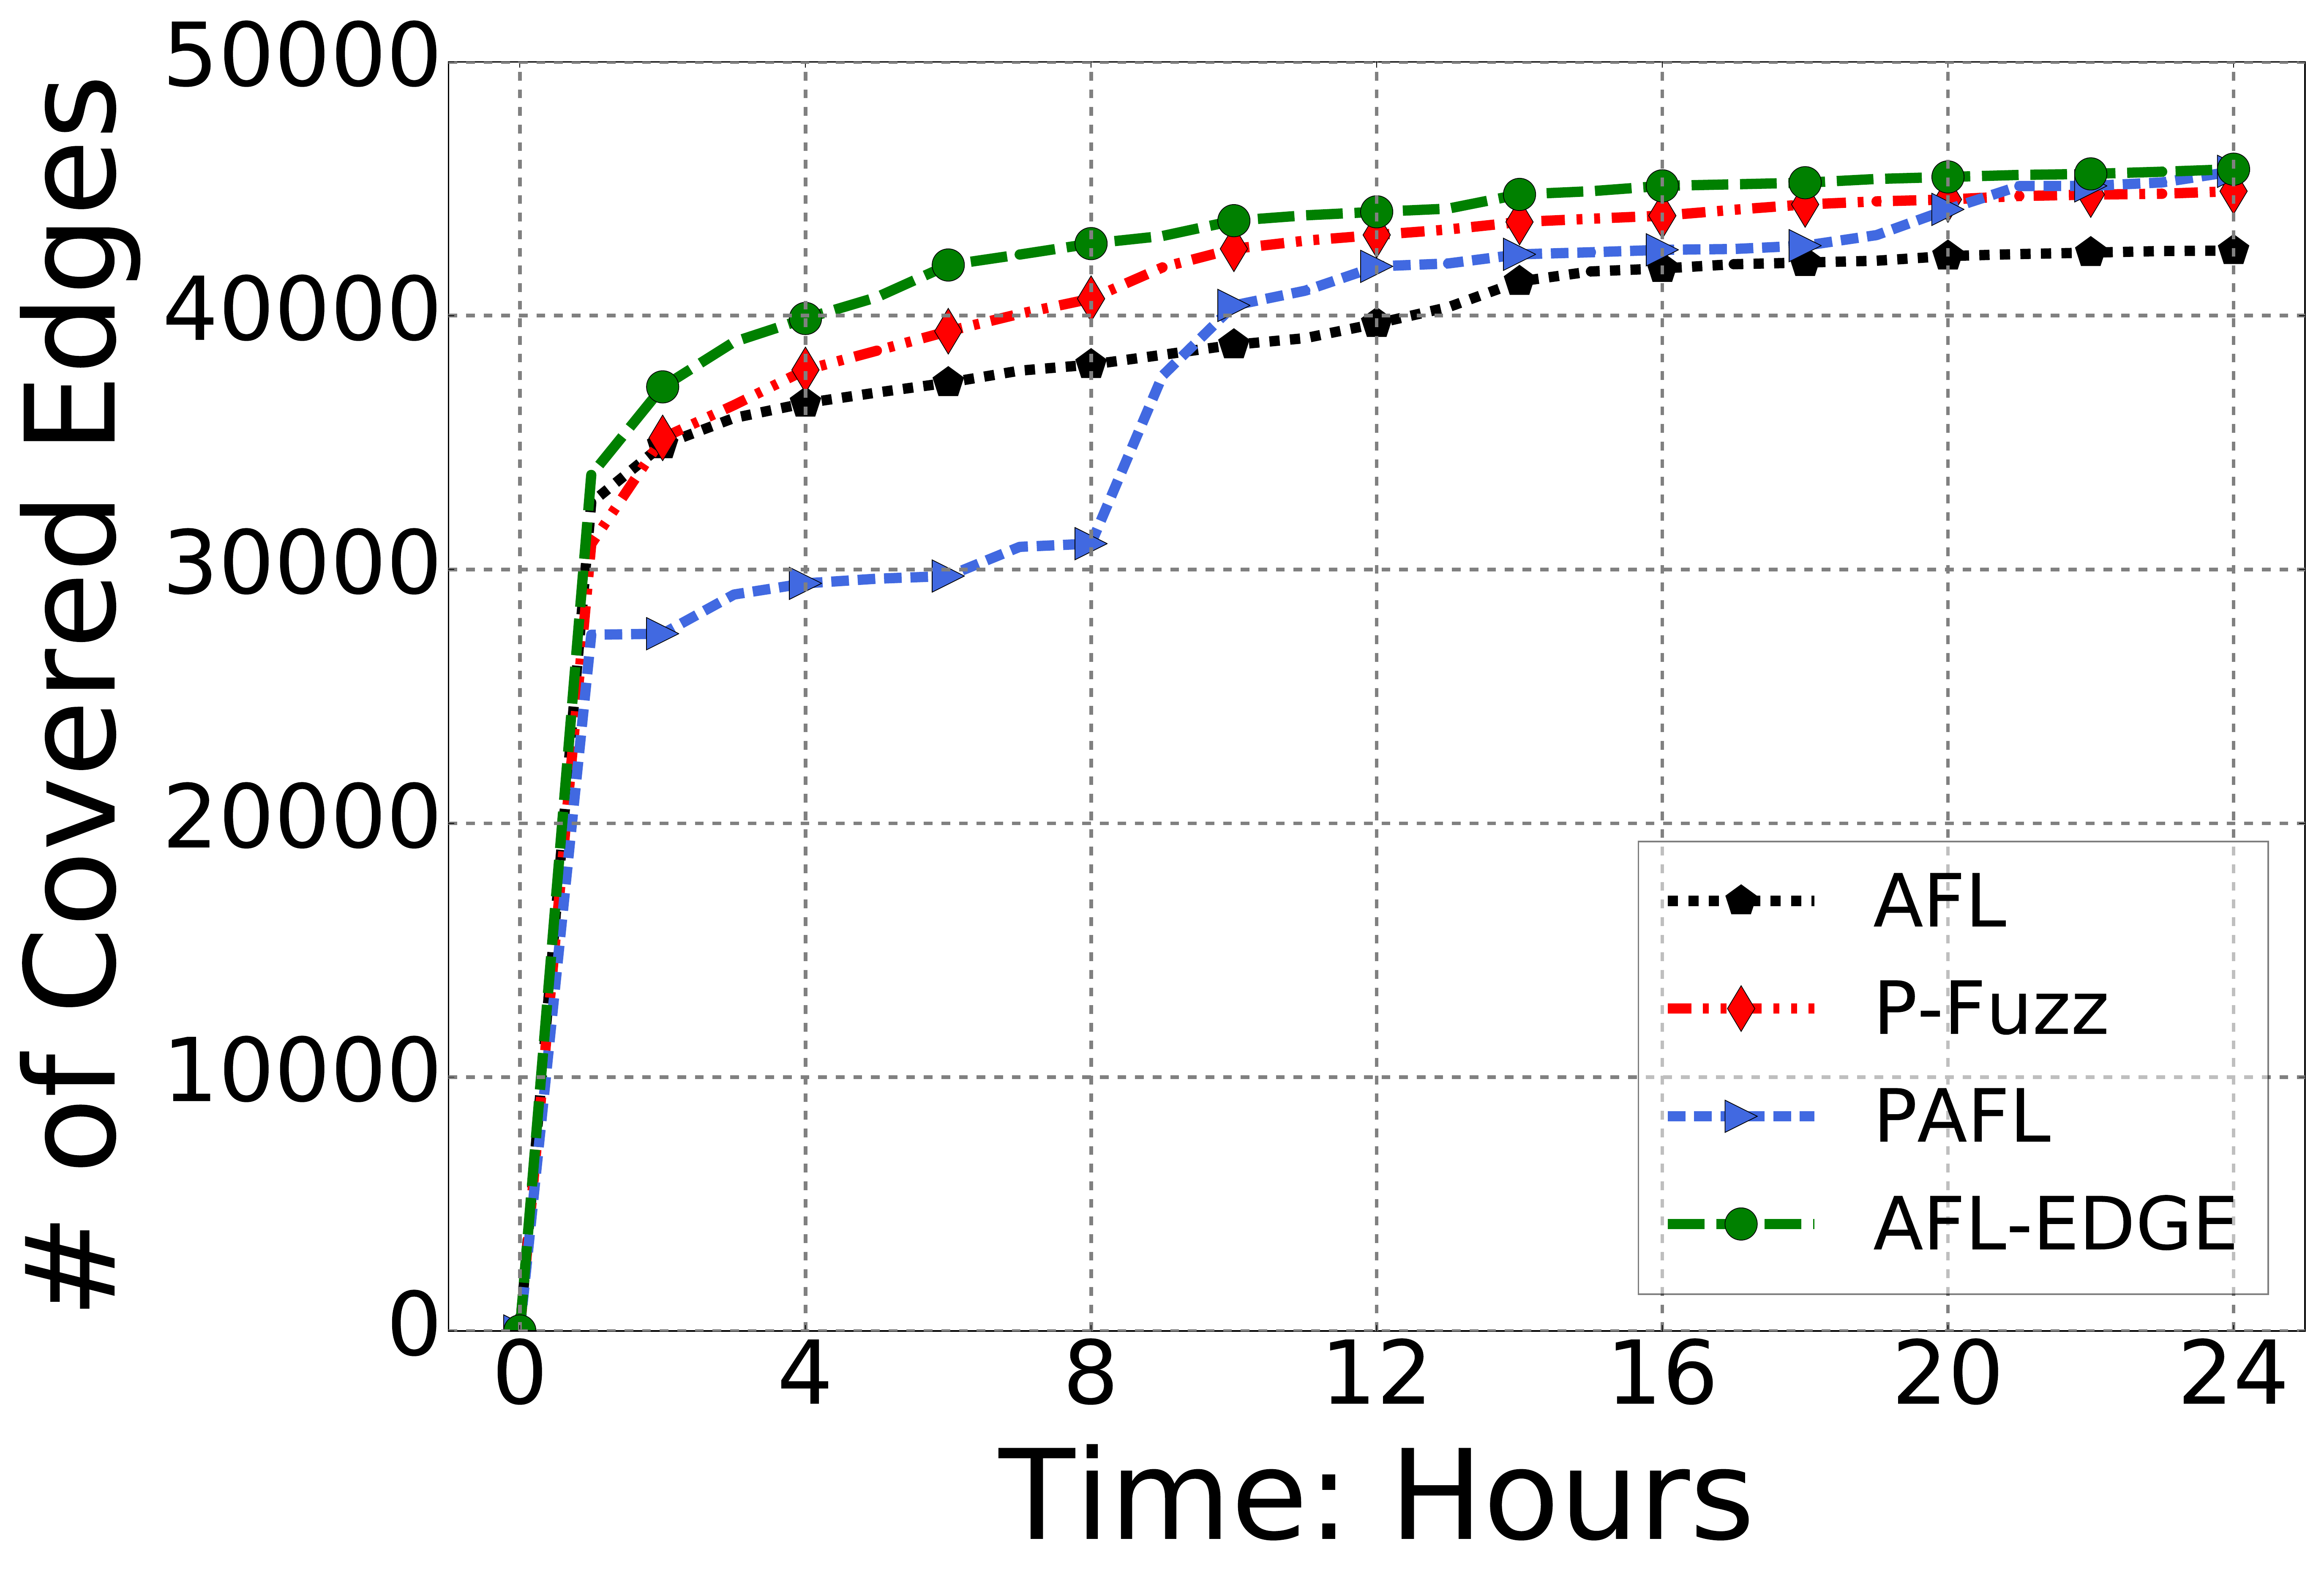} & 
         \includegraphics[scale=0.075]{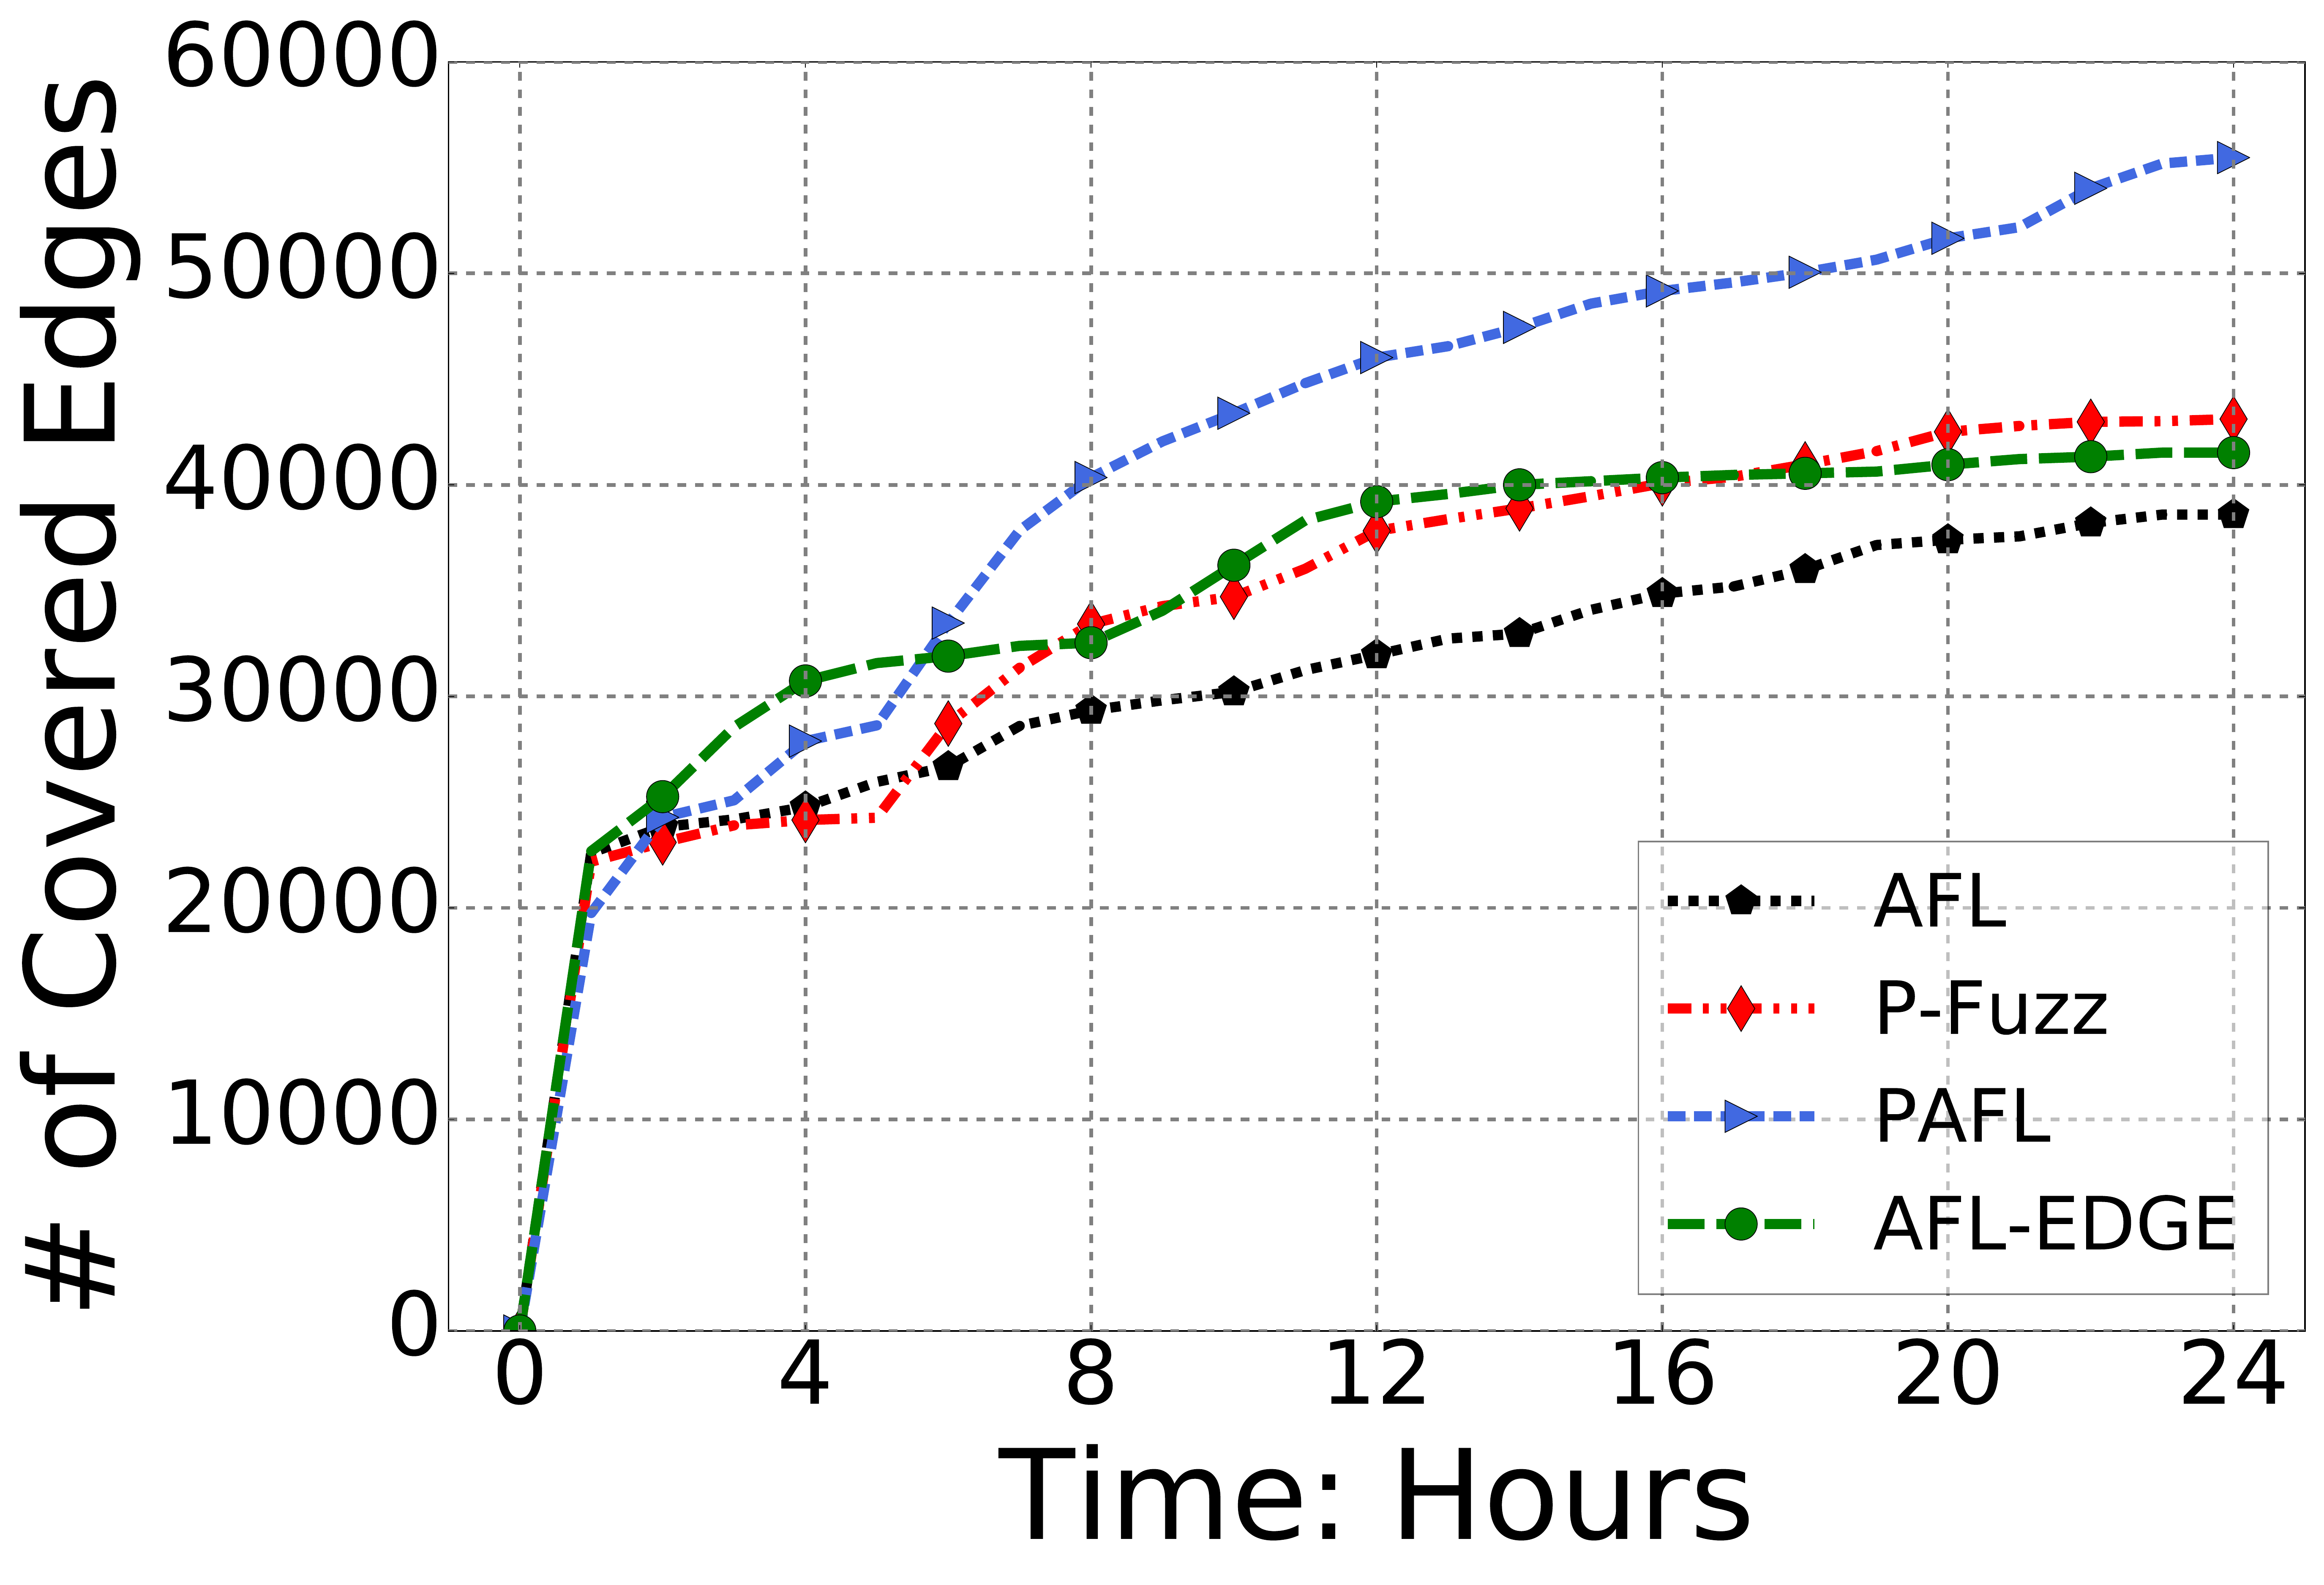} &
         \includegraphics[scale=0.075]{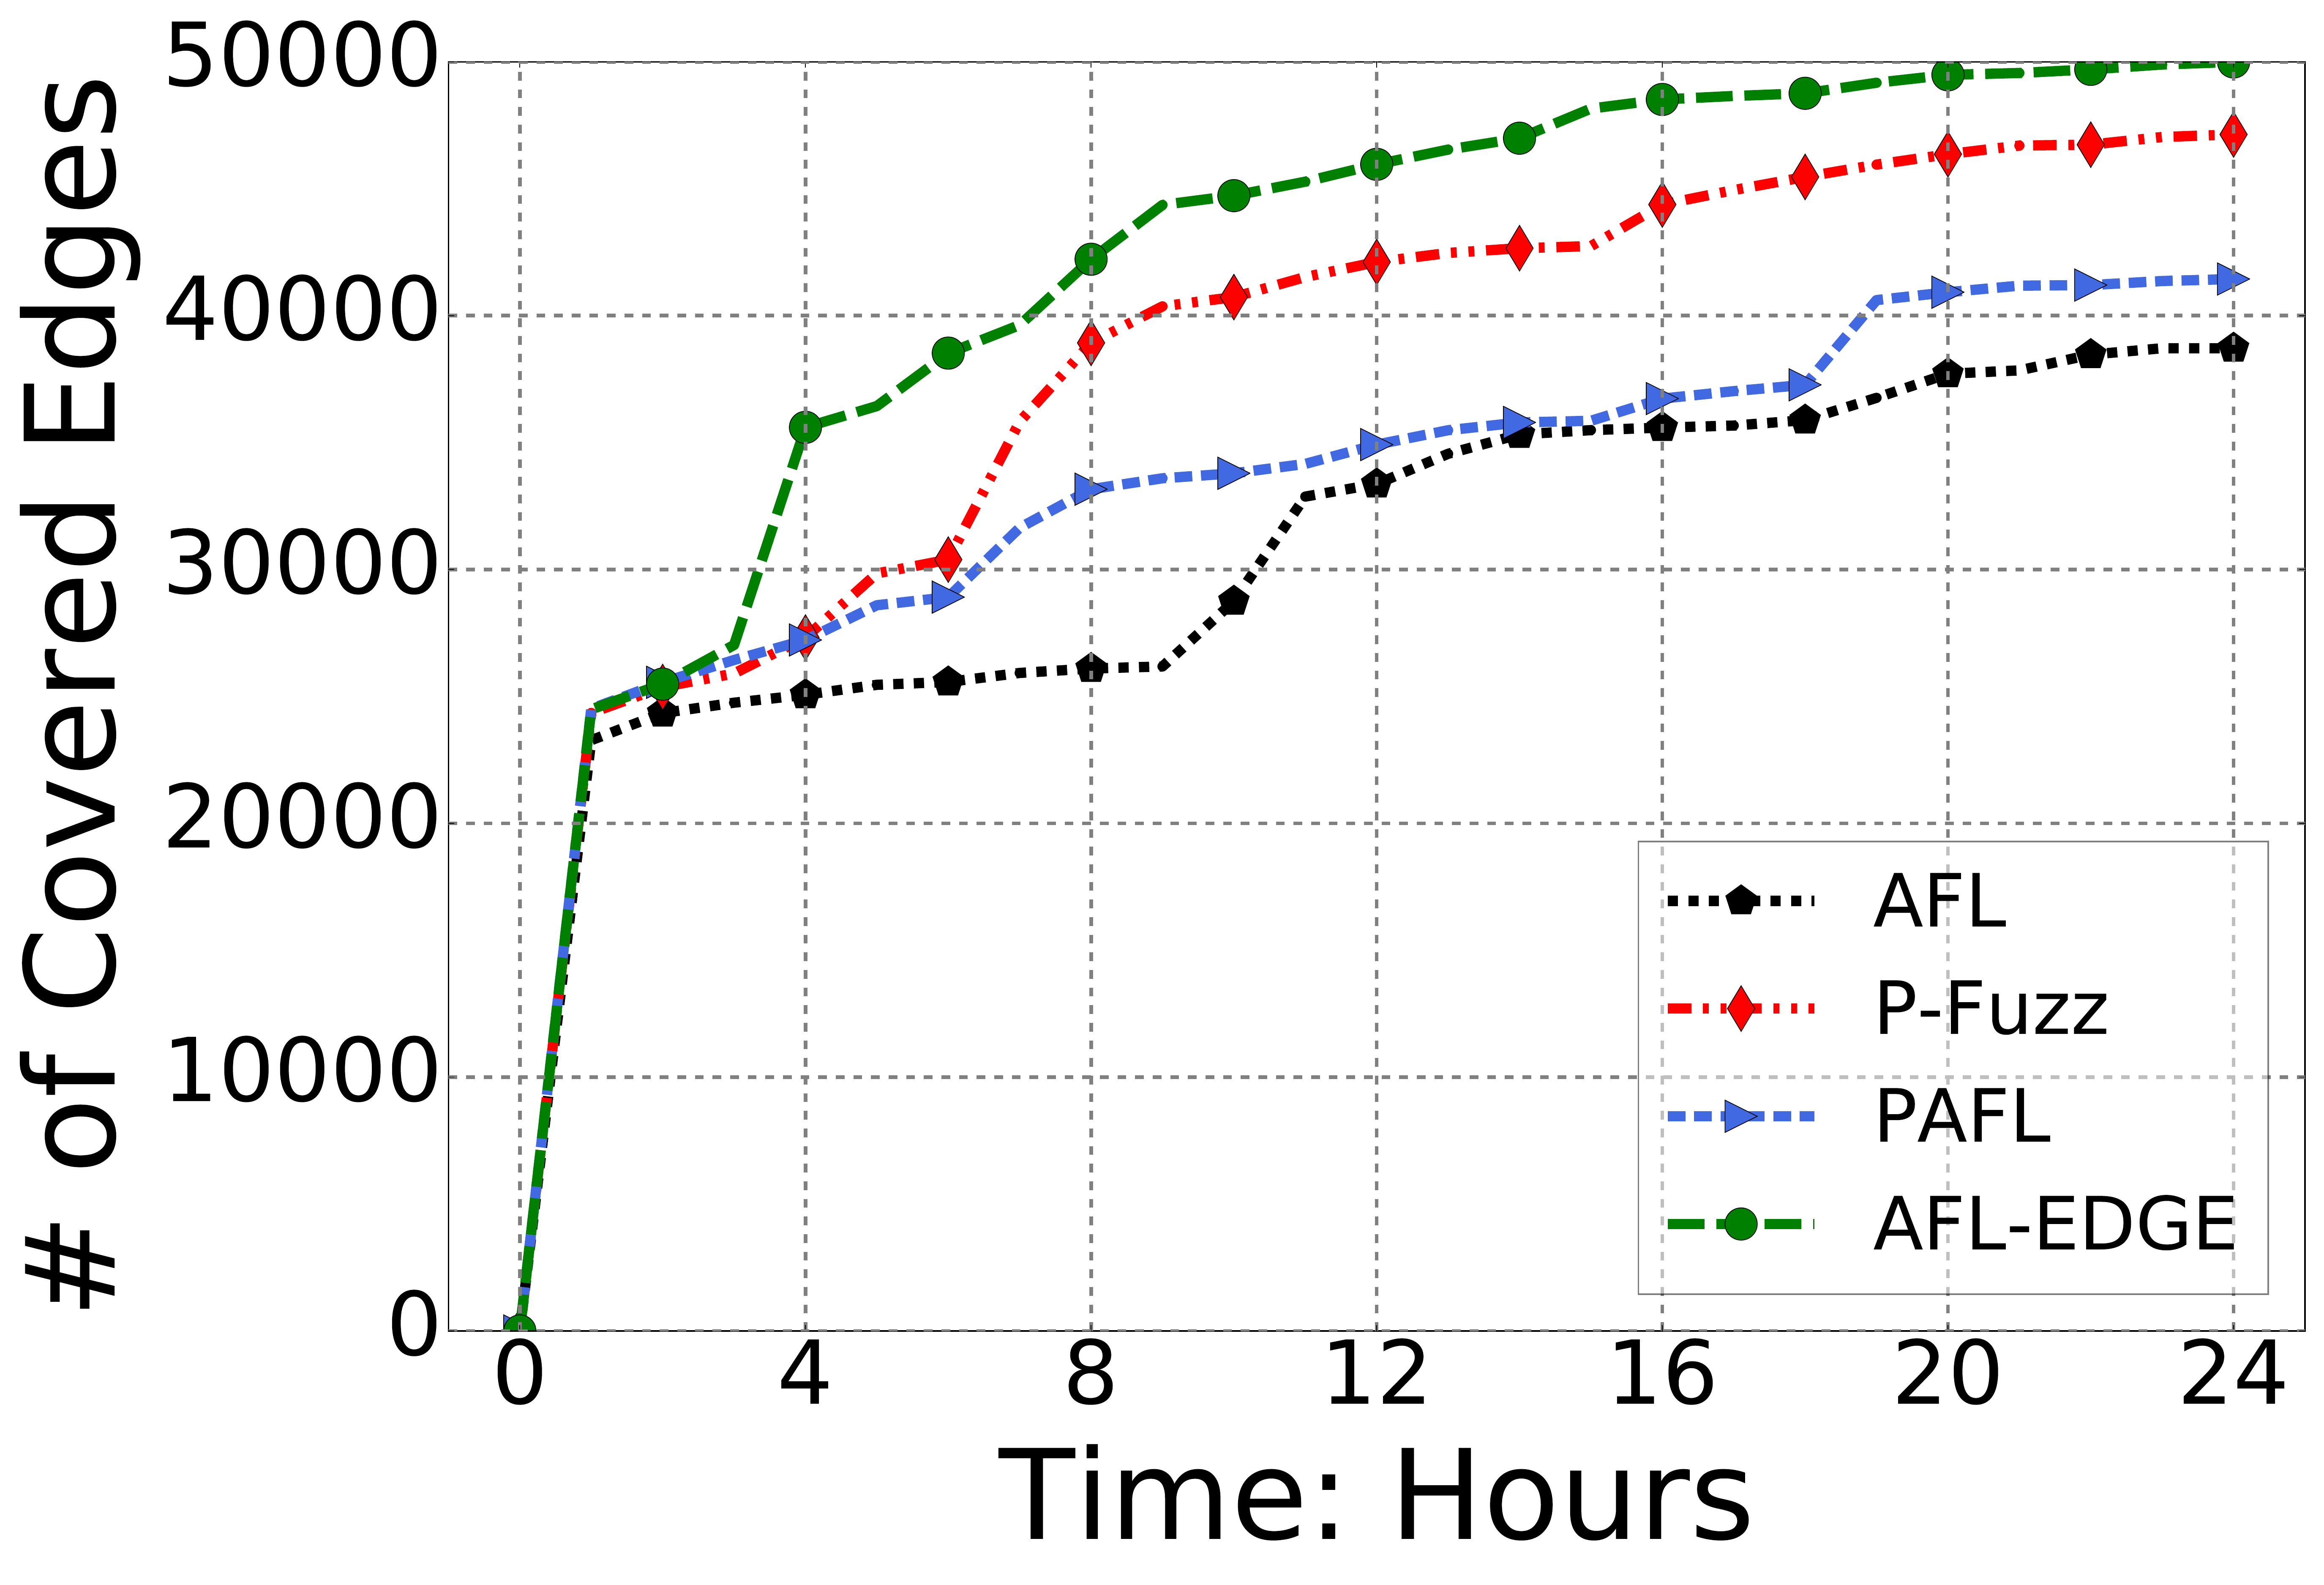} 
         \\
         {\scriptsize\textbf{libxml} \scriptsize 2 instances AFL} &
         {\scriptsize\textbf{libxml} \scriptsize 4 instances AFL} &
         {\scriptsize\textbf{libxml} \scriptsize 8 instances AFL}
        %  {\scriptsize\textbf{libxml} \scriptsize 2 instance QSYM} &
        %  {\scriptsize\textbf{libxml} \scriptsize 4 instance QSYM} &
        %  {\scriptsize\textbf{libxml} \scriptsize 8 instance QSYM} \\
         \\
         \includegraphics[scale=0.075]{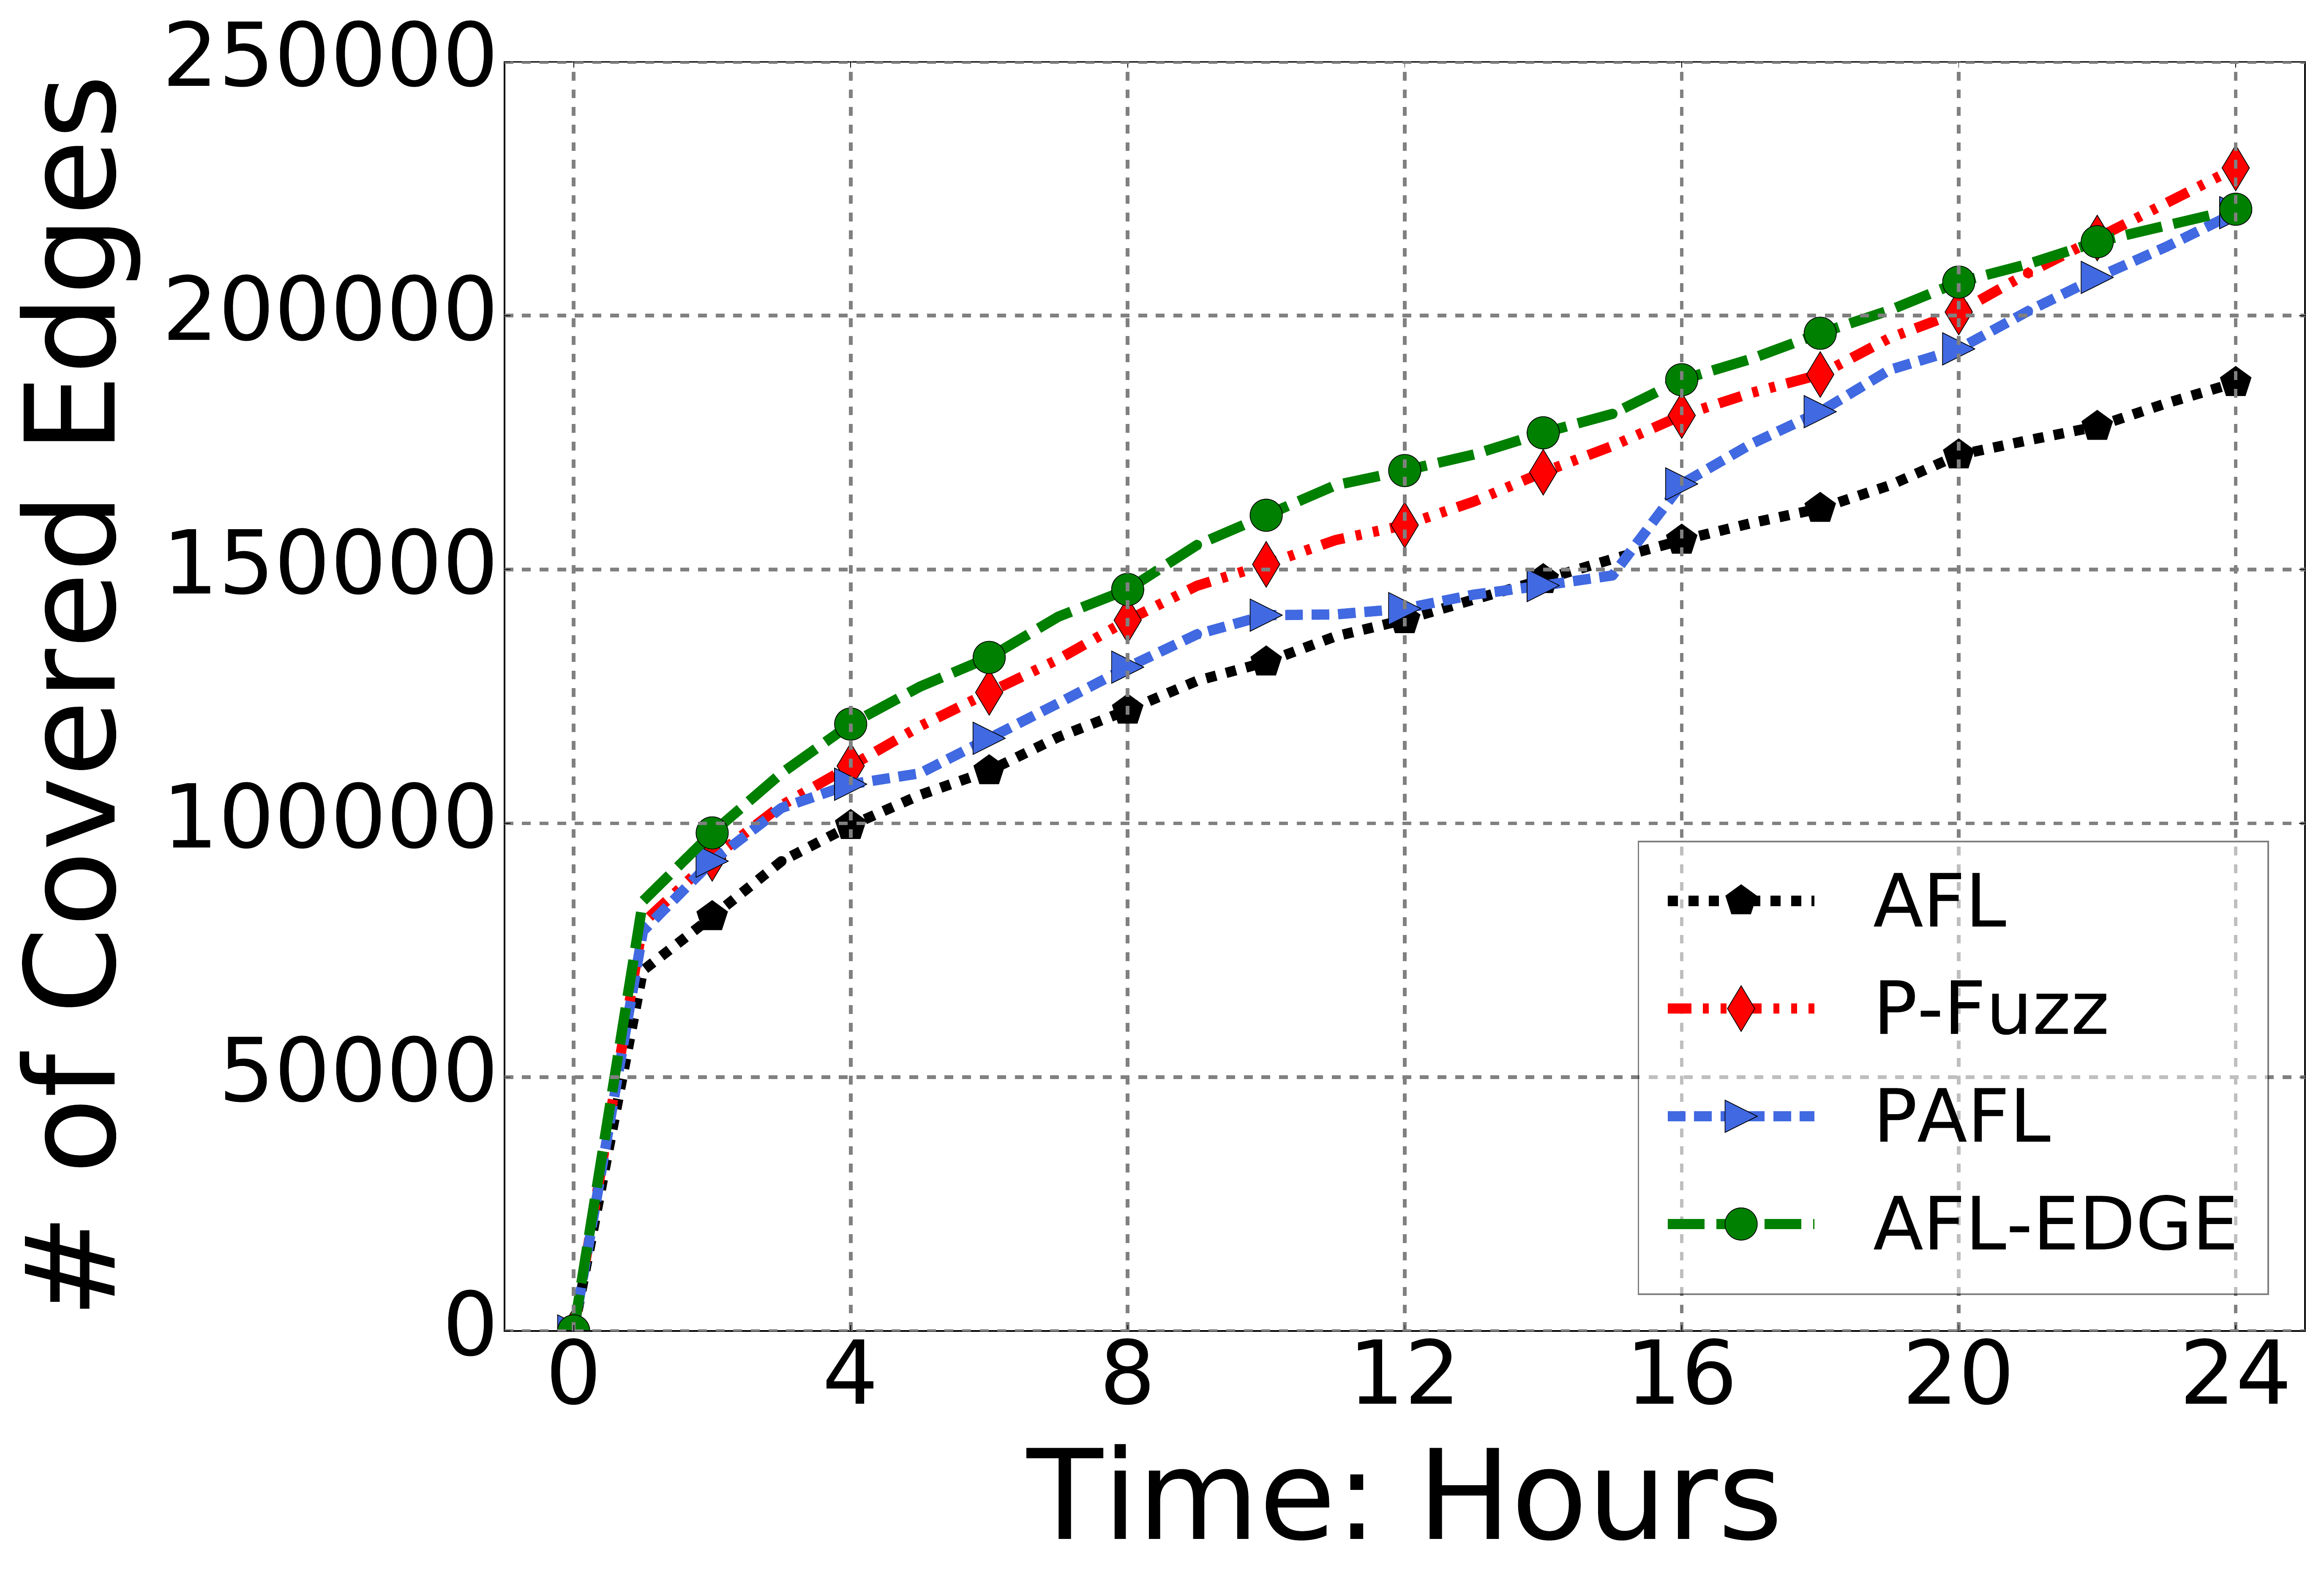} & 
         \includegraphics[scale=0.075]{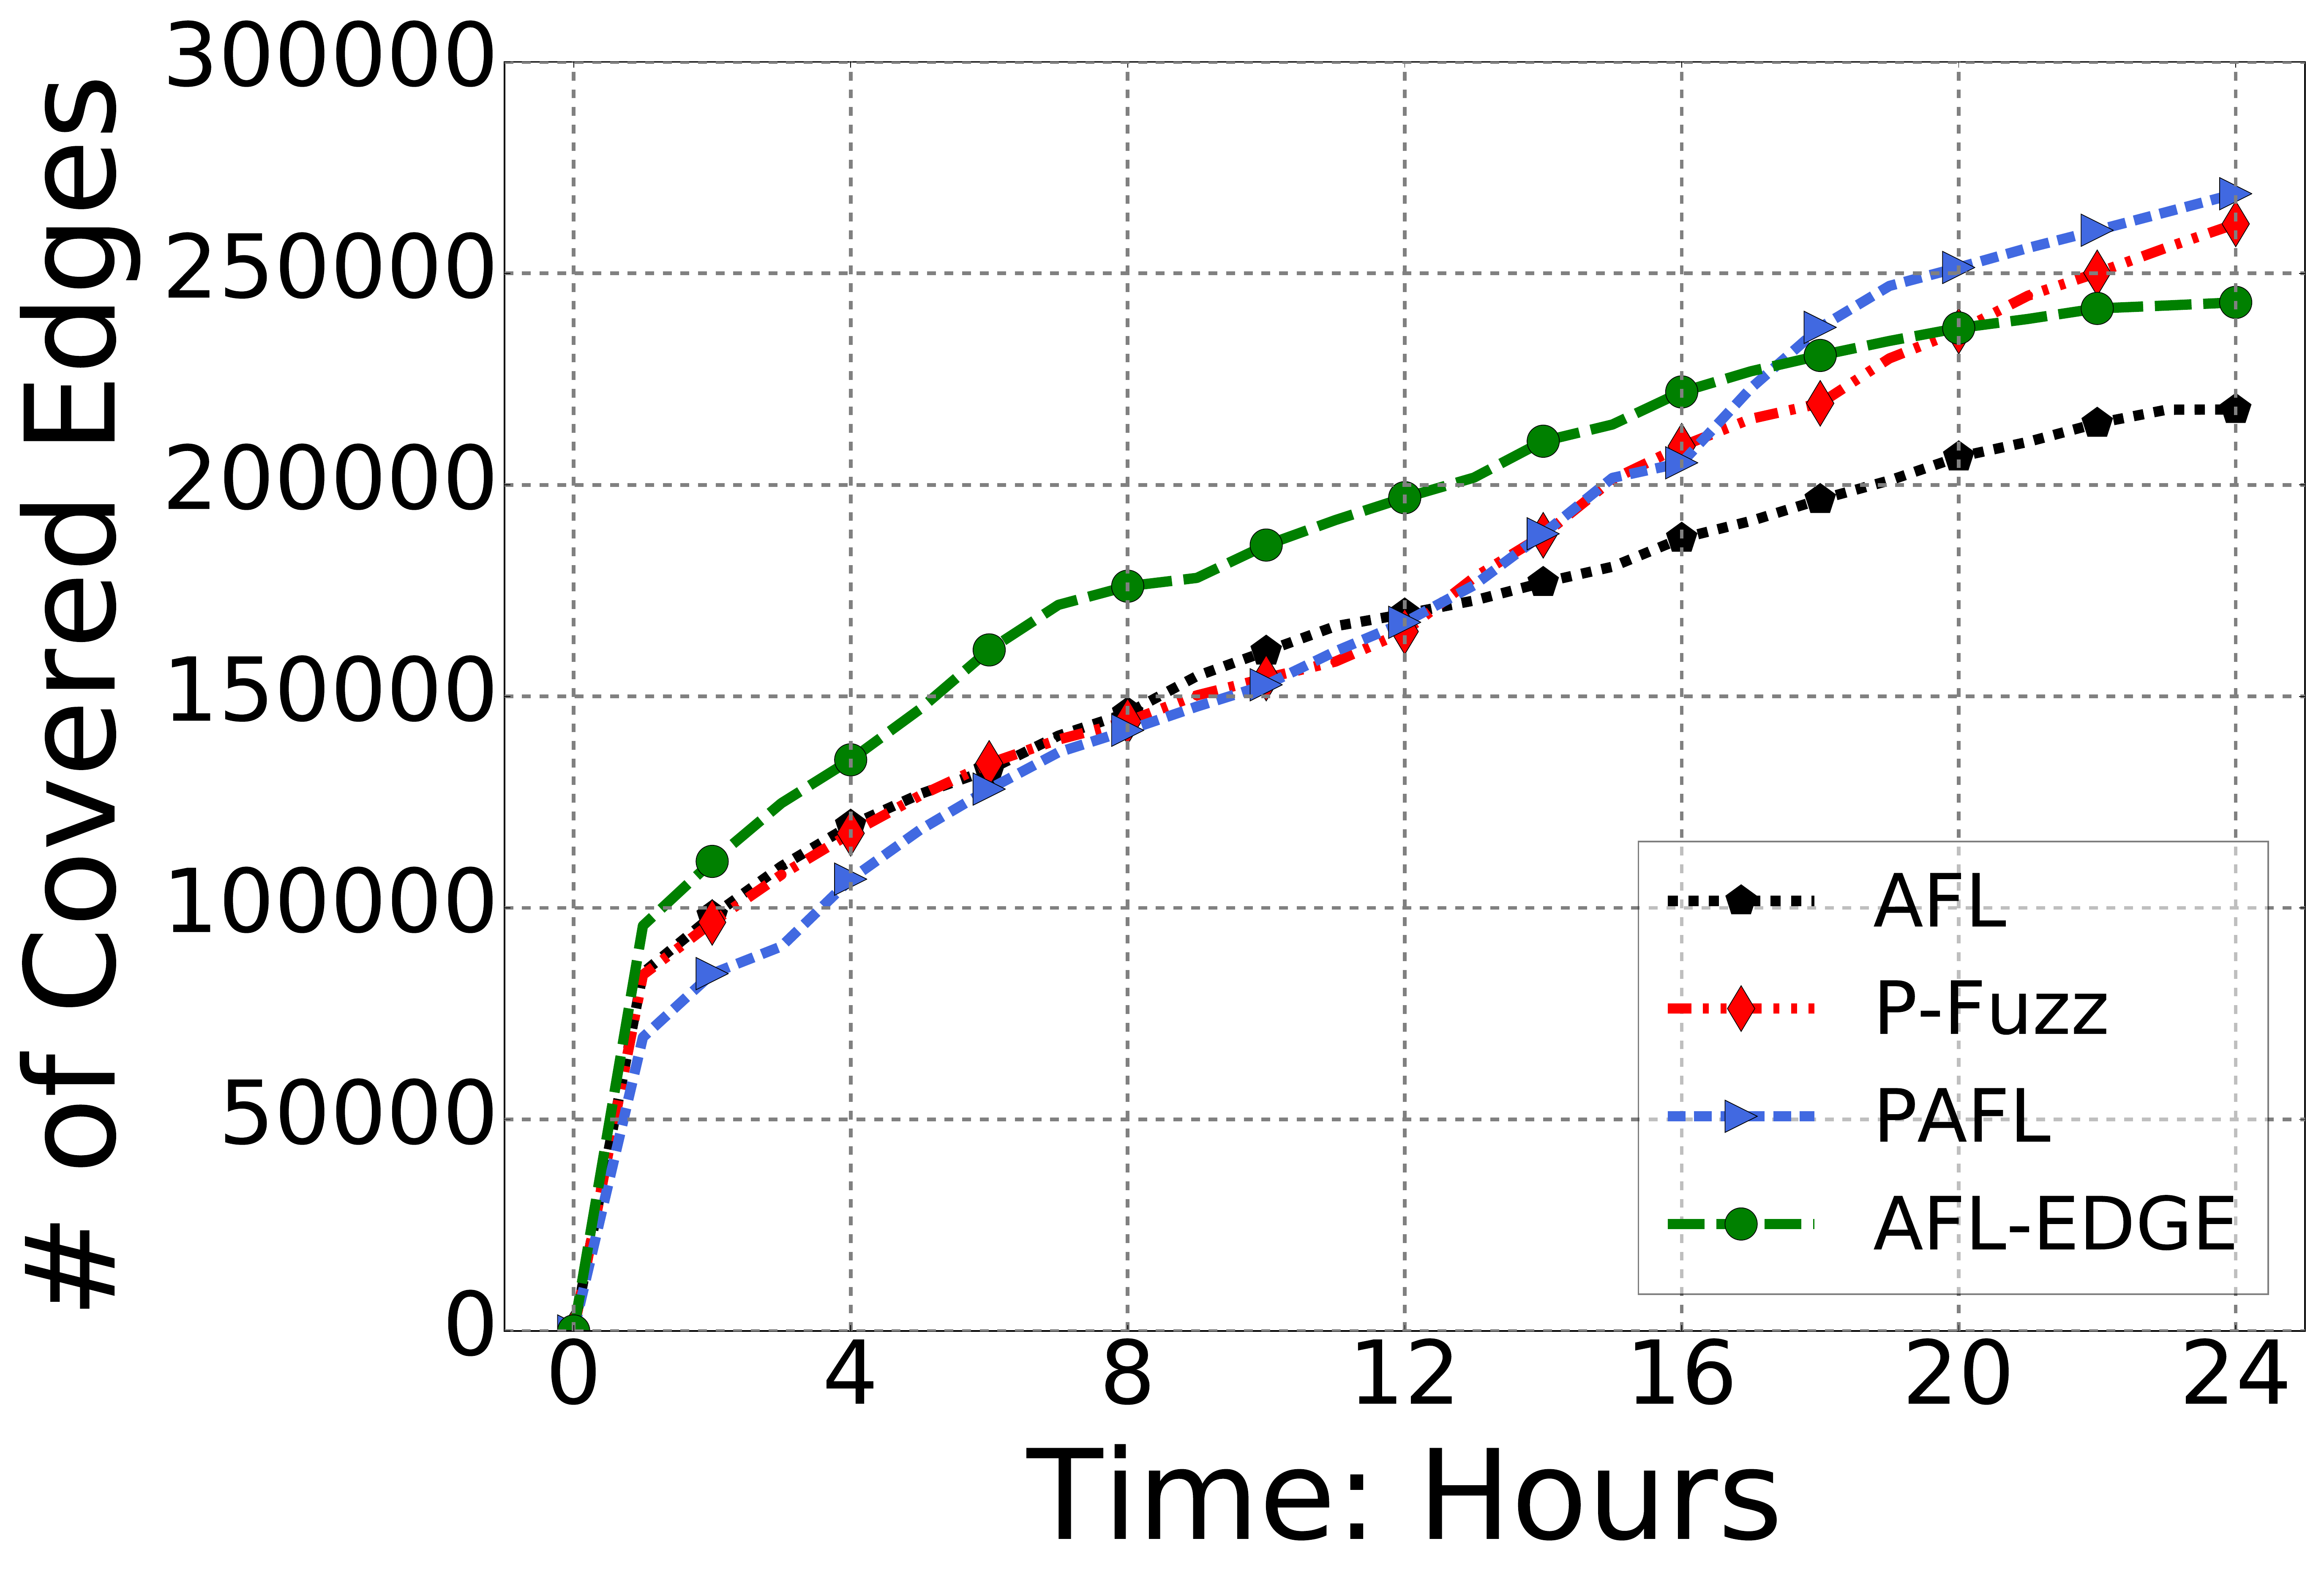} &
         \includegraphics[scale=0.075]{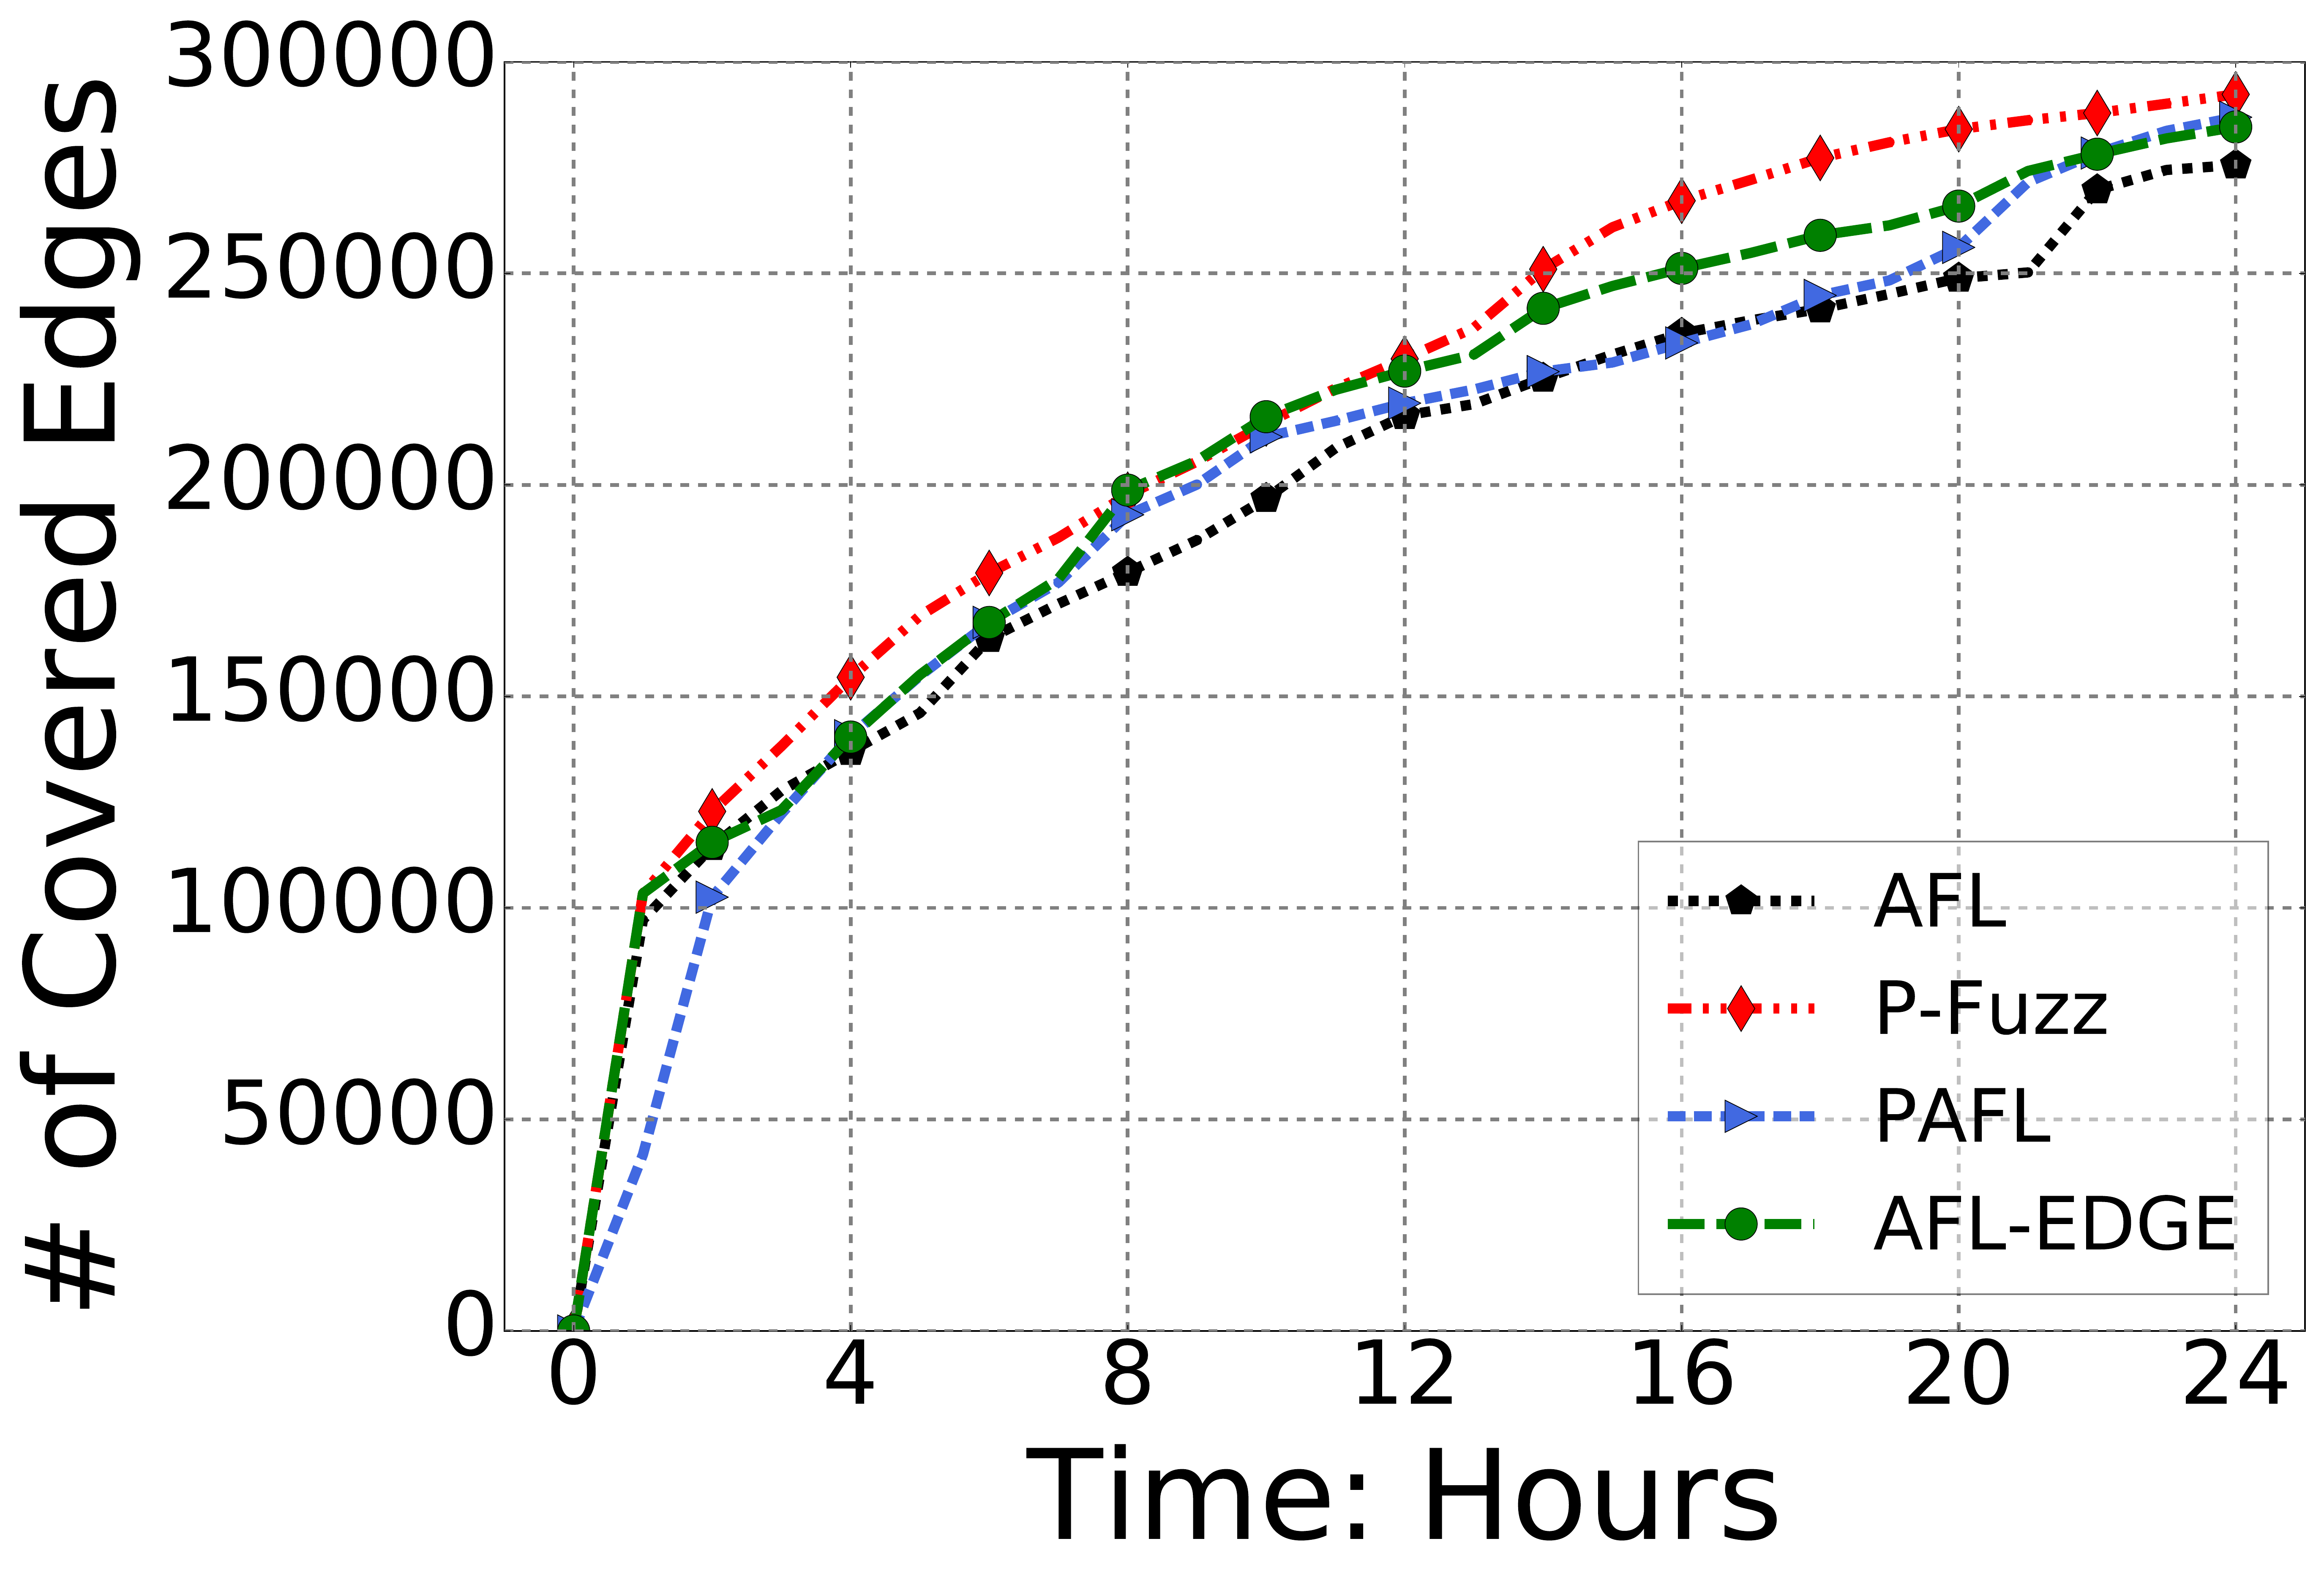} 
         \\
         
         {\scriptsize\textbf{ffmpeg} \scriptsize 2 instances AFL} &
         {\scriptsize\textbf{ffmpeg} \scriptsize 4 instances AFL} &
         {\scriptsize\textbf{ffmpeg} \scriptsize 8 instances AFL}
        %  {\scriptsize\textbf{ffmpeg} \scriptsize 2 instance QSYM} &
        %  {\scriptsize\textbf{ffmpeg} \scriptsize 4 instance QSYM} &
        %  {\scriptsize\textbf{ffmpeg} \scriptsize 8 instance QSYM} 
         
\end{longtable}
\vspace{0.5em}
% \end{adjustwidth}
\captionof{figure}{Results of code coverage with our 9 benchmark programs across 24 hours. }
% The \emph{left} part shows the results of \afl and the \emph{right} part shows the results of \qsym.}

% \captionof{figure}{Results of code coverage with our 9 benchmark programs across 24 hours. The \emph{left} part shows the results of \afl and the \emph{right} part shows the results of \qsym. In the legends, {\tt without\_split} stands for stock \afl/\qsym; {\tt with\_path\_split} means \afl/\qsym with our path-coverage-based task distribution; and {\tt with\_edge\_split} represents \afl/\qsym with our edge-coverage-based task distribution.}
\label{fig:codecov}
% \end{table*}

\clearpage
